# Supplementary material for: Two-loop renormalization of the CPT-even Lorentz-violating Scalar QED
Source: arXiv:2306.08488 source file (2023-06-14)
Supplement: Supplementary file 1 [file LV-SQED-2loops-SupplementalMaterial_pagenumber.pdf]

# Supplemental Material: Two-loop self-energies in CPT-even Lorentz-violating Scalar QED

L. C. T. Brito,[1,*] J. C. C. Felipe,[2,†] A. C. Lehum,[3,‡] and A. Yu. Petrov[4,§]

[1]*Departamento de Física, Instituto de Ciências Naturais, Universidade Federal de Lavras, Caixa Postal 3037, 37200-900, Lavras, Minas Gerais, Brasil*

[2]*Instituto de Engenharia, Ciência e Tecnologia, Universidade Federal dos Vales do Jequitinhonha e Mucuri, Avenida Um, 4050 - 39447-790 - Cidade Universitária - Janaúba, Minas Gerais, Brazil*

[3]*Faculdade de Física, Universidade Federal do Pará, 66075-110, Belém, Pará, Brazil*

[4]*Departamento de Física, Universidade Federal da Paraíba, Caixa Postal 5008, 58051-970 João Pessoa, Paraíba, Brazil*

This supplemental material accompanies the paper titled "Two-loop self-energies in CPT-even Lorentz-violating Scalar QED". In this document, we provide additional information and calculation details that were omitted from the main text, including the two-loop diagrams associated with the photon and scalar self-energies. Throughout this supplementary material, we adopt natural units with $c = \hbar = 1$, and employ the spacetime signature $(+ - - -)$.

## I. CALCULATION OF THE TWO-LOOP PHOTON SELF-ENERGY DIAGRAMS

We initiate our analysis by investigating the two-loop corrections associated with the photon self-energy. The computation of the diagrams is performed utilizing a set of MATHEMATICA packages [1–5]. The two-loop polarization tensor can be decomposed into two distinct components. The first component corresponds to the conventional term, which is proportional to $\left(p^2\eta^{\mu\gamma} - p^\mu p^\gamma\right)$, and is illustrated in Figs. 1 and 2. The second component entails the insertion of a Lorentz-violating (LV) vertex, as depicted in Figs. 3 and 4.

The two-loop polarization tensor $\Pi_{2l}^{\gamma\mu}(p)$ can be expressed as

$$\Pi_{2l}^{\gamma\mu}(p) = \sum_i \int \frac{d^Dk_1}{(2\pi)^D}\frac{d^Dk_2}{(2\pi)^D}\tilde{\Pi}_i^{\gamma\mu}(p), \tag{1}$$

where expressions for $\tilde{\Pi}_i^{\gamma\mu}(p)$ for each contribution as depicted in Fig. 1 are given by

*Electronic address: lcbrito@dfi.ufla.br
†Electronic address: jean.cfelipe@ufvjm.edu.br
‡Electronic address: lehum@ufpa.br
§Electronic address: petrov@fisica.ufpb.br

$$\tilde{\Pi}_1^{\gamma\mu}(p) = \frac{i\, e^2\, \lambda\, (2\, k_1{}^{\gamma} - p^{\gamma})\, (2\, k_1{}^{\mu} - p^{\mu})}{k_1{}^2 . k_2{}^2 . (\, k_1 - p\,)^{2^2}}$$

$$\tilde{\Pi}_2^{\gamma\mu}(p) = \frac{i\, e^2\, \lambda\, (2\, k_1{}^{\gamma} - p^{\gamma})\, (2\, k_1{}^{\mu} - p^{\mu})}{k_1{}^2 . k_2{}^2 . (\, k_1 - p\,)^{2^2}}$$

$$\tilde{\Pi}_3^{\gamma\mu}(p) = \frac{i\, D\, e^4\, (2\, k_1{}^{\gamma} - p^{\gamma})\, (2\, k_1{}^{\mu} - p^{\mu})}{k_1{}^2 . k_2{}^2 . (\, k_1 - p\,)^{2^2}}$$

$$\tilde{\Pi}_4^{\gamma\mu}(p) = \frac{i\, D\, e^4\, (2\, k_1{}^{\gamma} - p^{\gamma})\, (2\, k_1{}^{\mu} - p^{\mu})}{k_1{}^2 . k_2{}^2 . (\, k_1 - p\,)^{2^2}}$$

$$\tilde{\Pi}_5^{\gamma\mu}(p) = \frac{2\, i\, e^4\, (p^{\mu} + 2\, k_1{}^{\mu})\, (k_1{}^{\gamma} - k_2{}^{\gamma})}{k_2{}^2 . k_1{}^2 . (\, k_1 + p\,)^2 . (\, k_1 + k_2\,)^2}$$

$$\tilde{\Pi}_6^{\gamma\mu}(p) = \frac{2\, i\, e^4\, (p^{\mu} + 2\, k_1{}^{\mu})\, (k_1{}^{\gamma} - k_2{}^{\gamma})}{k_2{}^2 . k_1{}^2 . (\, k_1 + p\,)^2 . (\, k_1 + k_2\,)^2}$$

$$\tilde{\Pi}_7^{\gamma\mu}(p) = \frac{2\, i\, e^4\, (2\, k_1{}^{\gamma} - p^{\gamma})\, (k_1{}^{\mu} - k_2{}^{\mu})}{k_2{}^2 . k_1{}^2 . (\, k_1 - p\,)^2 . (\, k_1 + k_2\,)^2}$$

$$\tilde{\Pi}_8^{\gamma\mu}(p) = \frac{2\, i\, e^4\, (2\, k_1{}^{\gamma} - p^{\gamma})\, (k_1{}^{\mu} - k_2{}^{\mu})}{k_2{}^2 . k_1{}^2 . (\, k_1 - p\,)^2 . (\, k_1 + k_2\,)^2}$$

$$\tilde{\Pi}_9^{\gamma\mu}(p) = \frac{i\, e^4\, (p^{\mu} + 2\, k_1{}^{\mu})\, (2\, k_2{}^{\gamma} - p^{\gamma})\left(2\, (k_1 \cdot p) - 2\, (k_2 \cdot p) - 2\, (k_1 \cdot k_2) + k_1{}^2 + k_2{}^2\right)}{k_2{}^2 . k_1{}^2 . (\, k_1 + p\,)^2 . (\, k_2 - p\,)^2 . (\, k_1 + k_2\,)^2}$$

$$\tilde{\Pi}_{10}^{\gamma\mu}(p) = -\frac{i\, e^4\, (2\, k_1{}^{\gamma} - p^{\gamma})\, (2\, k_1{}^{\mu} - p^{\mu})\left(-2\, (k_1 \cdot p) - 2\, (k_2 \cdot p) + p^2 + 2\, (k_1 \cdot k_2) + k_1{}^2 + k_2{}^2\right)}{k_2{}^2 . k_1{}^2 . (\, k_1 - p\,)^{2^2} . (\, -k_1 + k_2 + p\,)^2}$$

$$\tilde{\Pi}_{11}^{\gamma\mu}(p) = -\frac{i\, e^4\, (2\, k_1{}^{\gamma} - p^{\gamma})\, (2\, k_1{}^{\mu} - p^{\mu})\left(-2\, (k_1 \cdot p) - 2\, (k_2 \cdot p) + p^2 + 2\, (k_1 \cdot k_2) + k_1{}^2 + k_2{}^2\right)}{k_2{}^2 . k_1{}^2 . (\, k_1 - p\,)^{2^2} . (\, -k_1 + k_2 + p\,)^2}$$

$$\tilde{\Pi}_{12}^{\gamma\mu}(p) = -\frac{2\, i\, e^2\, \lambda\, g^{\mu\,\gamma}}{\left(k_1{}^2\right)^2 . k_2{}^2}$$

$$\tilde{\Pi}_{13}^{\gamma\mu}(p) = -\frac{2\, i\, D\, e^4\, g^{\mu\,\gamma}}{\left(k_1{}^2\right)^2 . k_2{}^2}$$

$$\tilde{\Pi}_{14}^{\gamma\mu}(p) = \frac{i\, e^2\, \lambda\, (2\, k_1{}^{\mu} - p^{\mu})\, (p^{\gamma} + 2\, k_2{}^{\gamma})}{k_2{}^2 . k_1{}^2 . (\, k_2 + p\,)^2 . (\, k_1 - p\,)^2}$$

$$\tilde{\Pi}_{15}^{\gamma\mu}(p) = \frac{2\, i\, e^4\, g^{\mu\,\gamma}\left(4\, (k_1 \cdot k_2) + 4\, k_1{}^2 + k_2{}^2\right)}{k_2{}^2 . k_1{}^2 . (\, k_1 + k_2\,)^{2^2}}$$

$$\tilde{\Pi}_{16}^{\gamma\mu}(p) = -\frac{4\, i\, e^4\, g^{\mu\,\gamma}}{k_2{}^2 . k_1{}^2 . (\, k_1 + k_2 + p\,)^2}$$

Now, in order to simplify the two-loop tensor integral, we perform a decomposition that involves transforming the Lorentz indices away from the loop momenta $k_1$ and $k_2$. This allows us to express the integral as follows

$$\tilde{\Pi}_1^{\gamma\mu}(p) = \frac{i\, e^2 \lambda\, p^\gamma p^\mu}{k_2^2.k_1^2.(k_1 - p)^{22}}$$

$$\tilde{\Pi}_2^{\gamma\mu}(p) = \frac{i\, e^2 \lambda\, p^\gamma p^\mu}{k_2^2.k_1^2.(k_1 - p)^{22}}$$

$$\tilde{\Pi}_3^{\gamma\mu}(p) = \frac{i\, D\, e^4\, p^\gamma p^\mu}{k_2^2.k_1^2.(k_1 - p)^{22}}$$

$$\tilde{\Pi}_4^{\gamma\mu}(p) = \frac{i\, D\, e^4\, p^\gamma p^\mu}{k_2^2.k_1^2.(k_1 - p)^{22}}$$

$$\tilde{\Pi}_5^{\gamma\mu}(p) = \frac{1}{(D-1)\, p^4}$$

$$i\, e^4 \left( \frac{2\,(k_1 \cdot p)\left(D\, p^\gamma p^\mu - p^2 g^{\mu\gamma}\right)}{k_2^2.(k_1 - k_2)^2.(k_1 - p)^2} + \frac{p^\gamma p^\mu \left(2\, D\,(k_1 \cdot p) - 5\, p^2\right) + p^2 g^{\mu\gamma}\left(5\, p^2 - 2\,(k_1 \cdot p)\right)}{k_1^2.(k_1 - k_2)^2.(k_2 - p)^2} - p^2 \left(p^2 g^{\mu\gamma} - p^\gamma p^\mu\right) \left( -\frac{2}{k_1^2.(k_1 - k_2)^2.(k_1 - p)^2} + \frac{p^2}{k_1^2.k_2^2.(k_1 - k_2)^2.(k_1 - p)^2} + \frac{2\,(k_1 \cdot p)}{k_1^2.k_2^2.(k_1 - k_2)^2.(k_2 - p)^2} \right)\right)$$

$$\tilde{\Pi}_6^{\gamma\mu}(p) = \frac{1}{(D-1)\, p^4} i\, e^4 \left( \frac{2\,(k_1 \cdot p)\left(D\, p^\gamma p^\mu - p^2 g^{\mu\gamma}\right)}{k_2^2.(k_1 - k_2)^2.(k_1 - p)^2} + \frac{p^\gamma p^\mu \left(2\, D\,(k_1 \cdot p) - 5\, p^2\right) + p^2 g^{\mu\gamma}\left(5\, p^2 - 2\,(k_1 \cdot p)\right)}{k_1^2.(k_1 - k_2)^2.(k_2 - p)^2} - p^2 \left(p^2 g^{\mu\gamma} - p^\gamma p^\mu\right) \left( -\frac{2}{k_1^2.(k_1 - k_2)^2.(k_1 - p)^2} + \frac{p^2}{k_1^2.k_2^2.(k_1 - k_2)^2.(k_1 - p)^2} + \frac{2\,(k_1 \cdot p)}{k_1^2.k_2^2.(k_1 - k_2)^2.(k_2 - p)^2} \right)\right)$$

$$\tilde{\Pi}_7^{\gamma\mu}(p) = \frac{1}{(D-1)\, p^4} i\, e^4 \left( \frac{2\,(k_1 \cdot p)\left(D\, p^\gamma p^\mu - p^2 g^{\mu\gamma}\right)}{k_2^2.(k_1 - k_2)^2.(k_1 - p)^2} + \frac{p^\gamma p^\mu \left(2\, D\,(k_1 \cdot p) - 5\, p^2\right) + p^2 g^{\mu\gamma}\left(5\, p^2 - 2\,(k_1 \cdot p)\right)}{k_1^2.(k_1 - k_2)^2.(k_2 - p)^2} - p^2 \left(p^2 g^{\mu\gamma} - p^\gamma p^\mu\right) \left( -\frac{2}{k_1^2.(k_1 - k_2)^2.(k_1 - p)^2} + \frac{p^2}{k_1^2.k_2^2.(k_1 - k_2)^2.(k_1 - p)^2} + \frac{2\,(k_1 \cdot p)}{k_1^2.k_2^2.(k_1 - k_2)^2.(k_2 - p)^2} \right)\right)$$

$$\tilde{\Pi}_8^{\gamma\mu}(p) = \frac{1}{(D-1)\, p^4} i\, e^4 \left( \frac{2\,(k_1 \cdot p)\left(D\, p^\gamma p^\mu - p^2 g^{\mu\gamma}\right)}{k_2^2.(k_1 - k_2)^2.(k_1 - p)^2} + \frac{p^\gamma p^\mu \left(2\, D\,(k_1 \cdot p) - 5\, p^2\right) + p^2 g^{\mu\gamma}\left(5\, p^2 - 2\,(k_1 \cdot p)\right)}{k_1^2.(k_1 - k_2)^2.(k_2 - p)^2} - p^2 \left(p^2 g^{\mu\gamma} - p^\gamma p^\mu\right) \left( -\frac{2}{k_1^2.(k_1 - k_2)^2.(k_1 - p)^2} + \frac{p^2}{k_1^2.k_2^2.(k_1 - k_2)^2.(k_1 - p)^2} + \frac{2\,(k_1 \cdot p)}{k_1^2.k_2^2.(k_1 - k_2)^2.(k_2 - p)^2} \right)\right)$$

$$\tilde{\Pi}_9^{\gamma\mu}(p) = -\frac{1}{(D-1)\, p^4} i\, e^4 \left( \frac{4\left(p^\gamma p^\mu \left(2\, D\,(k_1 \cdot p) - p^2\right) + p^2 g^{\mu\gamma}\left(p^2 - 2\,(k_1 \cdot p)\right)\right)}{k_1^2.(k_1 - k_2)^2.(k_2 - p)^2} + p^2 \left(p^2 g^{\mu\gamma} - p^\gamma p^\mu\right) \left( \frac{2\, p^4}{k_1^2.k_2^2.(k_1 - k_2)^2.(k_1 - p)^2.(k_2 - p)^2} - \frac{8\, p^2}{k_1^2.k_2^2.(k_1 - k_2)^2.(k_1 - p)^2} + \frac{8}{k_1^2.(k_1 - k_2)^2.(k_1 - p)^2} - \frac{8\,(k_1 \cdot p)}{k_1^2.k_2^2.(k_1 - k_2)^2.(k_2 - p)^2} + \frac{5\, p^2 - 4\,(k_1 \cdot k_2)}{k_1^2.k_2^2.(k_1 - p)^2.(k_2 - p)^2} \right)\right)$$

$$\tilde{\Pi}_{10}^{\gamma\mu}(p) = -\frac{1}{(D-1)\,p^4} i\, e^4 \left( \frac{2\,(k_1\cdot p)\left(D\,p^\gamma\,p^\mu - p^2\,g^{\mu\gamma}\right)}{k_2{}^2.(k_1-k_2)^2.(k_1-p)^2} + \frac{p^\gamma\,p^\mu\left(2\,D\,(k_1\cdot k_2) - (D+2)\,p^2\right) + p^2\,g^{\mu\gamma}\left(3\,p^2 - 2\,(k_1\cdot k_2)\right)}{k_1{}^2.(k_1-k_2)^2.(k_2-p)^2} + \right.$$

$$p^2 \left( p^2 \left( \frac{p^\gamma\,p^\mu\left(-(D-1)\,p^2 - 2\,(D-2)\,(k_1\cdot k_2)\right) - 2\,p^2\,g^{\mu\gamma}\,(k_1\cdot k_2)}{\left(k_1{}^2\right)^2.k_2{}^2.(k_1-k_2)^2.(k_1-p)^2} + \right.\right.$$

$$\left.\left.\left. \frac{(D-1)\,p^\gamma\,p^\mu\left(-2\,(k_2\cdot p) + p^2 + 2\,(k_1\cdot k_2)\right)}{k_1{}^2.k_2{}^2.(k_1-p)^{2\,2}.(k_1-k_2-p)^2} \right) + \frac{\left(p^2\,g^{\mu\gamma} - p^\gamma\,p^\mu\right)\left(4\,(k_1\cdot k_2) - p^2\right)}{k_1{}^2.k_2{}^2.(k_1-k_2)^2.(k_1-p)^2} \right)\right)$$

$$\tilde{\Pi}_{11}^{\gamma\mu}(p) = -\frac{1}{(D-1)\,p^4} i\, e^4 \left( \frac{2\,(k_1\cdot p)\left(D\,p^\gamma\,p^\mu - p^2\,g^{\mu\gamma}\right)}{k_2{}^2.(k_1-k_2)^2.(k_1-p)^2} + \frac{p^\gamma\,p^\mu\left(2\,D\,(k_1\cdot k_2) - (D+2)\,p^2\right) + p^2\,g^{\mu\gamma}\left(3\,p^2 - 2\,(k_1\cdot k_2)\right)}{k_1{}^2.(k_1-k_2)^2.(k_2-p)^2} + \right.$$

$$p^2 \left( p^2 \left( \frac{p^\gamma\,p^\mu\left(-(D-1)\,p^2 - 2\,(D-2)\,(k_1\cdot k_2)\right) - 2\,p^2\,g^{\mu\gamma}\,(k_1\cdot k_2)}{\left(k_1{}^2\right)^2.k_2{}^2.(k_1-k_2)^2.(k_1-p)^2} + \right.\right.$$

$$\left.\left.\left. \frac{(D-1)\,p^\gamma\,p^\mu\left(-2\,(k_2\cdot p) + p^2 + 2\,(k_1\cdot k_2)\right)}{k_1{}^2.k_2{}^2.(k_1-p)^{2\,2}.(k_1-k_2-p)^2} \right) + \frac{\left(p^2\,g^{\mu\gamma} - p^\gamma\,p^\mu\right)\left(4\,(k_1\cdot k_2) - p^2\right)}{k_1{}^2.k_2{}^2.(k_1-k_2)^2.(k_1-p)^2} \right)\right)$$

$$\tilde{\Pi}_{12}^{\gamma\mu}(p) = -\frac{2\,i\,e^2\,\lambda\,g^{\mu\gamma}}{k_2{}^2.\left(k_1{}^2\right)^2}$$

$$\tilde{\Pi}_{13}^{\gamma\mu}(p) = -\frac{2\,i\,D\,e^4\,g^{\mu\gamma}}{k_2{}^2.\left(k_1{}^2\right)^2}$$

$$\tilde{\Pi}_{14}^{\gamma\mu}(p) = i\,e^2\,\lambda \left( \frac{p^\gamma\,p^\mu\left(4\,(k_1\cdot k_2) - D\,p^2\right) + p^2\,g^{\mu\gamma}\left(p^2 - 4\,(k_1\cdot k_2)\right)}{(D-1)\,p^2\,k_1{}^2.k_2{}^2.(k_1-p)^2.(k_2-p)^2} + \right.$$

$$\left. p^\gamma\,p^\mu \left( \frac{2}{k_1{}^2.k_2{}^2.(k_1-p)^2.(k_2-p)^2} - \frac{1}{k_1{}^2.k_2{}^2.(k_1-p)^2.(k_2+p)^2} \right)\right)$$

$$\tilde{\Pi}_{15}^{\gamma\mu}(p) = 0$$

$$\tilde{\Pi}_{16}^{\gamma\mu}(p) = -\frac{4\,i\,e^4\,g^{\mu\gamma}}{k_1{}^2.k_2{}^2.(k_1+k_2+p)^2}$$

The subsequent step involves applying the Tarasov algorithm [6] to express the scalar integrals in terms of a set of fundamental ones. This procedure is facilitated by utilizing the TARCER package [5] within the MATHEMATICA software. The basic integrals utilized in this algorithm are defined in the Appendix. Thus, after performing the necessary calculations, we obtain the following results:

$$(4\,\pi)^D\,\Pi_1^{\gamma\mu}(p) = 0$$
$$(4\,\pi)^D\,\Pi_2^{\gamma\mu}(p) = 0$$
$$(4\,\pi)^D\,\Pi_3^{\gamma\mu}(p) = 0$$
$$(4\,\pi)^D\,\Pi_4^{\gamma\mu}(p) = 0$$
$$(4\,\pi)^D\,\Pi_5^{\gamma\mu}(p) = \frac{2\,i\,\mathrm{e}^4\left((D-3)\,p^\gamma\,p^\mu - p^2\,g^{\mu\,\gamma}\right)\mathbf{J}^{(D)}_{\{1,0\}\,\{1,0\}\,\{1,0\}}}{(D-4)\,p^2}$$
$$(4\,\pi)^D\,\Pi_6^{\gamma\mu}(p) = \frac{2\,i\,\mathrm{e}^4\left((D-3)\,p^\gamma\,p^\mu - p^2\,g^{\mu\,\gamma}\right)\mathbf{J}^{(D)}_{\{1,0\}\,\{1,0\}\,\{1,0\}}}{(D-4)\,p^2}$$
$$(4\,\pi)^D\,\Pi_7^{\gamma\mu}(p) = \frac{2\,i\,\mathrm{e}^4\left((D-3)\,p^\gamma\,p^\mu - p^2\,g^{\mu\,\gamma}\right)\mathbf{J}^{(D)}_{\{1,0\}\,\{1,0\}\,\{1,0\}}}{(D-4)\,p^2}$$
$$(4\,\pi)^D\,\Pi_8^{\gamma\mu}(p) = \frac{2\,i\,\mathrm{e}^4\left((D-3)\,p^\gamma\,p^\mu - p^2\,g^{\mu\,\gamma}\right)\mathbf{J}^{(D)}_{\{1,0\}\,\{1,0\}\,\{1,0\}}}{(D-4)\,p^2}$$
$$(4\,\pi)^D\,\Pi_9^{\gamma\mu}(p) =$$
$$-\frac{1}{3\,(D-4)^2\,(D-1)\,p^2} 4\,i\,\mathrm{e}^4\left(p^2\,g^{\mu\,\gamma}\left(4\left(D^2-2\,D-2\right)\mathbf{J}^{(D)}_{\{1,0\}\,\{1,0\}\,\{1,0\}} - 3\,(D-4)\,p^2\left(\mathbf{B}^{(D)}_{\{1,0\}\,\{1,0\}}\right)^2\right) + \right.$$
$$\left. p^\gamma\,p^\mu\left(3\,(D-4)\,p^2\left(\mathbf{B}^{(D)}_{\{1,0\}\,\{1,0\}}\right)^2 + 2\left(D^3-11\,D^2+28\,D-12\right)\mathbf{J}^{(D)}_{\{1,0\}\,\{1,0\}\,\{1,0\}}\right)\right)$$
$$(4\,\pi)^D\,\Pi_{10}^{\gamma\mu}(p) = -\frac{2\,i\,\mathrm{e}^4\left(D\,p^\gamma\,p^\mu - 4\,p^2\,g^{\mu\,\gamma}\right)\mathbf{J}^{(D)}_{\{1,0\}\,\{1,0\}\,\{1,0\}}}{3\,(D-4)\,p^2}$$
$$(4\,\pi)^D\,\Pi_{11}^{\gamma\mu}(p) = -\frac{2\,i\,\mathrm{e}^4\left(D\,p^\gamma\,p^\mu - 4\,p^2\,g^{\mu\,\gamma}\right)\mathbf{J}^{(D)}_{\{1,0\}\,\{1,0\}\,\{1,0\}}}{3\,(D-4)\,p^2}$$
$$(4\,\pi)^D\,\Pi_{12}^{\gamma\mu}(p) = 0$$
$$(4\,\pi)^D\,\Pi_{13}^{\gamma\mu}(p) = 0$$
$$(4\,\pi)^D\,\Pi_{14}^{\gamma\mu}(p) = 0$$
$$(4\,\pi)^D\,\Pi_{15}^{\gamma\mu}(p) = 0$$
$$(4\,\pi)^D\,\Pi_{16}^{\gamma\mu}(p) = -4\,i\,\mathrm{e}^4\,g^{\mu\,\gamma}\,\mathbf{J}^{(D)}_{\{1,0\}\,\{1,0\}\,\{1,0\}}$$

where the vanishing amplitudes are proportional to the $\mathbf{A}^{(D)}_{1,0}$ integral, except for $\Pi^{\gamma\mu}_{14}(p)$, which is vanishing due to cancellations among the $\mathbf{J}$ integrals. The integrals used in these expressions are defined in the Appendix.

By expanding around $D = 4 - 2\epsilon$ and considering all relevant contributions, we obtain

$$-i\Pi^{\gamma\mu}_{2l}(p) = -\frac{e^4\left(p^2\eta^{\gamma\mu} - p^\gamma p^\mu\right)}{128\pi^4\epsilon} + \text{finite}. \tag{2}$$

The diagrams depicted in Figs. 3 and 4 represent the contribution of LV effects to the two-loop polarization tensor. In our analysis, we will primarily focus on computing the expressions associated with the two-loop diagrams. Taking into account the form provided in Eq. (1), the functions $\tilde{\Pi}^{\gamma\mu}_i(p)$ can be expressed as follows

$$\tilde{\Pi}^{\gamma\mu}_{1.\,\mathrm{LV}}(p) = -\frac{2\, i\, \mathrm{e}^4\, Q_1\, (p^\mu + 2\, k_1{}^\mu)\, (k_1{}^\gamma - k_2{}^\gamma)\, (\, k_2 \cdot u\,)^2}{\left(k_2{}^2\right)^2 . k_1{}^2 .(\, k_1 + p\,)^2 .(\, k_1 + k_2\,)^2}$$

$$\tilde{\Pi}^{\gamma\mu}_{2\,\mathrm{LV}}(p) = -\frac{2\, i\, \mathrm{e}^4\, Q_1\, (p^\mu + 2\, k_1{}^\mu)\, (k_1{}^\gamma - k_2{}^\gamma)\, (\, k_2 \cdot u\,)^2}{\left(k_2{}^2\right)^2 . k_1{}^2 .(\, k_1 + p\,)^2 .(\, k_1 + k_2\,)^2}$$

$$\tilde{\Pi}^{\gamma\mu}_{3\,\mathrm{LV}}(p) = \frac{2\, i\, \mathrm{e}^4\, Q_2\, (p^\mu + 2\, k_1{}^\mu)\left((k_2 \cdot u)\, (k_1{}^\gamma\, (k_2 \cdot u) - k_2{}^\gamma\, (k_1 \cdot u)) + u^\gamma \left(k_2{}^2\, (k_1 \cdot u) - (k_1 \cdot k_2)\, (k_2 \cdot u)\right)\right)}{\left(k_2{}^2\right)^2 . k_1{}^2 .(\, k_1 + p\,)^2 .(\, k_1 + k_2\,)^2}$$

$$\tilde{\Pi}^{\gamma\mu}_{4\,\mathrm{LV}}(p) = \frac{2\, i\, \mathrm{e}^4\, Q_2\, (p^\mu + 2\, k_1{}^\mu)\left((k_2 \cdot u)\, (k_1{}^\gamma\, (k_2 \cdot u) - k_2{}^\gamma\, (k_1 \cdot u)) + u^\gamma \left(k_2{}^2\, (k_1 \cdot u) - (k_1 \cdot k_2)\, (k_2 \cdot u)\right)\right)}{\left(k_2{}^2\right)^2 . k_1{}^2 .(\, k_1 + p\,)^2 .(\, k_1 + k_2\,)^2}$$

$$\tilde{\Pi}^{\gamma\mu}_{5\,\mathrm{LV}}(p) = \frac{i\, \mathrm{e}^4\, Q_1\, (p^\mu + 2\, k_1{}^\mu)\, (2\, k_2{}^\gamma - p^\gamma)\, (k_1 \cdot u - k_2 \cdot u)\, (2\, (p \cdot u) + k_1 \cdot u - k_2 \cdot u)}{k_2{}^2 . k_1{}^2 .(\, k_1 + p\,)^2 .(\, k_2 - p\,)^2 .(\, k_1 + k_2\,)^2}$$

$$\tilde{\Pi}^{\gamma\mu}_{6\,\mathrm{LV}}(p) = \frac{i\, \mathrm{e}^4\, Q_1\, (p^\mu + 2\, k_1{}^\mu)\, (2\, k_2{}^\gamma - p^\gamma)\, (k_1 \cdot u - k_2 \cdot u)\, (2\, (p \cdot u) + k_1 \cdot u - k_2 \cdot u)}{k_2{}^2 . k_1{}^2 .(\, k_1 + p\,)^2 .(\, k_2 - p\,)^2 .(\, k_1 + k_2\,)^2}$$

$$\tilde{\Pi}^{\gamma\mu}_{7\,\mathrm{LV}}(p) = \frac{2\, i\, \mathrm{e}^4\, Q_1\, (2\, k_2{}^\gamma - p^\gamma)\, (k_1{}^\mu - k_2{}^\mu)\, (\, k_1 \cdot u\,)^2}{k_1{}^2 . k_2{}^2 . k_1{}^2 .(\, k_2 - p\,)^2 .(\, k_1 + k_2\,)^2}$$

$$\tilde{\Pi}^{\gamma\mu}_{8\,\mathrm{LV}}(p) = \frac{2\, i\, \mathrm{e}^4\, Q_1\, (2\, k_2{}^\gamma - p^\gamma)\, (k_1{}^\mu - k_2{}^\mu)\, (\, k_1 \cdot u\,)^2}{k_1{}^2 . k_2{}^2 . k_1{}^2 .(\, k_2 - p\,)^2 .(\, k_1 + k_2\,)^2}$$

$$\tilde{\Pi}^{\gamma\mu}_{9\,\mathrm{LV}}(p) = -\frac{2\, i\, \mathrm{e}^4\, Q_2\, (2\, k_2{}^\gamma - p^\gamma)\left((k_1 \cdot u)\, (k_1{}^\mu\, (k_2 \cdot u) - k_2{}^\mu\, (k_1 \cdot u)) + u^\mu \left((k_1 \cdot k_2)\, (k_1 \cdot u) - k_1{}^2\, (k_2 \cdot u)\right)\right)}{k_1{}^2 . k_2{}^2 . k_1{}^2 .(\, k_2 - p\,)^2 .(\, k_1 + k_2\,)^2}$$

$$\tilde{\Pi}^{\gamma\mu}_{10\,\mathrm{LV}}(p) = -\frac{2\, i\, \mathrm{e}^4\, Q_2\, (2\, k_2{}^\gamma - p^\gamma)\left((k_1 \cdot u)\, (k_1{}^\mu\, (k_2 \cdot u) - k_2{}^\mu\, (k_1 \cdot u)) + u^\mu \left((k_1 \cdot k_2)\, (k_1 \cdot u) - k_1{}^2\, (k_2 \cdot u)\right)\right)}{k_1{}^2 . k_2{}^2 . k_1{}^2 .(\, k_2 - p\,)^2 .(\, k_1 + k_2\,)^2}$$

$$\tilde{\Pi}^{\gamma\mu}_{11\,\mathrm{LV}}(p) = -\frac{i\, \mathrm{e}^4\, Q_1\, (p^\mu + 2\, k_1{}^\mu)\, (2\, k_2{}^\gamma - p^\gamma)\left(2\, (k_1 \cdot p) - 2\, (k_2 \cdot p) - 2\, (k_1 \cdot k_2) + k_1{}^2 + k_2{}^2\right)(k_2 \cdot u - p \cdot u)^2}{k_2{}^2 . k_1{}^2 .(\, k_1 + p\,)^2 .(\, k_2 - p\,)^{2\,2} .(\, k_1 + k_2\,)^2}$$

$$\tilde{\Pi}^{\gamma\mu}_{12\,\mathrm{LV}}(p) = -\frac{i\, \mathrm{e}^4\, Q_1\, (p^\mu + 2\, k_1{}^\mu)\, (2\, k_2{}^\gamma - p^\gamma)\left(2\, (k_1 \cdot p) - 2\, (k_2 \cdot p) - 2\, (k_1 \cdot k_2) + k_1{}^2 + k_2{}^2\right)(k_2 \cdot u - p \cdot u)^2}{k_2{}^2 . k_1{}^2 .(\, k_1 + p\,)^2 .(\, k_2 - p\,)^{2\,2} .(\, k_1 + k_2\,)^2}$$

$$\tilde{\Pi}^{\gamma\mu}_{13\,\mathrm{LV}}(p) = -\frac{i\, \mathrm{e}^4\, Q_1\, (2\, k_1{}^\mu - p^\mu)\, (2\, k_2{}^\gamma - p^\gamma)\left(-p^2 - 2\, (k_1 \cdot k_2) + k_1{}^2 + k_2{}^2\right)(\, k_1 \cdot u\,)^2}{k_1{}^2 . k_2{}^2 . k_1{}^2 .(\, k_1 - p\,)^2 .(\, k_2 - p\,)^2 .(\, k_1 + k_2 - p\,)^2}$$

$$\tilde{\Pi}^{\gamma\mu}_{14\,\mathrm{LV}}(p) = -\frac{i\, \mathrm{e}^4\, Q_1\, (2\, k_1{}^\mu - p^\mu)\, (2\, k_2{}^\gamma - p^\gamma)\left(-p^2 - 2\, (k_1 \cdot k_2) + k_1{}^2 + k_2{}^2\right)(\, k_1 \cdot u\,)^2}{k_1{}^2 . k_2{}^2 . k_1{}^2 .(\, k_1 - p\,)^2 .(\, k_2 - p\,)^2 .(\, k_1 + k_2 - p\,)^2}$$

$$\tilde{\Pi}^{\gamma\mu}_{15\,\mathrm{LV}}(p) = \frac{i\, \mathrm{e}^4\, Q_1\, (2\, k_1{}^\gamma - p^\gamma)\, (2\, k_1{}^\mu - p^\mu)\left(-2\, (k_1 \cdot p) + 2\, (k_2 \cdot p) + p^2 - 2\, (k_1 \cdot k_2) + k_1{}^2 + k_2{}^2\right)(\, k_2 \cdot u\,)^2}{\left(k_2{}^2\right)^2 . k_1{}^2 .(\, k_1 - p\,)^{2\,2} .(\, k_1 + k_2 - p\,)^2}$$

$$\tilde{\Pi}^{\gamma\mu}_{16\,\mathrm{LV}}(p) = \frac{i\, \mathrm{e}^4\, Q_1\, (2\, k_1{}^\gamma - p^\gamma)\, (2\, k_1{}^\mu - p^\mu)\left(-2\, (k_1 \cdot p) + 2\, (k_2 \cdot p) + p^2 - 2\, (k_1 \cdot k_2) + k_1{}^2 + k_2{}^2\right)(\, k_2 \cdot u\,)^2}{\left(k_2{}^2\right)^2 . k_1{}^2 .(\, k_1 - p\,)^{2\,2} .(\, k_1 + k_2 - p\,)^2}$$

$$\tilde{\Pi}^{\gamma\mu}_{17\,\mathrm{LV}}(p) = -\frac{1}{\left(k_2{}^2\right)^2 . k_1{}^2 .(\, k_1 - p\,)^{2\,2} .(\, k_1 + k_2 - p\,)^2}\, 2\, i\, \mathrm{e}^4\, Q_2\, (2\, k_1{}^\gamma - p^\gamma)\, (2\, k_1{}^\mu - p^\mu)$$
$$\Big(-2\, (k_1 \cdot p)\, (\, k_2 \cdot u\,)^2 + k_2{}^2\, (\, p \cdot u\,)^2 + p^2\, (\, k_2 \cdot u\,)^2 + k_2{}^2\, (\, k_1 \cdot u\,)^2 + k_1{}^2\, (\, k_2 \cdot u\,)^2 - 2\, (k_1 \cdot u)$$
$$\left(-(k_2 \cdot p)\, (k_2 \cdot u) + k_2{}^2\, (p \cdot u) + (k_1 \cdot k_2)\, (k_2 \cdot u)\right) + 2\, (p \cdot u)\, (k_1 \cdot k_2)\, (k_2 \cdot u) - 2\, (k_2 \cdot p)\, (p \cdot u)\, (k_2 \cdot u)\Big)$$

$$\tilde{\Pi}^{\gamma\mu}_{18\,\mathrm{LV}}(p) = -\frac{1}{\left(k_2{}^2\right)^2 . k_1{}^2 .( k_1 - p )^{2\,2} .( k_1 + k_2 - p )^2} 2\, i\, \mathrm{e}^4\, Q_2\, (2\, k_1{}^{\gamma} - p^{\gamma})\, (2\, k_1{}^{\mu} - p^{\mu})$$
$$\left(-2\, (k_1 \cdot p)\, ( k_2 \cdot u )^2 + k_2{}^2\, ( p \cdot u )^2 + p^2\, ( k_2 \cdot u )^2 + k_2{}^2\, ( k_1 \cdot u )^2 + k_1{}^2\, ( k_2 \cdot u )^2 - 2\, (k_1 \cdot u)\right.$$
$$\left.\left(-(k_2 \cdot p)\, (k_2 \cdot u) + k_2{}^2\, (p \cdot u) + (k_1 \cdot k_2)\, (k_2 \cdot u)\right) + 2\, (p \cdot u)\, (k_1 \cdot k_2)\, (k_2 \cdot u) - 2\, (k_2 \cdot p)\, (p \cdot u)\, (k_2 \cdot u)\right)$$

$$\tilde{\Pi}^{\gamma\mu}_{19\,\mathrm{LV}}(p) = \frac{2\, i\, \mathrm{e}^4\, Q_1\, u^{\gamma}\, (2\, k_1{}^{\mu} - p^{\mu})\, (-p \cdot u + k_1 \cdot u + k_2 \cdot u)}{k_2{}^2 . k_1{}^2 .( k_1 - p )^2 .( -k_1 + k_2 + p )^2}$$

$$\tilde{\Pi}^{\gamma\mu}_{20\,\mathrm{LV}}(p) = \frac{2\, i\, \mathrm{e}^4\, Q_1\, u^{\gamma}\, (2\, k_1{}^{\mu} - p^{\mu})\, (-p \cdot u + k_1 \cdot u + k_2 \cdot u)}{k_2{}^2 . k_1{}^2 .( k_1 - p )^2 .( -k_1 + k_2 + p )^2}$$

$$\tilde{\Pi}^{\gamma\mu}_{21\,\mathrm{LV}}(p) = \frac{i\, \mathrm{e}^2\, \lambda\, Q_1\, u^{\gamma}\, (2\, k_1{}^{\mu} - p^{\mu})\, (2\, (k_1 \cdot u) - p \cdot u)}{k_1{}^2 . k_2{}^2 .( k_1 - p )^{2\,2}}$$

$$\tilde{\Pi}^{\gamma\mu}_{22\,\mathrm{LV}}(p) = \frac{i\, \mathrm{e}^2\, \lambda\, Q_1\, u^{\gamma}\, (2\, k_1{}^{\mu} - p^{\mu})\, (2\, (k_1 \cdot u) - p \cdot u)}{k_1{}^2 . k_2{}^2 .( k_1 - p )^{2\,2}}$$

$$\tilde{\Pi}^{\gamma\mu}_{23\,\mathrm{LV}}(p) = \frac{i\, D\, \mathrm{e}^4\, Q_1\, u^{\gamma}\, (2\, k_1{}^{\mu} - p^{\mu})\, (2\, (k_1 \cdot u) - p \cdot u)}{k_1{}^2 . k_2{}^2 .( k_1 - p )^{2\,2}}$$

$$\tilde{\Pi}^{\gamma\mu}_{24\,\mathrm{LV}}(p) = \frac{i\, D\, \mathrm{e}^4\, Q_1\, u^{\gamma}\, (2\, k_1{}^{\mu} - p^{\mu})\, (2\, (k_1 \cdot u) - p \cdot u)}{k_1{}^2 . k_2{}^2 .( k_1 - p )^{2\,2}}$$

$$\tilde{\Pi}^{\gamma\mu}_{25\,\mathrm{LV}}(p) = \frac{2\, i\, \mathrm{e}^4\, Q_1\, u^{\gamma}\, (p^{\mu} + 2\, k_1{}^{\mu})\, (k_1 \cdot u - k_2 \cdot u)}{k_2{}^2 . k_1{}^2 .( k_1 + p )^2 .( k_1 + k_2 )^2}$$

$$\tilde{\Pi}^{\gamma\mu}_{26\,\mathrm{LV}}(p) = \frac{2\, i\, \mathrm{e}^4\, Q_1\, u^{\gamma}\, (p^{\mu} + 2\, k_1{}^{\mu})\, (k_1 \cdot u - k_2 \cdot u)}{k_2{}^2 . k_1{}^2 .( k_1 + p )^2 .( k_1 + k_2 )^2}$$

$$\tilde{\Pi}^{\gamma\mu}_{29\,\mathrm{LV}}(p) = \frac{4\, i\, \mathrm{e}^4\, Q_1\, g^{\mu\,\gamma}\, ( k_1 \cdot u )^2}{k_1{}^2 . k_2{}^2 . k_1{}^2 .( -k_1 + k_2 + p )^2}$$

$$\tilde{\Pi}^{\gamma\mu}_{30\,\mathrm{LV}}(p) = \frac{4\, i\, \mathrm{e}^4\, Q_1\, g^{\mu\,\gamma}\, ( k_1 \cdot u )^2}{k_1{}^2 . k_2{}^2 . k_1{}^2 .( -k_1 + k_2 + p )^2}$$

$$\tilde{\Pi}^{\gamma\mu}_{31\,\mathrm{LV}}(p) = -\frac{2\, i\, \mathrm{e}^4\, Q_2\, \left((k_1 \cdot u)\, (g^{\mu\,\gamma}\, (k_1 \cdot u) - k_1{}^{\mu}\, u^{\gamma}) + u^{\mu}\, \left(k_1{}^2\, u^{\gamma} - k_1{}^{\gamma}\, (k_1 \cdot u)\right)\right)}{k_1{}^2 . k_2{}^2 . k_1{}^2 .( -k_1 + k_2 + p )^2}$$

$$\tilde{\Pi}^{\gamma\mu}_{32\,\mathrm{LV}}(p) = \frac{2\, i\, \mathrm{e}^4\, Q_1\, u^{\mu}\, (p^{\gamma} + 2\, k_1{}^{\gamma})\, (k_1 \cdot u + k_2 \cdot u)}{k_2{}^2 . k_1{}^2 .( k_1 + p )^2 .( k_2 - k_1 )^2}$$

$$\tilde{\Pi}^{\gamma\mu}_{33\,\mathrm{LV}}(p) = \frac{2\, i\, \mathrm{e}^4\, Q_1\, u^{\mu}\, (p^{\gamma} + 2\, k_1{}^{\gamma})\, (k_1 \cdot u + k_2 \cdot u)}{k_2{}^2 . k_1{}^2 .( k_1 + p )^2 .( k_2 - k_1 )^2}$$

$$\tilde{\Pi}^{\gamma\mu}_{34\,\mathrm{LV}}(p) = \frac{2\, i\, \mathrm{e}^4\, Q_1\, u^{\gamma}\, (2\, k_1{}^{\mu} + k_2{}^{\mu})\, (p \cdot u + 2\, (k_1 \cdot u) + 2\, (k_2 \cdot u))}{k_2{}^2 . k_1{}^2 .( k_1 + k_2 )^2 .( k_1 + k_2 + p )^2}$$

$$\tilde{\Pi}^{\gamma\mu}_{35\,\mathrm{LV}}(p) = \frac{2\, i\, \mathrm{e}^4\, Q_1\, u^{\gamma}\, (2\, k_1{}^{\mu} + k_2{}^{\mu})\, (p \cdot u + 2\, (k_1 \cdot u) + 2\, (k_2 \cdot u))}{k_2{}^2 . k_1{}^2 .( k_1 + k_2 )^2 .( k_1 + k_2 + p )^2}$$

$$\tilde{\Pi}^{\gamma\mu}_{36\,\mathrm{LV}}(p) = \frac{2\, i\, \mathrm{e}^2\, \lambda\, Q_1\, g^{\mu\,\gamma}\, ( k_1 \cdot u )^2}{\left(k_1{}^2\right)^3 . k_2{}^2}$$

$$\tilde{\Pi}^{\gamma\mu}_{37\,\mathrm{LV}}(p) = \frac{2\,i\,\mathrm{e}^2\,\lambda\,Q_1\,g^{\mu\,\gamma}\,(\,k_1\cdot u\,)^2}{\left(k_1{}^2\right)^3.k_2{}^2}$$

$$\tilde{\Pi}^{\gamma\mu}_{38\,\mathrm{LV}}(p) = \frac{2\,i\,D\,\mathrm{e}^4\,Q_1\,g^{\mu\,\gamma}\,(\,k_1\cdot u\,)^2}{\left(k_1{}^2\right)^3.k_2{}^2}$$

$$\tilde{\Pi}^{\gamma\mu}_{39\,\mathrm{LV}}(p) = \frac{2\,i\,D\,\mathrm{e}^4\,Q_1\,g^{\mu\,\gamma}\,(\,k_1\cdot u\,)^2}{\left(k_1{}^2\right)^3.k_2{}^2}$$

$$\tilde{\Pi}^{\gamma\mu}_{40\,\mathrm{LV}}(p) = \frac{2\,i\,\mathrm{e}^4\,Q_1\,g^{\mu\,\gamma}\,(2\,(k_1\cdot u)+k_2\cdot u)^2}{k_2{}^2.k_1{}^2.(\,k_1+k_2\,)^{2\,2}}$$

$$\tilde{\Pi}^{\gamma\mu}_{41\,\mathrm{LV}}(p) = \frac{2\,i\,\mathrm{e}^4\,Q_1\,g^{\mu\,\gamma}\,(2\,(k_1\cdot u)+k_2\cdot u)^2}{k_2{}^2.k_1{}^2.(\,k_1+k_2\,)^{2\,2}}$$

$$\tilde{\Pi}^{\gamma\mu}_{42\,\mathrm{LV}}(p) = \frac{i\,\mathrm{e}^2\,\lambda\,Q_1\,u^\mu\,(p^\gamma+2\,k_1{}^\gamma)\,(p\cdot u+2\,(k_1\cdot u))}{k_1{}^2.k_2{}^2.(\,k_1+p\,)^{2\,2}}$$

$$\tilde{\Pi}^{\gamma\mu}_{43\,\mathrm{LV}}(p) = \frac{i\,\mathrm{e}^2\,\lambda\,Q_1\,u^\mu\,(p^\gamma+2\,k_1{}^\gamma)\,(p\cdot u+2\,(k_1\cdot u))}{k_1{}^2.k_2{}^2.(\,k_1+p\,)^{2\,2}}$$

$$\tilde{\Pi}^{\gamma\mu}_{44\,\mathrm{LV}}(p) = \frac{i\,D\,\mathrm{e}^4\,Q_1\,u^\mu\,(p^\gamma+2\,k_1{}^\gamma)\,(p\cdot u+2\,(k_1\cdot u))}{k_1{}^2.k_2{}^2.(\,k_1+p\,)^{2\,2}}$$

$$\tilde{\Pi}^{\gamma\mu}_{45\,\mathrm{LV}}(p) = \frac{i\,D\,\mathrm{e}^4\,Q_1\,u^\mu\,(p^\gamma+2\,k_1{}^\gamma)\,(p\cdot u+2\,(k_1\cdot u))}{k_1{}^2.k_2{}^2.(\,k_1+p\,)^{2\,2}}$$

$$\tilde{\Pi}^{\gamma\mu}_{46\,\mathrm{LV}}(p) = \frac{2\,i\,\mathrm{e}^4\,Q_1\,u^\mu\,(2\,k_1{}^\gamma+k_2{}^\gamma)\,(-p\cdot u+2\,(k_1\cdot u)+2\,(k_2\cdot u))}{k_2{}^2.k_1{}^2.(\,k_1+k_2\,)^2.(\,k_1+k_2-p\,)^2}$$

$$\tilde{\Pi}^{\gamma\mu}_{47\,\mathrm{LV}}(p) = \frac{2\,i\,\mathrm{e}^4\,Q_1\,u^\mu\,(2\,k_1{}^\gamma+k_2{}^\gamma)\,(-p\cdot u+2\,(k_1\cdot u)+2\,(k_2\cdot u))}{k_2{}^2.k_1{}^2.(\,k_1+k_2\,)^2.(\,k_1+k_2-p\,)^2}$$

$$\tilde{\Pi}^{\gamma\mu}_{48\,\mathrm{LV}}(p) = \frac{2\,i\,\mathrm{e}^4\,Q_1\,u^\mu\,(2\,k_1{}^\gamma-p^\gamma)\,(k_1\cdot u-k_2\cdot u)}{k_2{}^2.k_1{}^2.(\,k_1-p\,)^2.(\,k_1+k_2\,)^2}$$

$$\tilde{\Pi}^{\gamma\mu}_{49\,\mathrm{LV}}(p) = \frac{2\,i\,\mathrm{e}^4\,Q_1\,u^\mu\,(2\,k_1{}^\gamma-p^\gamma)\,(k_1\cdot u-k_2\cdot u)}{k_2{}^2.k_1{}^2.(\,k_1-p\,)^2.(\,k_1+k_2\,)^2}$$

$$\tilde{\Pi}^{\gamma\mu}_{50\,\mathrm{LV}}(p) = -\frac{i\,\mathrm{e}^2\,\lambda\,Q_1\,(2\,k_1{}^\gamma-p^\gamma)\,(2\,k_1{}^\mu-p^\mu)\,(\,k_1\cdot u\,)^2}{\left(k_1{}^2\right)^3.k_2{}^2.(\,k_1-p\,)^2}$$

$$\tilde{\Pi}^{\gamma\mu}_{51\,\mathrm{LV}}(p) = -\frac{i\,\mathrm{e}^2\,\lambda\,Q_1\,(2\,k_1{}^\gamma-p^\gamma)\,(2\,k_1{}^\mu-p^\mu)\,(\,k_1\cdot u\,)^2}{\left(k_1{}^2\right)^3.k_2{}^2.(\,k_1-p\,)^2}$$

$$\tilde{\Pi}^{\gamma\mu}_{52\,\mathrm{LV}}(p) = -\frac{i\,D\,\mathrm{e}^4\,Q_1\,(2\,k_1{}^\gamma-p^\gamma)\,(2\,k_1{}^\mu-p^\mu)\,(\,k_1\cdot u\,)^2}{\left(k_1{}^2\right)^3.k_2{}^2.(\,k_1-p\,)^2}$$

$$\tilde{\Pi}^{\gamma\mu}_{53\,\mathrm{LV}}(p) = -\frac{i\,D\,\mathrm{e}^4\,Q_1\,(2\,k_1{}^\gamma-p^\gamma)\,(2\,k_1{}^\mu-p^\mu)\,(\,k_1\cdot u\,)^2}{\left(k_1{}^2\right)^3.k_2{}^2.(\,k_1-p\,)^2}$$

$$\tilde{\Pi}^{\gamma\mu}_{54\,\mathrm{LV}}(p) = -\frac{i\,\mathrm{e}^2\,\lambda\,Q_1\,(2\,k_1{}^\gamma-p^\gamma)\,(2\,k_1{}^\mu-p^\mu)\,(\,k_1\cdot u\,)^2}{\left(k_1{}^2\right)^2.k_2{}^2.(\,k_1-p\,)^{2\,2}}$$

$$\tilde{\Pi}^{\gamma\mu}_{55\,\mathrm{LV}}(p) = -\frac{i\,\mathrm{e}^2\,\lambda\,Q_1\,(2\,k_1{}^{\gamma} - p^{\gamma})\,(2\,k_1{}^{\mu} - p^{\mu})\,(\,k_1\cdot u\,)^2}{\left(k_1{}^2\right)^2.k_2{}^2.(\,k_1 - p\,)^{2^2}}$$

$$\tilde{\Pi}^{\gamma\mu}_{56\,\mathrm{LV}}(p) = -\frac{i\,D\,\mathrm{e}^4\,Q_1\,(2\,k_1{}^{\gamma} - p^{\gamma})\,(2\,k_1{}^{\mu} - p^{\mu})\,(\,k_1\cdot u\,)^2}{\left(k_1{}^2\right)^2.k_2{}^2.(\,k_1 - p\,)^{2^2}}$$

$$\tilde{\Pi}^{\gamma\mu}_{57\,\mathrm{LV}}(p) = -\frac{i\,D\,\mathrm{e}^4\,Q_1\,(2\,k_1{}^{\gamma} - p^{\gamma})\,(2\,k_1{}^{\mu} - p^{\mu})\,(\,k_1\cdot u\,)^2}{\left(k_1{}^2\right)^2.k_2{}^2.(\,k_1 - p\,)^{2^2}}$$

$$\tilde{\Pi}^{\gamma\mu}_{58\,\mathrm{LV}}(p) = -\frac{i\,\mathrm{e}^2\,\lambda\,Q_1\,(2\,k_1{}^{\mu} - p^{\mu})\,(p^{\gamma} + 2\,k_2{}^{\gamma})\,(\,k_1\cdot u\,)^2}{\left(k_1{}^2\right)^2.k_2{}^2.(\,k_1 - p\,)^2.(\,k_2 + p\,)^2}$$

$$\tilde{\Pi}^{\gamma\mu}_{59\,\mathrm{LV}}(p) = \frac{i\,\mathrm{e}^2\,\lambda\,Q_1\,(2\,k_1{}^{\mu} - p^{\mu})\,(p^{\gamma} + 2\,k_2{}^{\gamma})\,(\,k_1\cdot u\,)^2}{\left(k_1{}^2\right)^2.k_2{}^2.(\,k_1 - p\,)^2.(\,k_2 + p\,)^2}$$

$$\tilde{\Pi}^{\gamma\mu}_{60\,\mathrm{LV}}(p) = -\frac{i\,\mathrm{e}^2\,\lambda\,Q_1\,(2\,k_1{}^{\gamma} - p^{\gamma})\,(2\,k_1{}^{\mu} - p^{\mu})\,(k_1\cdot u - p\cdot u)^2}{k_1{}^2.k_2{}^2.(\,k_1 - p\,)^{2^3}}$$

$$\tilde{\Pi}^{\gamma\mu}_{61\,\mathrm{LV}}(p) = -\frac{i\,\mathrm{e}^2\,\lambda\,Q_1\,(2\,k_1{}^{\gamma} - p^{\gamma})\,(2\,k_1{}^{\mu} - p^{\mu})\,(k_1\cdot u - p\cdot u)^2}{k_1{}^2.k_2{}^2.(\,k_1 - p\,)^{2^3}}$$

$$\tilde{\Pi}^{\gamma\mu}_{62\,\mathrm{LV}}(p) = -\frac{i\,D\,\mathrm{e}^4\,Q_1\,(2\,k_1{}^{\gamma} - p^{\gamma})\,(2\,k_1{}^{\mu} - p^{\mu})\,(k_1\cdot u - p\cdot u)^2}{k_1{}^2.k_2{}^2.(\,k_1 - p\,)^{2^3}}$$

$$\tilde{\Pi}^{\gamma\mu}_{63\,\mathrm{LV}}(p) = -\frac{i\,D\,\mathrm{e}^4\,Q_1\,(2\,k_1{}^{\gamma} - p^{\gamma})\,(2\,k_1{}^{\mu} - p^{\mu})\,(k_1\cdot u - p\cdot u)^2}{k_1{}^2.k_2{}^2.(\,k_1 - p\,)^{2^3}}$$

$$\tilde{\Pi}^{\gamma\mu}_{64\,\mathrm{LV}}(p) = -\frac{i\,\mathrm{e}^2\,\lambda\,Q_1\,(2\,k_1{}^{\gamma} - p^{\gamma})\,(2\,k_1{}^{\mu} - p^{\mu})\,(\,k_2\cdot u\,)^2}{k_1{}^2.\left(k_2{}^2\right)^2.(\,k_1 - p\,)^{2^2}}$$

$$\tilde{\Pi}^{\gamma\mu}_{65\,\mathrm{LV}}(p) = -\frac{i\,\mathrm{e}^2\,\lambda\,Q_1\,(2\,k_1{}^{\gamma} - p^{\gamma})\,(2\,k_1{}^{\mu} - p^{\mu})\,(\,k_2\cdot u\,)^2}{k_1{}^2.\left(k_2{}^2\right)^2.(\,k_1 - p\,)^{2^2}}$$

$$\tilde{\Pi}^{\gamma\mu}_{66\,\mathrm{LV}}(p) = \frac{i\,(D-2)\,\mathrm{e}^4\,Q_2\,(2\,k_1{}^{\gamma} - p^{\gamma})\,(2\,k_1{}^{\mu} - p^{\mu})\,(\,k_2\cdot u\,)^2}{2\,k_1{}^2.\left(k_2{}^2\right)^2.(\,k_1 - p\,)^{2^2}}$$

$$\tilde{\Pi}^{\gamma\mu}_{67\,\mathrm{LV}}(p) = \frac{i\,(D-2)\,\mathrm{e}^4\,Q_2\,(2\,k_1{}^{\gamma} - p^{\gamma})\,(2\,k_1{}^{\mu} - p^{\mu})\,(\,k_2\cdot u\,)^2}{2\,k_1{}^2.\left(k_2{}^2\right)^2.(\,k_1 - p\,)^{2^2}}$$

$$\tilde{\Pi}^{\gamma\mu}_{68\,\mathrm{LV}}(p) = -\frac{i\,\mathrm{e}^2\,\lambda\,Q_1\,(2\,k_1{}^{\mu} - p^{\mu})\,(2\,k_2{}^{\gamma} - p^{\gamma})\,(\,k_2\cdot u\,)^2}{\left(k_2{}^2\right)^2.k_1{}^2.(\,k_2 - p\,)^2.(\,k_1 - p\,)^2}$$

$$\tilde{\Pi}^{\gamma\mu}_{69\,\mathrm{LV}}(p) = \frac{i\,\mathrm{e}^2\,\lambda\,Q_1\,(2\,k_1{}^{\mu} - p^{\mu})\,(2\,k_2{}^{\gamma} - p^{\gamma})\,(\,k_2\cdot u\,)^2}{\left(k_2{}^2\right)^2.k_1{}^2.(\,k_2 - p\,)^2.(\,k_1 - p\,)^2}$$

$$\tilde{\Pi}^{\gamma\mu}_{70\,\mathrm{LV}}(p) = -\frac{2\,i\,\mathrm{e}^4\,Q_1\,(2\,k_1{}^{\mu} - p^{\mu})\,(k_1{}^{\gamma} - (p + k_2)^{\gamma})\,(\,k_1\cdot u\,)^2}{k_1{}^2.k_2{}^2.k_1{}^2.(\,k_1 - p\,)^2.(\,k_1 + k_2 - p\,)^2}$$

$$\tilde{\Pi}^{\gamma\mu}_{71\,\mathrm{LV}}(p) = -\frac{2\,i\,\mathrm{e}^4\,Q_1\,(2\,k_1{}^{\mu} - p^{\mu})\,(k_1{}^{\gamma} - (p + k_2)^{\gamma})\,(\,k_1\cdot u\,)^2}{k_1{}^2.k_2{}^2.k_1{}^2.(\,k_1 - p\,)^2.(\,k_1 + k_2 - p\,)^2}$$

$$\tilde{\Pi}^{\gamma\mu}_{72\,\mathrm{LV}}(p) = -\frac{2\,i\,\mathrm{e}^4\,Q_1\,(2\,k_1{}^{\mu} - p^{\mu})\,(k_1 + k_2)^{\gamma}\,(\,k_1\cdot u\,)^2}{k_1{}^2.k_2{}^2.k_1{}^2.(\,k_1 - p\,)^2.(\,k_2 - k_1\,)^2}$$

$$\tilde{\Pi}^{\gamma\mu}_{73\,\mathrm{LV}}(p) = -\frac{2\,i\,\mathrm{e}^4\,Q_1\,(2\,k_1{}^{\mu} - p^{\mu})\,(k_1 + k_2)^{\gamma}\,(\,k_1 \cdot u\,)^2}{k_1{}^2.k_2{}^2.k_1{}^2.(\,k_1 - p\,)^2.(\,k_2 - k_1\,)^2}$$

$$\tilde{\Pi}^{\gamma\mu}_{74\,\mathrm{LV}}(p) = -\frac{i\,\mathrm{e}^4\,Q_1\,(2\,k_1{}^{\gamma} - p^{\gamma})\,(2\,k_1{}^{\mu} - p^{\mu})\,(p \cdot u - (k_1 \cdot u) + k_2 \cdot u)^2}{k_2{}^2.k_1{}^2.(\,k_1 - p\,)^{2\,2}.(\,k_1 + k_2 - p\,)^2}$$

$$\tilde{\Pi}^{\gamma\mu}_{75\,\mathrm{LV}}(p) = -\frac{i\,\mathrm{e}^4\,Q_1\,(2\,k_1{}^{\gamma} - p^{\gamma})\,(2\,k_1{}^{\mu} - p^{\mu})\,(p \cdot u - (k_1 \cdot u) + k_2 \cdot u)^2}{k_2{}^2.k_1{}^2.(\,k_1 - p\,)^{2\,2}.(\,k_1 + k_2 - p\,)^2}$$

$$\tilde{\Pi}^{\gamma\mu}_{76\,\mathrm{LV}}(p) = -\frac{i\,\mathrm{e}^4\,Q_1\,(2\,k_1{}^{\gamma} - p^{\gamma})\,(2\,k_1{}^{\mu} - p^{\mu})\,(-p \cdot u + k_1 \cdot u + k_2 \cdot u)^2}{k_2{}^2.k_1{}^2.(\,k_1 - p\,)^{2\,2}.(\,-k_1 + k_2 + p\,)^2}$$

$$\tilde{\Pi}^{\gamma\mu}_{77\,\mathrm{LV}}(p) = -\frac{i\,\mathrm{e}^4\,Q_1\,(2\,k_1{}^{\gamma} - p^{\gamma})\,(2\,k_1{}^{\mu} - p^{\mu})\,(-p \cdot u + k_1 \cdot u + k_2 \cdot u)^2}{k_2{}^2.k_1{}^2.(\,k_1 - p\,)^{2\,2}.(\,-k_1 + k_2 + p\,)^2}$$

$$\tilde{\Pi}^{\gamma\mu}_{78\,\mathrm{LV}}(p) = -\frac{i\,\mathrm{e}^4\,Q_1\,u^{\gamma}\,(p^{\mu} + 2\,k_1{}^{\mu})\left(2\,(k_1 \cdot k_2) + k_1{}^2 + k_2{}^2\right)(p \cdot u + 2\,(k_1 \cdot u))}{k_2{}^2.\left(k_1{}^2\right)^2.(\,k_1 + p\,)^2.(\,k_2 - k_1\,)^2}$$

$$\tilde{\Pi}^{\gamma\mu}_{79\,\mathrm{LV}}(p) = -\frac{i\,\mathrm{e}^4\,Q_1\,u^{\gamma}\,(p^{\mu} + 2\,k_1{}^{\mu})\left(2\,(k_1 \cdot k_2) + k_1{}^2 + k_2{}^2\right)(p \cdot u + 2\,(k_1 \cdot u))}{k_2{}^2.\left(k_1{}^2\right)^2.(\,k_1 + p\,)^2.(\,k_2 - k_1\,)^2}$$

$$\tilde{\Pi}^{\gamma\mu}_{80\,\mathrm{LV}}(p) = -\frac{i\,\mathrm{e}^4\,Q_1\,u^{\gamma}\,(p^{\mu} + 2\,k_1{}^{\mu})\left(4\,(k_1 \cdot p) - 2\,(k_2 \cdot p) - 4\,(k_1 \cdot k_2) + 4\,k_1{}^2 + k_2{}^2\right)(p \cdot u + 2\,(k_1 \cdot u) - 2\,(k_2 \cdot u))}{k_2{}^2.k_1{}^2.(\,k_1 + p\,)^2.(\,k_1 - k_2\,)^2.(\,-k_1 + k_2 - p\,)^2}$$

$$\tilde{\Pi}^{\gamma\mu}_{81\,\mathrm{LV}}(p) = -\frac{2\,i\,\mathrm{e}^4\,Q_1\,(2\,k_1{}^{\gamma} - p^{\gamma})\,(k_1{}^{\mu} - k_2{}^{\mu})\,(\,k_1 \cdot u\,)^2}{k_1{}^2.k_2{}^2.k_1{}^2.(\,k_1 - p\,)^2.(\,k_1 + k_2\,)^2}$$

$$\tilde{\Pi}^{\gamma\mu}_{82\,\mathrm{LV}}(p) = -\frac{2\,i\,\mathrm{e}^4\,Q_1\,(2\,k_1{}^{\gamma} - p^{\gamma})\,(k_1{}^{\mu} - k_2{}^{\mu})\,(\,k_1 \cdot u\,)^2}{k_1{}^2.k_2{}^2.k_1{}^2.(\,k_1 - p\,)^2.(\,k_1 + k_2\,)^2}$$

$$\tilde{\Pi}^{\gamma\mu}_{83\,\mathrm{LV}}(p) = -\frac{2\,i\,\mathrm{e}^4\,Q_1\,(2\,k_1{}^{\gamma} - p^{\gamma})\,((k_1 + k_2)^{\mu} - p^{\mu})\,(\,k_1 \cdot u\,)^2}{k_1{}^2.k_2{}^2.k_1{}^2.(\,k_1 - p\,)^2.(\,-k_1 + k_2 + p\,)^2}$$

$$\tilde{\Pi}^{\gamma\mu}_{84\,\mathrm{LV}}(p) = -\frac{2\,i\,\mathrm{e}^4\,Q_1\,(2\,k_1{}^{\gamma} - p^{\gamma})\,((k_1 + k_2)^{\mu} - p^{\mu})\,(\,k_1 \cdot u\,)^2}{k_1{}^2.k_2{}^2.k_1{}^2.(\,k_1 - p\,)^2.(\,-k_1 + k_2 + p\,)^2}$$

$$\tilde{\Pi}^{\gamma\mu}_{85\,\mathrm{LV}}(p) = -\frac{2\,i\,\mathrm{e}^4\,Q_1\,g^{\mu\,\gamma}\left(2\,(k_1 \cdot k_2) + k_1{}^2 + k_2{}^2\right)(\,k_1 \cdot u\,)^2}{k_1{}^2.k_2{}^2.\left(k_1{}^2\right)^2.(\,k_2 - k_1\,)^2}$$

$$\tilde{\Pi}^{\gamma\mu}_{86\,\mathrm{LV}}(p) = -\frac{2\,i\,\mathrm{e}^4\,Q_1\,g^{\mu\,\gamma}\left(2\,(k_1 \cdot k_2) + k_1{}^2 + k_2{}^2\right)(\,k_1 \cdot u\,)^2}{k_1{}^2.k_2{}^2.\left(k_1{}^2\right)^2.(\,k_2 - k_1\,)^2}$$

$$\tilde{\Pi}^{\gamma\mu}_{87\,\mathrm{LV}}(p) = -\frac{2\,i\,\mathrm{e}^4\,Q_1\,g^{\mu\,\gamma}\left(-4\,(k_1 \cdot k_2) + 4\,k_1{}^2 + k_2{}^2\right)(\,k_1 \cdot u\,)^2}{k_1{}^2.k_2{}^2.k_1{}^2.(\,k_2 - k_1\,)^2.(\,k_1 - k_2\,)^2}$$

$$\tilde{\Pi}^{\gamma\mu}_{88\,\mathrm{LV}}(p) = \frac{4\,i\,\mathrm{e}^4\,Q_2\,g^{\mu\,\gamma}\left(k_2{}^2\,(\,k_1 \cdot u\,)^2 + k_1{}^2\,(\,k_2 \cdot u\,)^2 - 2\,(k_1 \cdot k_2)\,(k_1 \cdot u)\,(k_2 \cdot u)\right)}{k_1{}^2.k_2{}^2.k_1{}^2.(\,k_2 - k_1\,)^2.(\,k_1 - k_2\,)^2}$$

$$\tilde{\Pi}^{\gamma\mu}_{89\,\mathrm{LV}}(p) = -\frac{i\,\mathrm{e}^4\,Q_1\,u^{\mu}\,(2\,k_1{}^{\gamma} - p^{\gamma})\left(2\,(k_1 \cdot k_2) + k_1{}^2 + k_2{}^2\right)(2\,(k_1 \cdot u) - p \cdot u)}{k_2{}^2.\left(k_1{}^2\right)^2.(\,k_1 - p\,)^2.(\,k_2 - k_1\,)^2}$$

$$\tilde{\Pi}^{\gamma\mu}_{90\,\mathrm{LV}}(p) = -\frac{i\,\mathrm{e}^4\,Q_1\,u^{\mu}\,(2\,k_1{}^{\gamma} - p^{\gamma})\left(2\,(k_1 \cdot k_2) + k_1{}^2 + k_2{}^2\right)(2\,(k_1 \cdot u) - p \cdot u)}{k_2{}^2.\left(k_1{}^2\right)^2.(\,k_1 - p\,)^2.(\,k_2 - k_1\,)^2}$$

$$\tilde{\Pi}^{\gamma\mu}_{91\,\mathrm{LV}}(p) = -\frac{i\, e^4\, Q_1\, u^\mu\, (2\, k_1{}^\gamma - p^\gamma)\left(-4\, (k_1 \cdot p) + 2\, (k_2 \cdot p) - 4\, (k_1 \cdot k_2) + 4\, k_1{}^2 + k_2{}^2\right)(-p \cdot u + 2\, (k_1 \cdot u) - 2\, (k_2 \cdot u))}{k_2{}^2 . k_1{}^2 .(\, k_1 - p\,)^2 .(\, k_1 - k_2\,)^2 .(\, -k_1 + k_2 + p\,)^2}$$

$$\tilde{\Pi}^{\gamma\mu}_{92\,\mathrm{LV}}(p) =$$
$$-\Big(\big(2\, i\, e^4\, Q_2\, (p^\mu + 2\, k_1{}^\mu)\, (p^\gamma + 2\, k_1{}^\gamma + 2\, k_2{}^\gamma)\, \big(k_2{}^2\, (\, k_1 \cdot u\,)^2 + (k_1 \cdot u)\, \big(-(k_2 \cdot p)\, (k_2 \cdot u) + k_2{}^2\, (p \cdot u) - 2\, (k_1 \cdot k_2)\, (k_2 \cdot u)\big) +$$
$$(k_2 \cdot u)\, \big((k_1 \cdot p)\, (k_2 \cdot u) - (p \cdot u)\, (k_1 \cdot k_2) + k_1{}^2\, (k_2 \cdot u)\big)\big)\big) \Big/ \left(\left(k_2{}^2\right)^2 . k_1{}^2 .(\, k_1 + p\,)^2 .(\, k_1 + k_2\,)^2 .(\, k_1 + k_2 + p\,)^2\right)$$

$$\tilde{\Pi}^{\gamma\mu}_{93\,\mathrm{LV}}(p) = \frac{i\, e^4\, Q_1\, (2\, k_1{}^\gamma - p^\gamma)\, (2\, k_1{}^\mu - p^\mu)\left(-2\, (k_1 \cdot p) - 2\, (k_2 \cdot p) + p^2 + 2\, (k_1 \cdot k_2) + k_1{}^2 + k_2{}^2\right)(\, k_1 \cdot u\,)^2}{k_1{}^2 . k_2{}^2 . k_1{}^2 .(\, k_1 - p\,)^{2^2} .(\, -k_1 + k_2 + p\,)^2}$$

$$\tilde{\Pi}^{\gamma\mu}_{94\,\mathrm{LV}}(p) = \frac{i\, e^4\, Q_1\, (2\, k_1{}^\gamma - p^\gamma)\, (2\, k_1{}^\mu - p^\mu)\left(-2\, (k_1 \cdot p) - 2\, (k_2 \cdot p) + p^2 + 2\, (k_1 \cdot k_2) + k_1{}^2 + k_2{}^2\right)(\, k_1 \cdot u\,)^2}{k_1{}^2 . k_2{}^2 . k_1{}^2 .(\, k_1 - p\,)^{2^2} .(\, -k_1 + k_2 + p\,)^2}$$

$$\tilde{\Pi}^{\gamma\mu}_{95\,\mathrm{LV}}(p) = \frac{i\, e^4\, Q_1\, (2\, k_1{}^\gamma - p^\gamma)\, (2\, k_1{}^\mu - p^\mu)\left(-2\, (k_1 \cdot k_2) + k_1{}^2 + k_2{}^2\right)(\, k_1 \cdot u\,)^2}{\left(k_1{}^2\right)^2 . k_2{}^2 . k_1{}^2 .(\, k_1 - p\,)^2 .(\, k_1 + k_2\,)^2}$$

$$\tilde{\Pi}^{\gamma\mu}_{96\,\mathrm{LV}}(p) = \frac{i\, e^4\, Q_1\, (2\, k_1{}^\gamma - p^\gamma)\, (2\, k_1{}^\mu - p^\mu)\left(-2\, (k_1 \cdot k_2) + k_1{}^2 + k_2{}^2\right)(\, k_1 \cdot u\,)^2}{\left(k_1{}^2\right)^2 . k_2{}^2 . k_1{}^2 .(\, k_1 - p\,)^2 .(\, k_1 + k_2\,)^2}$$

$$\tilde{\Pi}^{\gamma\mu}_{97\,\mathrm{LV}}(p) = \frac{i\, e^4\, Q_1\, (2\, k_1{}^\gamma - p^\gamma)\, (2\, k_1{}^\mu - p^\mu)\left(-2\, (k_1 \cdot p) - 2\, (k_2 \cdot p) + p^2 + 2\, (k_1 \cdot k_2) + k_1{}^2 + k_2{}^2\right)(k_1 \cdot u - p \cdot u)^2}{k_2{}^2 . k_1{}^2 .(\, k_1 - p\,)^{2^3} .(\, -k_1 + k_2 + p\,)^2}$$

$$\tilde{\Pi}^{\gamma\mu}_{98\,\mathrm{LV}}(p) = \frac{i\, e^4\, Q_1\, (2\, k_1{}^\gamma - p^\gamma)\, (2\, k_1{}^\mu - p^\mu)\left(-2\, (k_1 \cdot p) - 2\, (k_2 \cdot p) + p^2 + 2\, (k_1 \cdot k_2) + k_1{}^2 + k_2{}^2\right)(k_1 \cdot u - p \cdot u)^2}{k_2{}^2 . k_1{}^2 .(\, k_1 - p\,)^{2^3} .(\, -k_1 + k_2 + p\,)^2}$$

$$\tilde{\Pi}^{\gamma\mu}_{100\,\mathrm{LV}}(p) = -\frac{2\, i\, e^2\, \lambda\, Q_1\, u^\gamma\, u^\mu}{\left(k_2{}^2\right)^2 . k_1{}^2}$$

$$\tilde{\Pi}^{\gamma\mu}_{101\,\mathrm{LV}}(p) = -\frac{2\, i\, D\, e^4\, Q_1\, u^\gamma\, u^\mu}{\left(k_2{}^2\right)^2 . k_1{}^2}$$

$$\tilde{\Pi}^{\gamma\mu}_{102\,\mathrm{LV}}(p) = \frac{i\, e^2\, \lambda\, Q_1\, u^\gamma\, (2\, k_1{}^\mu - p^\mu)\, (p \cdot u + 2\, (k_2 \cdot u))}{k_2{}^2 . k_1{}^2 .(\, k_2 + p\,)^2 .(\, k_1 - p\,)^2}$$

$$\tilde{\Pi}^{\gamma\mu}_{103\,\mathrm{LV}}(p) = \frac{2\, i\, e^2\, \lambda\, Q_1\, g^{\mu\,\gamma}\, (\, k_1 \cdot u\,)^2}{\left(k_2{}^2\right)^2 . \left(k_1{}^2\right)^2}$$

$$\tilde{\Pi}^{\gamma\mu}_{104\,\mathrm{LV}}(p) = -\frac{i\, (D - 2)\, e^4\, Q_2\, g^{\mu\,\gamma}\, (\, k_1 \cdot u\,)^2}{\left(k_2{}^2\right)^2 . \left(k_1{}^2\right)^2}$$

$$\tilde{\Pi}^{\gamma\mu}_{105\,\mathrm{LV}}(p) = \frac{i\, e^2\, \lambda\, Q_1\, u^\mu\, (p^\gamma + 2\, k_1{}^\gamma)\, (2\, (k_2 \cdot u) - p \cdot u)}{k_2{}^2 . k_1{}^2 .(\, k_2 - p\,)^2 .(\, k_1 + p\,)^2}$$

$$\tilde{\Pi}^{\gamma\mu}_{106\,\mathrm{LV}}(p) = \frac{2\, i\, e^4\, Q_1\, u^\gamma\, u^\mu \left(4\left(k_1 \cdot k_2 + k_1{}^2\right) + k_2{}^2\right)}{k_2{}^2 . k_1{}^2 .(\, k_1 + k_2\,)^{2^2}}$$

$$\tilde{\Pi}^{\gamma\mu}_{107\,\mathrm{LV}}(p) = -\frac{4\, i\, e^4\, Q_1\, u^\gamma\, u^\mu}{k_2{}^2 . k_1{}^2 .(\, k_1 + k_2 - p\,)^2}$$

$$\tilde{\Pi}^{\gamma\mu}_{108\,\mathrm{LV}}(p) = -\frac{4\, i\, e^4\, Q_1\, u^\gamma\, u^\mu}{k_2{}^2 . k_1{}^2 .(\, k_1 + k_2 + p\,)^2}$$

where we have omitted the vanishing amplitudes that are proportional to $u^2$.

Now, through the process of decomposing the two-loop tensor integral and employing Tarasov's algorithm, we obtain

$$(4\pi)^D\,\Pi^{\gamma\mu}_{1.\mathrm{LV}}(p) = \frac{1}{3\,(D-6)\,(D-4)\,(D-1)\,(3\,D-4)\,p^4}\,2\,i\,e^4\,Q_1\,\mathbf{J}^{(D)}_{\{1,0\}\{1,0\}\{1,0\}}\Big((D-3)\,(p\cdot u)\left(\left(-3\,D^3+20\,D^2-36\,D+16\right)p^2\,g^{\mu\gamma}\,(p\cdot u)+ p^\mu\left(\left(-3\,D^3+27\,D^2-66\,D+40\right)p^2\,u^\gamma+D\,(3\,D-2)\,(D-4)^2\,p^\gamma\,(p\cdot u)\right)\right)+ p^2\,u^\mu\left(\left(3\,D^3-21\,D^2+38\,D-24\right)p^2\,u^\gamma-2\left(3\,D^4-29\,D^3+96\,D^2-124\,D+48\right)p^\gamma\,(p\cdot u)\right)\Big)$$

$$(4\pi)^D\,\Pi^{\gamma\mu}_{2\,\mathrm{LV}}(p) = \frac{1}{3\,(D-6)\,(D-4)\,(D-1)\,(3\,D-4)\,p^4}\,2\,i\,e^4\,Q_1\,\mathbf{J}^{(D)}_{\{1,0\}\{1,0\}\{1,0\}}\Big((D-3)\,(p\cdot u)\left(\left(-3\,D^3+20\,D^2-36\,D+16\right)p^2\,g^{\mu\gamma}\,(p\cdot u)+ p^\mu\left(\left(-3\,D^3+27\,D^2-66\,D+40\right)p^2\,u^\gamma+D\,(3\,D-2)\,(D-4)^2\,p^\gamma\,(p\cdot u)\right)\right)+ p^2\,u^\mu\left(\left(3\,D^3-21\,D^2+38\,D-24\right)p^2\,u^\gamma-2\left(3\,D^4-29\,D^3+96\,D^2-124\,D+48\right)p^\gamma\,(p\cdot u)\right)\Big)$$

$$(4\pi)^D\,\Pi^{\gamma\mu}_{3\,\mathrm{LV}}(p) = \frac{i\,(D-2)\,e^4\,Q_2\,u^\gamma\left((D-3)\,p^\mu\,(p\cdot u)-p^2\,u^\mu\right)\mathbf{J}^{(D)}_{\{1,0\}\{1,0\}\{1,0\}}}{3\,(D-4)\,p^2}$$

$$(4\pi)^D\,\Pi^{\gamma\mu}_{4\,\mathrm{LV}}(p) = \frac{i\,(D-2)\,e^4\,Q_2\,u^\gamma\left((D-3)\,p^\mu\,(p\cdot u)-p^2\,u^\mu\right)\mathbf{J}^{(D)}_{\{1,0\}\{1,0\}\{1,0\}}}{3\,(D-4)\,p^2}$$

$$(4\pi)^D\,\Pi^{\gamma\mu}_{5\,\mathrm{LV}}(p) = \Bigg(i\,e^4\,Q_1\Bigg(p^2\,u^\mu\Bigg(p^2\,u^\gamma\left(3\left(3\,D^4-19\,D^3+20\,D^2+48\,D-64\right)p^2\left(\mathbf{B}^{(D)}_{\{1,0\}\{1,0\}}\right)^2-4\left(9\,D^4-43\,D^3+44\,D^2+48\,D-64\right)\mathbf{J}^{(D)}_{\{1,0\}\{1,0\}\{1,0\}}\right)+p^\gamma\,(p\cdot u)\left(8\left(7\,D^4-36\,D^3+37\,D^2+40\,D-48\right)\mathbf{J}^{(D)}_{\{1,0\}\{1,0\}\{1,0\}}-3\left(3\,D^4-19\,D^3+20\,D^2+48\,D-64\right)p^2\left(\mathbf{B}^{(D)}_{\{1,0\}\{1,0\}}\right)^2\right)\Bigg)+(p\cdot u)\Bigg(p^2\,g^{\mu\gamma}\,(p\cdot u)\left(3\left(6\,D^4-41\,D^3+68\,D^2+16\,D-64\right)p^2\left(\mathbf{B}^{(D)}_{\{1,0\}\{1,0\}}\right)^2-4\,D\left(9\,D^4-52\,D^3+71\,D^2+44\,D-96\right)\mathbf{J}^{(D)}_{\{1,0\}\{1,0\}\{1,0\}}\right)+p^\mu\Bigg(p^2\,u^\gamma\left(8\left(7\,D^4-36\,D^3+37\,D^2+40\,D-48\right)\mathbf{J}^{(D)}_{\{1,0\}\{1,0\}\{1,0\}}-3\left(3\,D^4-19\,D^3+20\,D^2+48\,D-64\right)p^2\left(\mathbf{B}^{(D)}_{\{1,0\}\{1,0\}}\right)^2\right)-(D-2)\,p^\gamma\,(p\cdot u)\left(3\,D\left(3\,D^2-16\,D+16\right)p^2\left(\mathbf{B}^{(D)}_{\{1,0\}\{1,0\}}\right)^2+2\left(9\,D^5-106\,D^4+369\,D^3-300\,D^2-416\,D+384\right)\mathbf{J}^{(D)}_{\{1,0\}\{1,0\}\{1,0\}}\right)\Bigg)\Bigg)\Bigg)\Bigg)\Bigg/\left(3\,(D-4)^2\,(D-2)\,(D-1)\,(D+1)\,(3\,D-4)\,p^4\right)$$

$$(4\pi)^D\,\Pi^{\gamma\mu}_{6\,\mathrm{LV}}(p) = \Bigg(i\,e^4\,Q_1\Bigg(p^2\,u^\mu\Bigg(p^2\,u^\gamma\left(3\left(3\,D^4-19\,D^3+20\,D^2+48\,D-64\right)p^2\left(\mathbf{B}^{(D)}_{\{1,0\}\{1,0\}}\right)^2-4\left(9\,D^4-43\,D^3+44\,D^2+48\,D-64\right)\mathbf{J}^{(D)}_{\{1,0\}\{1,0\}\{1,0\}}\right)+p^\gamma\,(p\cdot u)\left(8\left(7\,D^4-36\,D^3+37\,D^2+40\,D-48\right)\mathbf{J}^{(D)}_{\{1,0\}\{1,0\}\{1,0\}}-3\left(3\,D^4-19\,D^3+20\,D^2+48\,D-64\right)p^2\left(\mathbf{B}^{(D)}_{\{1,0\}\{1,0\}}\right)^2\right)\Bigg)+(p\cdot u)\Bigg(p^2\,g^{\mu\gamma}\,(p\cdot u)\left(3\left(6\,D^4-41\,D^3+68\,D^2+16\,D-64\right)p^2\left(\mathbf{B}^{(D)}_{\{1,0\}\{1,0\}}\right)^2-4\,D\left(9\,D^4-52\,D^3+71\,D^2+44\,D-96\right)\mathbf{J}^{(D)}_{\{1,0\}\{1,0\}\{1,0\}}\right)+p^\mu\Bigg(p^2\,u^\gamma\left(8\left(7\,D^4-36\,D^3+37\,D^2+40\,D-48\right)\mathbf{J}^{(D)}_{\{1,0\}\{1,0\}\{1,0\}}-3\left(3\,D^4-19\,D^3+20\,D^2+48\,D-64\right)p^2\left(\mathbf{B}^{(D)}_{\{1,0\}\{1,0\}}\right)^2\right)-(D-2)\,p^\gamma\,(p\cdot u)\left(3\,D\left(3\,D^2-16\,D+16\right)p^2\left(\mathbf{B}^{(D)}_{\{1,0\}\{1,0\}}\right)^2+2\left(9\,D^5-106\,D^4+369\,D^3-300\,D^2-416\,D+384\right)\mathbf{J}^{(D)}_{\{1,0\}\{1,0\}\{1,0\}}\right)\Bigg)\Bigg)\Bigg)\Bigg)\Bigg/\left(3\,(D-4)^2\,(D-2)\,(D-1)\,(D+1)\,(3\,D-4)\,p^4\right)$$

$$
(4\,\pi)^D\,\Pi^{\gamma\mu}_{7\,\mathrm{LV}}(p) = \frac{1}{3\,(D-6)\,(D-4)\,(D-1)\,(3\,D-4)\,p^4}\,2\,i\,\mathrm{e}^4\,Q_1\,\mathbf{J}^{(D)}_{\{1,0\}\,\{1,0\}\,\{1,0\}}
$$
$$
\Big(\big(3\,D^3-23\,D^2+50\,D-24\big)\,(p\cdot u)\,\big(p^\mu\,\big((D-4)\,D\,p^\gamma\,(p\cdot u)-2\,(D-2)\,p^2\,u^\gamma\big)-(D-2)\,p^2\,g^{\mu\,\gamma}\,(p\cdot u)\big)+
$$
$$
p^2\,u^\mu\,\big(\big(3\,D^3-21\,D^2+38\,D-24\big)\,p^2\,u^\gamma+\big(-3\,D^4+36\,D^3-147\,D^2+238\,D-120\big)\,p^\gamma\,(p\cdot u)\big)\Big)
$$

$$
(4\,\pi)^D\,\Pi^{\gamma\mu}_{8\,\mathrm{LV}}(p) = \frac{1}{3\,(D-6)\,(D-4)\,(D-1)\,(3\,D-4)\,p^4}\,2\,i\,\mathrm{e}^4\,Q_1\,\mathbf{J}^{(D)}_{\{1,0\}\,\{1,0\}\,\{1,0\}}
$$
$$
\Big(\big(3\,D^3-23\,D^2+50\,D-24\big)\,(p\cdot u)\,\big(p^\mu\,\big((D-4)\,D\,p^\gamma\,(p\cdot u)-2\,(D-2)\,p^2\,u^\gamma\big)-(D-2)\,p^2\,g^{\mu\,\gamma}\,(p\cdot u)\big)+
$$
$$
p^2\,u^\mu\,\big(\big(3\,D^3-21\,D^2+38\,D-24\big)\,p^2\,u^\gamma+\big(-3\,D^4+36\,D^3-147\,D^2+238\,D-120\big)\,p^\gamma\,(p\cdot u)\big)\Big)
$$

$$
(4\,\pi)^D\,\Pi^{\gamma\mu}_{9\,\mathrm{LV}}(p) = \frac{i\,(D-2)\,\mathrm{e}^4\,Q_2\,u^\mu\,\big((D-3)\,p^\gamma\,(p\cdot u)-p^2\,u^\gamma\big)\,\mathbf{J}^{(D)}_{\{1,0\}\,\{1,0\}\,\{1,0\}}}{3\,(D-4)\,p^2}
$$

$$
(4\,\pi)^D\,\Pi^{\gamma\mu}_{10\,\mathrm{LV}}(p) = \frac{i\,(D-2)\,\mathrm{e}^4\,Q_2\,u^\mu\,\big((D-3)\,p^\gamma\,(p\cdot u)-p^2\,u^\gamma\big)\,\mathbf{J}^{(D)}_{\{1,0\}\,\{1,0\}\,\{1,0\}}}{3\,(D-4)\,p^2}
$$

$$
(4\,\pi)^D\,\Pi^{\gamma\mu}_{11\,\mathrm{LV}}(p) =
$$
$$
-\Bigg(\Bigg(i\,\mathrm{e}^4\,Q_1\,\Bigg(2\,p^2\,u^\mu\,\Bigg(p^2\,u^\gamma\,\Bigg(3\,\big(6\,D^4-71\,D^3+258\,D^2-304\,D+96\big)\,p^2\,\Big(\mathbf{B}^{(D)}_{\{1,0\}\,\{1,0\}}\Big)^2-8\,\big(2\,D^5-18\,D^4+31\,D^3+33\,D^2-
$$
$$
78\,D+24\big)\,\mathbf{J}^{(D)}_{\{1,0\}\,\{1,0\}\,\{1,0\}}\Bigg)+p^\gamma\,(p\cdot u)\,\Bigg(9\,\big(3\,D^3-34\,D^2+112\,D-96\big)\,p^2\,\Big(\mathbf{B}^{(D)}_{\{1,0\}\,\{1,0\}}\Big)^2-
$$
$$
2\,\big(4\,D^6-41\,D^5+140\,D^4-189\,D^3+18\,D^2+344\,D-384\big)\,\mathbf{J}^{(D)}_{\{1,0\}\,\{1,0\}\,\{1,0\}}\Bigg)\Bigg)+
$$
$$
(p\cdot u)\,\Bigg(p^2\,g^{\mu\,\gamma}\,(p\cdot u)\,\Bigg(8\,\big(2\,D^6-26\,D^5+95\,D^4-41\,D^3-244\,D^2+76\,D+240\big)\,\mathbf{J}^{(D)}_{\{1,0\}\,\{1,0\}\,\{1,0\}}-
$$
$$
3\,\big(6\,D^5-83\,D^4+364\,D^3-412\,D^2-640\,D+960\big)\,p^2\,\Big(\mathbf{B}^{(D)}_{\{1,0\}\,\{1,0\}}\Big)^2\Bigg)+
$$
$$
p^\mu\,\Bigg(p^\gamma\,(p\cdot u)\,\Bigg(3\,\big(6\,D^5-83\,D^4+346\,D^3-208\,D^2-1312\,D+1536\big)\,p^2\,\Big(\mathbf{B}^{(D)}_{\{1,0\}\,\{1,0\}}\Big)^2+
$$
$$
4\,\big(2\,D^7-50\,D^6+443\,D^5-1706\,D^4+2531\,D^3+196\,D^2-2880\,D+1152\big)
$$
$$
\mathbf{J}^{(D)}_{\{1,0\}\,\{1,0\}\,\{1,0\}}\Bigg)-2\,p^2\,u^\gamma\,\Bigg(3\,\big(6\,D^4-71\,D^3+258\,D^2-304\,D+96\big)\,p^2\,\Big(\mathbf{B}^{(D)}_{\{1,0\}\,\{1,0\}}\Big)^2-
$$
$$
4\,\big(4\,D^6-43\,D^5+157\,D^4-243\,D^3+109\,D^2+196\,D-192\big)\,\mathbf{J}^{(D)}_{\{1,0\}\,\{1,0\}\,\{1,0\}}\Bigg)\Bigg)\Bigg)\Bigg)\Bigg)\Bigg/
$$
$$
\Big(6\,(D-6)\,(D-4)^2\,(D-1)\,(D+1)\,(3\,D-4)\,p^4\Big)\Bigg)
$$

$$
(4\,\pi)^D\,\Pi^{\gamma\mu}_{12\,\mathrm{LV}}(p) =
$$
$$
-\Bigg(\Bigg(i\,\mathrm{e}^4\,Q_1\,\Bigg(2\,p^2\,u^\mu\,\Bigg(p^2\,u^\gamma\,\Bigg(3\,\big(6\,D^4-71\,D^3+258\,D^2-304\,D+96\big)\,p^2\,\Big(\mathbf{B}^{(D)}_{\{1,0\}\,\{1,0\}}\Big)^2-8\,\big(2\,D^5-18\,D^4+31\,D^3+33\,D^2-
$$
$$
78\,D+24\big)\,\mathbf{J}^{(D)}_{\{1,0\}\,\{1,0\}\,\{1,0\}}\Bigg)+p^\gamma\,(p\cdot u)\,\Bigg(9\,\big(3\,D^3-34\,D^2+112\,D-96\big)\,p^2\,\Big(\mathbf{B}^{(D)}_{\{1,0\}\,\{1,0\}}\Big)^2-
$$
$$
2\,\big(4\,D^6-41\,D^5+140\,D^4-189\,D^3+18\,D^2+344\,D-384\big)\,\mathbf{J}^{(D)}_{\{1,0\}\,\{1,0\}\,\{1,0\}}\Bigg)\Bigg)+
$$
$$
(p\cdot u)\,\Bigg(p^2\,g^{\mu\,\gamma}\,(p\cdot u)\,\Bigg(8\,\big(2\,D^6-26\,D^5+95\,D^4-41\,D^3-244\,D^2+76\,D+240\big)\,\mathbf{J}^{(D)}_{\{1,0\}\,\{1,0\}\,\{1,0\}}-
$$
$$
3\,\big(6\,D^5-83\,D^4+364\,D^3-412\,D^2-640\,D+960\big)\,p^2\,\Big(\mathbf{B}^{(D)}_{\{1,0\}\,\{1,0\}}\Big)^2\Bigg)+
$$
$$
p^\mu\,\Bigg(p^\gamma\,(p\cdot u)\,\Bigg(3\,\big(6\,D^5-83\,D^4+346\,D^3-208\,D^2-1312\,D+1536\big)\,p^2\,\Big(\mathbf{B}^{(D)}_{\{1,0\}\,\{1,0\}}\Big)^2+
$$
$$
4\,\big(2\,D^7-50\,D^6+443\,D^5-1706\,D^4+2531\,D^3+196\,D^2-2880\,D+1152\big)
$$
$$
\mathbf{J}^{(D)}_{\{1,0\}\,\{1,0\}\,\{1,0\}}\Bigg)-2\,p^2\,u^\gamma\,\Bigg(3\,\big(6\,D^4-71\,D^3+258\,D^2-304\,D+96\big)\,p^2\,\Big(\mathbf{B}^{(D)}_{\{1,0\}\,\{1,0\}}\Big)^2-
$$
$$
4\,\big(4\,D^6-43\,D^5+157\,D^4-243\,D^3+109\,D^2+196\,D-192\big)\,\mathbf{J}^{(D)}_{\{1,0\}\,\{1,0\}\,\{1,0\}}\Bigg)\Bigg)\Bigg)\Bigg)\Bigg)\Bigg/
$$
$$
\Big(6\,(D-6)\,(D-4)^2\,(D-1)\,(D+1)\,(3\,D-4)\,p^4\Big)\Bigg)
$$

$$
\begin{aligned}
(4\pi)^D\, \Pi^{\gamma\mu}_{13\,\mathrm{LV}}(p) = &-\Big(\Big(i\, e^4\, Q_1 \Big(2\, p^2\, u^\mu \Big(p^2\, u^\gamma \Big(3\, (6\, D^4 - 71\, D^3 + 258\, D^2 - 304\, D + 96)\, p^2 \Big(\mathbf{B}^{(D)}_{\{1,0\}\{1,0\}}\Big)^2 - \\
&8\, (2\, D^5 - 18\, D^4 + 31\, D^3 + 33\, D^2 - 78\, D + 24)\, \mathbf{J}^{(D)}_{\{1,0\}\{1,0\}\{1,0\}}\Big) + \\
&p^\gamma\, (p\cdot u) \Big(4\, (4\, D^6 - 43\, D^5 + 157\, D^4 - 243\, D^3 + 109\, D^2 + 196\, D - 192)\, \mathbf{J}^{(D)}_{\{1,0\}\{1,0\}\{1,0\}} - \\
&3\, (6\, D^4 - 71\, D^3 + 258\, D^2 - 304\, D + 96)\, p^2 \Big(\mathbf{B}^{(D)}_{\{1,0\}\{1,0\}}\Big)^2\Big)\Big) + \\
&(p\cdot u) \Big(p^2\, g^{\mu\gamma}\, (p\cdot u) \Big(8\, (2\, D^6 - 26\, D^5 + 95\, D^4 - 41\, D^3 - 244\, D^2 + 76\, D + 240)\, \mathbf{J}^{(D)}_{\{1,0\}\{1,0\}\{1,0\}} - \\
&3\, (6\, D^5 - 83\, D^4 + 364\, D^3 - 412\, D^2 - 640\, D + 960)\, p^2 \Big(\mathbf{B}^{(D)}_{\{1,0\}\{1,0\}}\Big)^2\Big) + \\
&p^\mu \Big(2\, p^2\, u^\gamma \Big(9\, (3\, D^3 - 34\, D^2 + 112\, D - 96)\, p^2 \Big(\mathbf{B}^{(D)}_{\{1,0\}\{1,0\}}\Big)^2 - \\
&2\, (4\, D^6 - 41\, D^5 + 140\, D^4 - 189\, D^3 + 18\, D^2 + 344\, D - 384)\, \mathbf{J}^{(D)}_{\{1,0\}\{1,0\}\{1,0\}}\Big) + \\
&p^\gamma\, (p\cdot u) \Big(3\, (6\, D^5 - 83\, D^4 + 346\, D^3 - 208\, D^2 - 1312\, D + 1536)\, p^2 \Big(\mathbf{B}^{(D)}_{\{1,0\}\{1,0\}}\Big)^2 + \\
&4\, (2\, D^7 - 50\, D^6 + 443\, D^5 - 1706\, D^4 + 2531\, D^3 + 196\, D^2 - 2880\, D + 1152) \\
&\mathbf{J}^{(D)}_{\{1,0\}\{1,0\}\{1,0\}}\Big)\Big)\Big)\Big)\Big) \Big/ \Big(6\, (D-6)\, (D-4)^2\, (D-1)\, (D+1)\, (3\, D-4)\, p^4\Big)\Big)
\end{aligned}
$$

$$
\begin{aligned}
(4\pi)^D\, \Pi^{\gamma\mu}_{14\,\mathrm{LV}}(p) = &-\Big(\Big(i\, e^4\, Q_1 \Big(2\, p^2\, u^\mu \Big(p^2\, u^\gamma \Big(3\, (6\, D^4 - 71\, D^3 + 258\, D^2 - 304\, D + 96)\, p^2 \Big(\mathbf{B}^{(D)}_{\{1,0\}\{1,0\}}\Big)^2 - \\
&8\, (2\, D^5 - 18\, D^4 + 31\, D^3 + 33\, D^2 - 78\, D + 24)\, \mathbf{J}^{(D)}_{\{1,0\}\{1,0\}\{1,0\}}\Big) + \\
&p^\gamma\, (p\cdot u) \Big(4\, (4\, D^6 - 43\, D^5 + 157\, D^4 - 243\, D^3 + 109\, D^2 + 196\, D - 192)\, \mathbf{J}^{(D)}_{\{1,0\}\{1,0\}\{1,0\}} - \\
&3\, (6\, D^4 - 71\, D^3 + 258\, D^2 - 304\, D + 96)\, p^2 \Big(\mathbf{B}^{(D)}_{\{1,0\}\{1,0\}}\Big)^2\Big)\Big) + \\
&(p\cdot u) \Big(p^2\, g^{\mu\gamma}\, (p\cdot u) \Big(8\, (2\, D^6 - 26\, D^5 + 95\, D^4 - 41\, D^3 - 244\, D^2 + 76\, D + 240)\, \mathbf{J}^{(D)}_{\{1,0\}\{1,0\}\{1,0\}} - \\
&3\, (6\, D^5 - 83\, D^4 + 364\, D^3 - 412\, D^2 - 640\, D + 960)\, p^2 \Big(\mathbf{B}^{(D)}_{\{1,0\}\{1,0\}}\Big)^2\Big) + \\
&p^\mu \Big(2\, p^2\, u^\gamma \Big(9\, (3\, D^3 - 34\, D^2 + 112\, D - 96)\, p^2 \Big(\mathbf{B}^{(D)}_{\{1,0\}\{1,0\}}\Big)^2 - \\
&2\, (4\, D^6 - 41\, D^5 + 140\, D^4 - 189\, D^3 + 18\, D^2 + 344\, D - 384)\, \mathbf{J}^{(D)}_{\{1,0\}\{1,0\}\{1,0\}}\Big) + \\
&p^\gamma\, (p\cdot u) \Big(3\, (6\, D^5 - 83\, D^4 + 346\, D^3 - 208\, D^2 - 1312\, D + 1536)\, p^2 \Big(\mathbf{B}^{(D)}_{\{1,0\}\{1,0\}}\Big)^2 + \\
&4\, (2\, D^7 - 50\, D^6 + 443\, D^5 - 1706\, D^4 + 2531\, D^3 + 196\, D^2 - 2880\, D + 1152) \\
&\mathbf{J}^{(D)}_{\{1,0\}\{1,0\}\{1,0\}}\Big)\Big)\Big)\Big)\Big) \Big/ \Big(6\, (D-6)\, (D-4)^2\, (D-1)\, (D+1)\, (3\, D-4)\, p^4\Big)\Big)
\end{aligned}
$$

$$
\begin{aligned}
(4\pi)^D\, \Pi^{\gamma\mu}_{15\,\mathrm{LV}}(p) = &-\frac{1}{3\,(D-6)\,(D-4)\,(D-1)\,(3\,D-4)\,p^4}\, 2\, i\, (D^2 - 6\, D + 4)\, e^4\, Q_1\, \mathbf{J}^{(D)}_{\{1,0\}\{1,0\}\{1,0\}} \\
&\big((D-3)\,(p\cdot u)\,\big((D-4)\,p^\mu\,\big((D+4)\,p^\gamma\,(p\cdot u) - 2\,p^2\,u^\gamma\big) - 4\,(D-2)\,p^2\,g^{\mu\gamma}\,(p\cdot u)\big) - \\
&2\,p^2\,u^\mu\,\big((D^2 - 7\,D + 12)\,p^\gamma\,(p\cdot u) - D\,p^2\,u^\gamma\big)\big)
\end{aligned}
$$

$$
\begin{aligned}
(4\pi)^D\, \Pi^{\gamma\mu}_{16\,\mathrm{LV}}(p) = &-\frac{1}{3\,(D-6)\,(D-4)\,(D-1)\,(3\,D-4)\,p^4}\, 2\, i\, (D^2 - 6\, D + 4)\, e^4\, Q_1\, \mathbf{J}^{(D)}_{\{1,0\}\{1,0\}\{1,0\}} \\
&\big((D-3)\,(p\cdot u)\,\big((D-4)\,p^\mu\,\big((D+4)\,p^\gamma\,(p\cdot u) - 2\,p^2\,u^\gamma\big) - 4\,(D-2)\,p^2\,g^{\mu\gamma}\,(p\cdot u)\big) - \\
&2\,p^2\,u^\mu\,\big((D^2 - 7\,D + 12)\,p^\gamma\,(p\cdot u) - D\,p^2\,u^\gamma\big)\big)
\end{aligned}
$$

$$
\begin{aligned}
(4\pi)^D\, \Pi^{\gamma\mu}_{17\,\mathrm{LV}}(p) = &-\Big(\Big(2\, i\, (D-2)\, e^4\, Q_2\, \mathbf{J}^{(D)}_{\{1,0\}\{1,0\}\{1,0\}} \\
&\big((D-3)\,(p\cdot u)\,\big((D-4)\,p^\mu\,\big((D+4)\,p^\gamma\,(p\cdot u) - 2\,p^2\,u^\gamma\big) - 4\,(D-2)\,p^2\,g^{\mu\gamma}\,(p\cdot u)\big) - \\
&2\,p^2\,u^\mu\,\big((D^2 - 7\,D + 12)\,p^\gamma\,(p\cdot u) - D\,p^2\,u^\gamma\big)\big)\Big) \Big/ \Big(3\,(D-6)\,(D-4)\,(3\,D-4)\,p^4\Big)\Big)
\end{aligned}
$$

$$
(4\pi)^D\, \Pi^{\gamma\mu}_{18\,\mathrm{LV}}(p) = -\Big(\Big(2\, i\, (D-2)\, e^4\, Q_2\, \mathbf{J}^{(D)}_{\{1,0\}\{1,0\}\{1,0\}}
$$

$$\Big((D-3)\,(p\cdot u)\,\big((D-4)\,p^{\mu}\,\big((D+4)\,p^{\gamma}\,(p\cdot u)-2\,p^2\,u^{\gamma}\big)-4\,(D-2)\,p^2\,g^{\mu\,\gamma}\,(p\cdot u)\big)-$$
$$2\,p^2\,u^{\mu}\,\big(\big(D^2-7\,D+12\big)\,p^{\gamma}\,(p\cdot u)-D\,p^2\,u^{\gamma}\big)\Big)\Big)\Big/\big(3\,(D-6)\,(D-4)\,(3\,D-4)\,p^4\big)\Big)$$

$$(4\,\pi)^D\,\Pi^{\gamma\mu}_{19\,\mathrm{LV}}(p)=-\frac{2\,i\,\mathrm{e}^4\,Q_1\,u^{\gamma}\,\big(p^2\,u^{\mu}-(D-3)\,p^{\mu}\,(p\cdot u)\big)\,\mathbf{J}^{(D)}_{\{1,0\}\,\{1,0\}\,\{1,0\}}}{(D-4)\,p^2}$$

$$(4\,\pi)^D\,\Pi^{\gamma\mu}_{20\,\mathrm{LV}}(p)=-\frac{2\,i\,\mathrm{e}^4\,Q_1\,u^{\gamma}\,\big(p^2\,u^{\mu}-(D-3)\,p^{\mu}\,(p\cdot u)\big)\,\mathbf{J}^{(D)}_{\{1,0\}\,\{1,0\}\,\{1,0\}}}{(D-4)\,p^2}$$

$$(4\,\pi)^D\,\Pi^{\gamma\mu}_{25\,\mathrm{LV}}(p)=-\frac{2\,i\,\mathrm{e}^4\,Q_1\,u^{\gamma}\,\big(p^2\,u^{\mu}-(D-3)\,p^{\mu}\,(p\cdot u)\big)\,\mathbf{J}^{(D)}_{\{1,0\}\,\{1,0\}\,\{1,0\}}}{(D-4)\,p^2}$$

$$(4\,\pi)^D\,\Pi^{\gamma\mu}_{26\,\mathrm{LV}}(p)=-\frac{2\,i\,\mathrm{e}^4\,Q_1\,u^{\gamma}\,\big(p^2\,u^{\mu}-(D-3)\,p^{\mu}\,(p\cdot u)\big)\,\mathbf{J}^{(D)}_{\{1,0\}\,\{1,0\}\,\{1,0\}}}{(D-4)\,p^2}$$

$$(4\,\pi)^D\,\Pi^{\gamma\mu}_{29\,\mathrm{LV}}(p)=-\frac{4\,i\,(D-3)\,\mathrm{e}^4\,Q_1\,g^{\mu\,\gamma}\,(\,p\cdot u\,)^2\,\mathbf{J}^{(D)}_{\{1,0\}\,\{1,0\}\,\{1,0\}}}{3\,p^2}$$

$$(4\,\pi)^D\,\Pi^{\gamma\mu}_{30\,\mathrm{LV}}(p)=-\frac{4\,i\,(D-3)\,\mathrm{e}^4\,Q_1\,g^{\mu\,\gamma}\,(\,p\cdot u\,)^2\,\mathbf{J}^{(D)}_{\{1,0\}\,\{1,0\}\,\{1,0\}}}{3\,p^2}$$

$$(4\,\pi)^D\,\Pi^{\gamma\mu}_{31\,\mathrm{LV}}(p)=-\frac{2\,i\,\mathrm{e}^4\,Q_2\,\mathbf{J}^{(D)}_{\{1,0\}\,\{1,0\}\,\{1,0\}}\,\big((D-3)\,(p\cdot u)\,(p^{\mu}\,u^{\gamma}-g^{\mu\,\gamma}\,(p\cdot u))+u^{\mu}\,\big((D-3)\,p^{\gamma}\,(p\cdot u)+p^2\,u^{\gamma}\big)\big)}{3\,p^2}$$

$$(4\,\pi)^D\,\Pi^{\gamma\mu}_{32\,\mathrm{LV}}(p)=-\frac{2\,i\,\mathrm{e}^4\,Q_1\,u^{\mu}\,\big(p^2\,u^{\gamma}-(D-3)\,p^{\gamma}\,(p\cdot u)\big)\,\mathbf{J}^{(D)}_{\{1,0\}\,\{1,0\}\,\{1,0\}}}{(D-4)\,p^2}$$

$$(4\,\pi)^D\,\Pi^{\gamma\mu}_{33\,\mathrm{LV}}(p)=-\frac{2\,i\,\mathrm{e}^4\,Q_1\,u^{\mu}\,\big(p^2\,u^{\gamma}-(D-3)\,p^{\gamma}\,(p\cdot u)\big)\,\mathbf{J}^{(D)}_{\{1,0\}\,\{1,0\}\,\{1,0\}}}{(D-4)\,p^2}$$

$$(4\,\pi)^D\,\Pi^{\gamma\mu}_{34\,\mathrm{LV}}(p)=-\frac{2\,i\,\mathrm{e}^4\,Q_1\,u^{\gamma}\,\big(p^2\,u^{\mu}-(D-3)\,p^{\mu}\,(p\cdot u)\big)\,\mathbf{J}^{(D)}_{\{1,0\}\,\{1,0\}\,\{1,0\}}}{(D-4)\,p^2}$$

$$(4\,\pi)^D\,\Pi^{\gamma\mu}_{35\,\mathrm{LV}}(p)=-\frac{2\,i\,\mathrm{e}^4\,Q_1\,u^{\gamma}\,\big(p^2\,u^{\mu}-(D-3)\,p^{\mu}\,(p\cdot u)\big)\,\mathbf{J}^{(D)}_{\{1,0\}\,\{1,0\}\,\{1,0\}}}{(D-4)\,p^2}$$

$$(4\,\pi)^D\,\Pi^{\gamma\mu}_{46\,\mathrm{LV}}(p)=-\frac{2\,i\,\mathrm{e}^4\,Q_1\,u^{\mu}\,\big(p^2\,u^{\gamma}-(D-3)\,p^{\gamma}\,(p\cdot u)\big)\,\mathbf{J}^{(D)}_{\{1,0\}\,\{1,0\}\,\{1,0\}}}{(D-4)\,p^2}$$

$$(4\,\pi)^D\,\Pi^{\gamma\mu}_{47\,\mathrm{LV}}(p)=-\frac{2\,i\,\mathrm{e}^4\,Q_1\,u^{\mu}\,\big(p^2\,u^{\gamma}-(D-3)\,p^{\gamma}\,(p\cdot u)\big)\,\mathbf{J}^{(D)}_{\{1,0\}\,\{1,0\}\,\{1,0\}}}{(D-4)\,p^2}$$

$$(4\,\pi)^D\,\Pi^{\gamma\mu}_{48\,\mathrm{LV}}(p)=-\frac{2\,i\,\mathrm{e}^4\,Q_1\,u^{\mu}\,\big(p^2\,u^{\gamma}-(D-3)\,p^{\gamma}\,(p\cdot u)\big)\,\mathbf{J}^{(D)}_{\{1,0\}\,\{1,0\}\,\{1,0\}}}{(D-4)\,p^2}$$

$$(4\,\pi)^D\,\Pi^{\gamma\mu}_{49\,\mathrm{LV}}(p)=-\frac{2\,i\,\mathrm{e}^4\,Q_1\,u^{\mu}\,\big(p^2\,u^{\gamma}-(D-3)\,p^{\gamma}\,(p\cdot u)\big)\,\mathbf{J}^{(D)}_{\{1,0\}\,\{1,0\}\,\{1,0\}}}{(D-4)\,p^2}$$

$$(4\,\pi)^D\,\Pi^{\gamma\mu}_{70\,\mathrm{LV}}(p)=\frac{1}{(D-4)\,(3\,D-4)\,p^4}$$

$$2\, i\, e^4\, Q_1\, \mathbf{J}^{(D)}_{\{1,0\}\{1,0\}\{1,0\}} \left((D-3)\,(p\cdot u)\left((D-4)\,p^\mu\left((D-4)\,p^\gamma\,(p\cdot u)+p^2\,u^\gamma\right)-D\,p^2\,g^{\mu\,\gamma}\,(p\cdot u)\right)+ \right.$$
$$\left. 2\,(D-2)\,p^2\,u^\mu\left(2\,(D-3)\,p^\gamma\,(p\cdot u)+p^2\,u^\gamma\right)\right)$$

$$(4\,\pi)^D\,\Pi^{\gamma\mu}_{71\,\mathrm{LV}}(p) = \frac{1}{(D-4)\,(3\,D-4)\,p^4} 2\, i\, e^4\, Q_1\, \mathbf{J}^{(D)}_{\{1,0\}\{1,0\}\{1,0\}}$$
$$\left((D-3)\,(p\cdot u)\left((D-4)\,p^\mu\left((D-4)\,p^\gamma\,(p\cdot u)+p^2\,u^\gamma\right)-D\,p^2\,g^{\mu\,\gamma}\,(p\cdot u)\right)+ \right.$$
$$\left. 2\,(D-2)\,p^2\,u^\mu\left(2\,(D-3)\,p^\gamma\,(p\cdot u)+p^2\,u^\gamma\right)\right)$$

$$(4\,\pi)^D\,\Pi^{\gamma\mu}_{72\,\mathrm{LV}}(p) = -\frac{1}{(D-6)\,(D-4)\,(3\,D-4)\,p^4} 4\, i\, e^4\, Q_1\, \mathbf{J}^{(D)}_{\{1,0\}\{1,0\}\{1,0\}} \left(p^2\,u^\mu\left(D\,p^2\,u^\gamma-4\left(D^2-5\,D+6\right)p^\gamma\,(p\cdot u)\right)+ \right.$$
$$\left. (D-3)\,(p\cdot u)\left((D-4)\,p^\mu\left(2\,D\,p^\gamma\,(p\cdot u)-p^2\,u^\gamma\right)-2\,(D-2)\,p^2\,g^{\mu\,\gamma}\,(p\cdot u)\right)\right)$$

$$(4\,\pi)^D\,\Pi^{\gamma\mu}_{73\,\mathrm{LV}}(p) = -\frac{1}{(D-6)\,(D-4)\,(3\,D-4)\,p^4} 4\, i\, e^4\, Q_1\, \mathbf{J}^{(D)}_{\{1,0\}\{1,0\}\{1,0\}} \left(p^2\,u^\mu\left(D\,p^2\,u^\gamma-4\left(D^2-5\,D+6\right)p^\gamma\,(p\cdot u)\right)+ \right.$$
$$\left. (D-3)\,(p\cdot u)\left((D-4)\,p^\mu\left(2\,D\,p^\gamma\,(p\cdot u)-p^2\,u^\gamma\right)-2\,(D-2)\,p^2\,g^{\mu\,\gamma}\,(p\cdot u)\right)\right)$$

$$(4\,\pi)^D\,\Pi^{\gamma\mu}_{74\,\mathrm{LV}}(p) = -\left(\left(i\,(9\,D-8)\,e^4\,Q_1\,\mathbf{J}^{(D)}_{\{1,0\}\{1,0\}\{1,0\}}\right.\right.$$
$$\left((D-3)\,(p\cdot u)\left((D-4)\,p^\mu\left((D+4)\,p^\gamma\,(p\cdot u)-2\,p^2\,u^\gamma\right)-4\,(D-2)\,p^2\,g^{\mu\,\gamma}\,(p\cdot u)\right)-\right.$$
$$\left.\left.\left. 2\,p^2\,u^\mu\left(\left(D^2-7\,D+12\right)p^\gamma\,(p\cdot u)-D\,p^2\,u^\gamma\right)\right)\right)\Big/\left(3\,(D-6)\,(D-4)\,(D-1)\,(3\,D-4)\,p^4\right)\right)$$

$$(4\,\pi)^D\,\Pi^{\gamma\mu}_{75\,\mathrm{LV}}(p) = -\left(\left(i\,(9\,D-8)\,e^4\,Q_1\,\mathbf{J}^{(D)}_{\{1,0\}\{1,0\}\{1,0\}}\right.\right.$$
$$\left((D-3)\,(p\cdot u)\left((D-4)\,p^\mu\left((D+4)\,p^\gamma\,(p\cdot u)-2\,p^2\,u^\gamma\right)-4\,(D-2)\,p^2\,g^{\mu\,\gamma}\,(p\cdot u)\right)-\right.$$
$$\left.\left.\left. 2\,p^2\,u^\mu\left(\left(D^2-7\,D+12\right)p^\gamma\,(p\cdot u)-D\,p^2\,u^\gamma\right)\right)\right)\Big/\left(3\,(D-6)\,(D-4)\,(D-1)\,(3\,D-4)\,p^4\right)\right)$$

$$(4\,\pi)^D\,\Pi^{\gamma\mu}_{76\,\mathrm{LV}}(p) = -\left(\left(i\,(9\,D-8)\,e^4\,Q_1\,\mathbf{J}^{(D)}_{\{1,0\}\{1,0\}\{1,0\}}\right.\right.$$
$$\left((D-3)\,(p\cdot u)\left((D-4)\,p^\mu\left((D+4)\,p^\gamma\,(p\cdot u)-2\,p^2\,u^\gamma\right)-4\,(D-2)\,p^2\,g^{\mu\,\gamma}\,(p\cdot u)\right)-\right.$$
$$\left.\left.\left. 2\,p^2\,u^\mu\left(\left(D^2-7\,D+12\right)p^\gamma\,(p\cdot u)-D\,p^2\,u^\gamma\right)\right)\right)\Big/\left(3\,(D-6)\,(D-4)\,(D-1)\,(3\,D-4)\,p^4\right)\right)$$

$$(4\,\pi)^D\,\Pi^{\gamma\mu}_{77\,\mathrm{LV}}(p) = -\left(\left(i\,(9\,D-8)\,e^4\,Q_1\,\mathbf{J}^{(D)}_{\{1,0\}\{1,0\}\{1,0\}}\right.\right.$$
$$\left((D-3)\,(p\cdot u)\left((D-4)\,p^\mu\left((D+4)\,p^\gamma\,(p\cdot u)-2\,p^2\,u^\gamma\right)-4\,(D-2)\,p^2\,g^{\mu\,\gamma}\,(p\cdot u)\right)-\right.$$
$$\left.\left.\left. 2\,p^2\,u^\mu\left(\left(D^2-7\,D+12\right)p^\gamma\,(p\cdot u)-D\,p^2\,u^\gamma\right)\right)\right)\Big/\left(3\,(D-6)\,(D-4)\,(D-1)\,(3\,D-4)\,p^4\right)\right)$$

$$(4\,\pi)^D\,\Pi^{\gamma\mu}_{78\,\mathrm{LV}}(p) = -\frac{2\,i\,e^4\,Q_1\,u^\gamma\left(D\,p^\mu\,(p\cdot u)-4\,p^2\,u^\mu\right)\mathbf{J}^{(D)}_{\{1,0\}\{1,0\}\{1,0\}}}{3\,(D-4)\,p^2}$$

$$(4\,\pi)^D\,\Pi^{\gamma\mu}_{79\,\mathrm{LV}}(p) = -\frac{2\,i\,e^4\,Q_1\,u^\gamma\left(D\,p^\mu\,(p\cdot u)-4\,p^2\,u^\mu\right)\mathbf{J}^{(D)}_{\{1,0\}\{1,0\}\{1,0\}}}{3\,(D-4)\,p^2}$$

$$(4\,\pi)^D\,\Pi^{\gamma\mu}_{80\,\mathrm{LV}}(p) = \frac{1}{3\,(D-4)^2\,(D-1)\,p^2}$$
$$4\,i\,e^4\,Q_1\,u^\gamma\left(p^2\,u^\mu\left(3\,(D-4)\,p^2\left(\mathbf{B}^{(D)}_{\{1,0\}\{1,0\}}\right)^2-4\left(D^2-2\,D-2\right)\mathbf{J}^{(D)}_{\{1,0\}\{1,0\}\{1,0\}}\right)+\right.$$
$$\left. p^\mu\,(p\cdot u)\left(-3\,(D-4)\,p^2\left(\mathbf{B}^{(D)}_{\{1,0\}\{1,0\}}\right)^2-2\left(D^3-11\,D^2+28\,D-12\right)\mathbf{J}^{(D)}_{\{1,0\}\{1,0\}\{1,0\}}\right)\right)$$

$$(4\,\pi)^D\,\Pi^{\gamma\mu}_{81\,\mathrm{LV}}(p) = -\frac{1}{(D-6)\,(D-4)\,(3\,D-4)\,p^4} 4\, i\, e^4\, Q_1\, \mathbf{J}^{(D)}_{\{1,0\}\{1,0\}\{1,0\}} \left(p^2\,u^\mu\left(D\,p^2\,u^\gamma-\left(D^2-7\,D+12\right)p^\gamma\,(p\cdot u)\right)+ \right.$$
$$\left. 2\,(D-3)\,(p\cdot u)\left(p^\mu\left((D-4)\,D\,p^\gamma\,(p\cdot u)-2\,(D-2)\,p^2\,u^\gamma\right)-(D-2)\,p^2\,g^{\mu\,\gamma}\,(p\cdot u)\right)\right)$$

$$(4\,\pi)^D\,\Pi^{\gamma\mu}_{82\,\mathrm{LV}}(p) = -\frac{1}{(D-6)\,(D-4)\,(3\,D-4)\,p^4} 4\, i\, e^4\, Q_1\, \mathbf{J}^{(D)}_{\{1,0\}\{1,0\}\{1,0\}} \left(p^2\,u^\mu\left(D\,p^2\,u^\gamma-\left(D^2-7\,D+12\right)p^\gamma\,(p\cdot u)\right)+ \right.$$
$$\left. 2\,(D-3)\,(p\cdot u)\left(p^\mu\left((D-4)\,D\,p^\gamma\,(p\cdot u)-2\,(D-2)\,p^2\,u^\gamma\right)-(D-2)\,p^2\,g^{\mu\,\gamma}\,(p\cdot u)\right)\right)$$

$$(4\pi)^D\,\Pi^{\gamma\mu}_{83\,\mathrm{LV}}(p) = \frac{1}{(D-4)(3D-4)p^4} 2\,i\,e^4\,Q_1\,\mathbf{J}^{(D)}_{\{1,0\}\{1,0\}\{1,0\}}\left(p^2 u^\mu\left(\left(D^2-7D+12\right)p^\gamma (p\cdot u)+2(D-2)p^2 u^\gamma\right)+\right.$$
$$\left.(D-3)(p\cdot u)\left(p^\mu\left(4(D-2)p^2 u^\gamma+(D-4)^2 p^\gamma (p\cdot u)\right)-D\,p^2 g^{\mu\gamma}(p\cdot u)\right)\right)$$

$$(4\pi)^D\,\Pi^{\gamma\mu}_{84\,\mathrm{LV}}(p) = \frac{1}{(D-4)(3D-4)p^4} 2\,i\,e^4\,Q_1\,\mathbf{J}^{(D)}_{\{1,0\}\{1,0\}\{1,0\}}\left(p^2 u^\mu\left(\left(D^2-7D+12\right)p^\gamma (p\cdot u)+2(D-2)p^2 u^\gamma\right)+\right.$$
$$\left.(D-3)(p\cdot u)\left(p^\mu\left(4(D-2)p^2 u^\gamma+(D-4)^2 p^\gamma (p\cdot u)\right)-D\,p^2 g^{\mu\gamma}(p\cdot u)\right)\right)$$

$$(4\pi)^D\,\Pi^{\gamma\mu}_{89\,\mathrm{LV}}(p) = -\frac{2\,i\,e^4\,Q_1\,u^\mu\left(D\,p^\gamma (p\cdot u)-4p^2 u^\gamma\right)\mathbf{J}^{(D)}_{\{1,0\}\{1,0\}\{1,0\}}}{3(D-4)p^2}$$

$$(4\pi)^D\,\Pi^{\gamma\mu}_{90\,\mathrm{LV}}(p) = -\frac{2\,i\,e^4\,Q_1\,u^\mu\left(D\,p^\gamma (p\cdot u)-4p^2 u^\gamma\right)\mathbf{J}^{(D)}_{\{1,0\}\{1,0\}\{1,0\}}}{3(D-4)p^2}$$

$$(4\pi)^D\,\Pi^{\gamma\mu}_{91\,\mathrm{LV}}(p) = \frac{1}{3(D-4)^2(D-1)p^2}$$
$$4\,i\,e^4\,Q_1\,u^\mu\left(p^2 u^\gamma\left(3(D-4)p^2\left(\mathbf{B}^{(D)}_{\{1,0\}\{1,0\}}\right)^2-4\left(D^2-2D-2\right)\mathbf{J}^{(D)}_{\{1,0\}\{1,0\}\{1,0\}}\right)+\right.$$
$$\left.p^\gamma (p\cdot u)\left(-3(D-4)p^2\left(\mathbf{B}^{(D)}_{\{1,0\}\{1,0\}}\right)^2-2\left(D^3-11D^2+28D-12\right)\mathbf{J}^{(D)}_{\{1,0\}\{1,0\}\{1,0\}}\right)\right)$$

$$(4\pi)^D\,\Pi^{\gamma\mu}_{92\,\mathrm{LV}}(p) =$$
$$-\left(\left(i\,e^4\,Q_2\left((p\cdot u)\left((D-1)p^2 g^{\mu\gamma}(p\cdot u)\left(4D^2\left(D^2-4D+3\right)\mathbf{J}^{(D)}_{\{1,0\}\{1,0\}\{1,0\}}-3\left(3D^2-16D+16\right)p^2\left(\mathbf{B}^{(D)}_{\{1,0\}\{1,0\}}\right)^2\right)+\right.\right.\right.$$
$$p^\mu\left((D-3)p^2 u^\gamma\left(2\left(D^4-D^3-6D^2-4D+16\right)\mathbf{J}^{(D)}_{\{1,0\}\{1,0\}\{1,0\}}-\right.\right.$$
$$\left.3\left(3D^2-16D+16\right)p^2\left(\mathbf{B}^{(D)}_{\{1,0\}\{1,0\}}\right)^2\right)+2(D-2)p^\gamma (p\cdot u)\left(3\left(3D^2-16D+16\right)\right.$$
$$\left.\left.\left.p^2\left(\mathbf{B}^{(D)}_{\{1,0\}\{1,0\}}\right)^2+D\left(D^4-12D^3+33D^2-10D-24\right)\mathbf{J}^{(D)}_{\{1,0\}\{1,0\}\{1,0\}}\right)\right)\right)+$$
$$p^2 u^\mu\left(p^2 u^\gamma\left(3\left(3D^3-25D^2+64D-48\right)p^2\left(\mathbf{B}^{(D)}_{\{1,0\}\{1,0\}}\right)^2-4\left(2D^4-11D^3+11D^2+\right.\right.\right.$$
$$\left.\left.24D-32\right)\mathbf{J}^{(D)}_{\{1,0\}\{1,0\}\{1,0\}}\right)+(D-3)p^\gamma (p\cdot u)$$
$$\left.\left.\left.\left.\left(2\left(D^4-D^3-6D^2-4D+16\right)\mathbf{J}^{(D)}_{\{1,0\}\{1,0\}\{1,0\}}-3\left(3D^2-16D+16\right)p^2\left(\mathbf{B}^{(D)}_{\{1,0\}\{1,0\}}\right)^2\right)\right)\right)\right)\right)\Big/$$
$$\left.\left(3(D-4)(D-2)(D-1)(D+1)(3D-4)p^4\right)\right)$$

$$(4\pi)^D\,\Pi^{\gamma\mu}_{93\,\mathrm{LV}}(p) = -\frac{1}{3(D-4)(3D-4)p^4}\,2\,i\,e^4\,Q_1\,\mathbf{J}^{(D)}_{\{1,0\}\{1,0\}\{1,0\}}$$
$$\left((p\cdot u)\left((D-4)p^\mu\left(\left(D^2-6D+24\right)p^\gamma (p\cdot u)+4(D-3)p^2 u^\gamma\right)-4(D-3)D\,p^2 g^{\mu\gamma}(p\cdot u)\right)+\right.$$
$$\left.4p^2 u^\mu\left(\left(D^2-7D+12\right)p^\gamma (p\cdot u)+2(D-2)p^2 u^\gamma\right)\right)$$

$$(4\pi)^D\,\Pi^{\gamma\mu}_{94\,\mathrm{LV}}(p) = -\frac{1}{3(D-4)(3D-4)p^4}\,2\,i\,e^4\,Q_1\,\mathbf{J}^{(D)}_{\{1,0\}\{1,0\}\{1,0\}}$$
$$\left((p\cdot u)\left((D-4)p^\mu\left(\left(D^2-6D+24\right)p^\gamma (p\cdot u)+4(D-3)p^2 u^\gamma\right)-4(D-3)D\,p^2 g^{\mu\gamma}(p\cdot u)\right)+\right.$$
$$\left.4p^2 u^\mu\left(\left(D^2-7D+12\right)p^\gamma (p\cdot u)+2(D-2)p^2 u^\gamma\right)\right)$$

$$(4\pi)^D\,\Pi^{\gamma\mu}_{95\,\mathrm{LV}}(p) = \left(8\,i\,e^4\,Q_1\,\mathbf{J}^{(D)}_{\{1,0\}\{1,0\}\{1,0\}}\right.$$
$$\left((D-3)(p\cdot u)\left((D-4)p^\mu\left((D+4)p^\gamma (p\cdot u)-2p^2 u^\gamma\right)-4(D-2)p^2 g^{\mu\gamma}(p\cdot u)\right)-\right.$$
$$\left.\left.2p^2 u^\mu\left(\left(D^2-7D+12\right)p^\gamma (p\cdot u)-D\,p^2 u^\gamma\right)\right)\right)\Big/\left(3(D-6)(D-4)(3D-4)p^4\right)$$

$$(4\pi)^D\,\Pi^{\gamma\mu}_{96\,\mathrm{LV}}(p) = \left(8\,i\,e^4\,Q_1\,\mathbf{J}^{(D)}_{\{1,0\}\{1,0\}\{1,0\}}\right.$$
$$\left((D-3)(p\cdot u)\left((D-4)p^\mu\left((D+4)p^\gamma (p\cdot u)-2p^2 u^\gamma\right)-4(D-2)p^2 g^{\mu\gamma}(p\cdot u)\right)-\right.$$

$$2\,p^2\,u^\mu\left((D^2-7\,D+12)\,p^\gamma\,(p\cdot u)-D\,p^2\,u^\gamma\right)\Big)\Big)\Big/\left(3\,(D-6)\,(D-4)\,(3\,D-4)\,p^4\right)$$

$$(4\,\pi)^D\,\Pi^{\gamma\mu}_{97\,\mathrm{LV}}(p)=\Big(8\,i\,e^4\,Q_1\,\mathbf{J}^{(D)}_{\{1,0\}\{1,0\}\{1,0\}}\Big((D-3)\,(p\cdot u)\left((D-4)\,p^\mu\left((D+4)\,p^\gamma\,(p\cdot u)-2\,p^2\,u^\gamma\right)-4\,(D-2)\,p^2\,g^{\mu\,\gamma}\,(p\cdot u)\right)-2\,p^2\,u^\mu\left((D^2-7\,D+12)\,p^\gamma\,(p\cdot u)-D\,p^2\,u^\gamma\right)\Big)\Big)\Big/\left(3\,(D-6)\,(D-4)\,(3\,D-4)\,p^4\right)$$

$$(4\,\pi)^D\,\Pi^{\gamma\mu}_{98\,\mathrm{LV}}(p)=\Big(8\,i\,e^4\,Q_1\,\mathbf{J}^{(D)}_{\{1,0\}\{1,0\}\{1,0\}}\Big((D-3)\,(p\cdot u)\left((D-4)\,p^\mu\left((D+4)\,p^\gamma\,(p\cdot u)-2\,p^2\,u^\gamma\right)-4\,(D-2)\,p^2\,g^{\mu\,\gamma}\,(p\cdot u)\right)-2\,p^2\,u^\mu\left((D^2-7\,D+12)\,p^\gamma\,(p\cdot u)-D\,p^2\,u^\gamma\right)\Big)\Big)\Big/\left(3\,(D-6)\,(D-4)\,(3\,D-4)\,p^4\right)$$

$$(4\,\pi)^D\,\Pi^{\gamma\mu}_{107\,\mathrm{LV}}(p)=-4\,i\,e^4\,Q_1\,u^\gamma\,u^\mu\,\mathbf{J}^{(D)}_{\{1,0\}\{1,0\}\{1,0\}}$$

$$(4\,\pi)^D\,\Pi^{\gamma\mu}_{108\,\mathrm{LV}}(p)=-4\,i\,e^4\,Q_1\,u^\gamma\,u^\mu\,\mathbf{J}^{(D)}_{\{1,0\}\{1,0\}\{1,0\}}$$

where we have omitted the vanishing results.

By expanding the aforementioned expressions around $D = 4 - 2\epsilon$ and incorporating all relevant contributions, we arrive at the following result

$$\begin{aligned}-i\Pi^{\mu\gamma}_{2l-LV}(p) &= (p\cdot u)\left[\eta^{\mu\gamma}(p\cdot u) - p^\mu u^\gamma + u^\mu\left(p^2u^\gamma - p^\gamma(p\cdot u)\right)\right] \\ &\times\left(-\frac{e^4(2Q_1+Q_2)}{1536\pi^4\epsilon^2} - \frac{e^4(38Q_1+Q_2)}{4608\pi^4\epsilon}\right) + \text{finite.}\end{aligned} \quad (3)$$

## II. CALCULATION OF THE TWO-LOOP SCALAR FIELD SELF-ENERGY DIAGRAMS

Let us now proceed with the computation of the two-loop scalar self-energy, which is represented by the diagrams in Figs. 5 to 8. The conventional amplitude is obtained from the Feynman diagrams shown in Figs. 5 and 6, while the LV contributions are represented by Figs. 7 and 8.

The expression for the scalar field self-energy can be written as

$$\Sigma_{2l}(p) = \sum_i \int \frac{d^Dk_1}{(2\pi)^D}\frac{d^Dk_2}{(2\pi)^D}\tilde{\Sigma}_i(p), \quad (4)$$

where $\tilde{\Sigma}_i(p)$ corresponds to the individual contributions. Considering the ordinary two-loop scalar field self-energy depicted in Fig. 5, the expressions for the corresponding contributions are as follows:

$$\tilde{\Sigma}_1(p) = -\frac{i\, e^2\, \lambda \left(-4\,(k_1\cdot p) + 4\,p^2 + k_1{}^2\right)}{k_1{}^2.k_2{}^2.(\,k_1 - p\,)^{2^2}}$$

$$\tilde{\Sigma}_2(p) = -\frac{2\,i\, e^4 \left(2\,(k_1\cdot p) + p^2 + k_1{}^2\right)}{k_1{}^2.k_2{}^2.(\,k_1 - p\,)^{2^2}}$$

$$\tilde{\Sigma}_3(p) = -\frac{i\,D\, e^4 \left(-4\,(k_1\cdot p) + 4\,p^2 + k_1{}^2\right)}{k_1{}^2.k_2{}^2.(\,k_1 - p\,)^{2^2}}$$

$$\tilde{\Sigma}_4(p) = \frac{i\, e^2\, \lambda \left(2\,(k_1\cdot p + 2\,(k_2\cdot p) + k_1\cdot k_2) + k_1{}^2\right)}{k_2{}^2.k_1{}^2.(\,k_1 + p\,)^2.(\,k_1 + k_2\,)^2}$$

$$\tilde{\Sigma}_4(p) = -\frac{2\,i\, e^4 \left(-k_1\cdot p + k_2\cdot p - k_1\cdot k_2 + k_1{}^2\right)}{k_2{}^2.k_1{}^2.(\,k_1 + p\,)^2.(\,k_1 + k_2\,)^2}$$

$$\tilde{\Sigma}_6(p) = -\frac{i\, e^2\, \lambda \left(-2\,(k_1\cdot p) - 4\,(k_2\cdot p) + 2\,(k_1\cdot k_2) + k_1{}^2\right)}{k_2{}^2.k_1{}^2.(\,k_1 - p\,)^2.(\,k_1 + k_2\,)^2}$$

$$\tilde{\Sigma}_7(p) = -\frac{2\,i\, e^4 \left(k_1\cdot p - k_2\cdot p - k_1\cdot k_2 + k_1{}^2\right)}{k_2{}^2.k_1{}^2.(\,k_1 - p\,)^2.(\,k_1 + k_2\,)^2}$$

$$\tilde{\Sigma}_8(p) = \frac{i\, e^4 \left(-4\,(k_1\cdot p) - 2\,(k_2\cdot p) + 2\,(k_1\cdot k_2) + k_2{}^2\right)\left(-2\,(k_1\cdot p) - 2\,(k_2\cdot p) + p^2 + 2\,(k_1\cdot k_2) + k_1{}^2\right)}{k_2{}^2.k_1{}^2.(\,k_1 + p\,)^2.(\,k_2 - p\,)^2.(\,k_1 + k_2\,)^2}$$

$$\tilde{\Sigma}_9(p) = \frac{i\, e^4 \left(2\,(k_2\cdot p) + p^2 + 2\,(k_1\cdot k_2) - k_1{}^2\right)^2}{k_2{}^2.k_1{}^2.(\,k_1 - p\,)^{2^2}.(\,-k_1 + k_2 + p\,)^2}$$

$$\tilde{\Sigma}_{10}(p) = \frac{i\, e^4 \left(-4\,(k_1\cdot p) + 4\,p^2 + k_1{}^2\right)\left(-2\,(k_1\cdot p) - 2\,(k_2\cdot p) + p^2 + 2\,(k_1\cdot k_2) + k_1{}^2 + k_2{}^2\right)}{k_2{}^2.k_1{}^2.(\,k_1 - p\,)^{2^2}.(\,-k_1 + k_2 + p\,)^2}$$

$$\tilde{\Sigma}_{11}(p) = \frac{i\,\lambda^2}{\left(k_1{}^2\right)^2.k_2{}^2}$$

$$\tilde{\Sigma}_{12}(p) = \frac{i\,D\, e^2\,\lambda}{\left(k_1{}^2\right)^2.k_2{}^2}$$

$$\tilde{\Sigma}_{13}(p) = \frac{2\,i\,D\, e^4}{\left(k_1{}^2\right)^2.k_2{}^2}$$

$$\tilde{\Sigma}_{14}(p) = \frac{2\,i\, e^4 \left(-k_1\cdot p + k_2\cdot p - p^2 + k_1\cdot k_2\right)}{k_2{}^2.k_1{}^2.(\,k_2 + p\,)^2.(\,k_1 - p\,)^2}$$

$$\tilde{\Sigma}_{15}(p) = -\frac{i\, e^2\,\lambda \left(4\,(k_1\cdot k_2) + 4\,k_1{}^2 + k_2{}^2\right)}{k_2{}^2.k_1{}^2.(\,k_1 + k_2\,)^{2^2}}$$

$$\tilde{\Sigma}_{16}(p) = -\frac{i\, e^4 \left(-2\,(k_1\cdot k_2) + k_1{}^2 + k_2{}^2\right)}{k_2{}^2.k_1{}^2.(\,k_1 + k_2\,)^{2^2}}$$

$$\tilde{\Sigma}_{17}(p) = \frac{i\,\lambda^2}{2\,k_2{}^2.k_1{}^2.(\,k_1 + k_2 + p\,)^2}$$

$$\tilde{\Sigma}_{18}(p) = \frac{2\,i\,D\, e^4}{k_2{}^2.k_1{}^2.(\,k_1 + k_2 + p\,)^2}$$

Now, employing the Tarasov's algorithm, we have

$$(4\pi)^D \Sigma_5(p) = -\frac{3i(3D-10)e^4 \mathbf{J}^{(D)}_{\{1,0\}\{1,0\}\{1,0\}}}{D-4}$$

$$(4\pi)^D \Sigma_7(p) = -\frac{3i(3D-10)e^4 \mathbf{J}^{(D)}_{\{1,0\}\{1,0\}\{1,0\}}}{D-4}$$

$$(4\pi)^D \Sigma_8(p) = -\frac{i e^4 \left((D-4)Dp^2\left(\mathbf{B}^{(D)}_{\{1,0\}\{1,0\}}\right)^2 - 2(16-5D)^2 \mathbf{J}^{(D)}_{\{1,0\}\{1,0\}\{1,0\}}\right)}{2(D-4)^2}$$

$$(4\pi)^D \Sigma_9(p) = \frac{4i(D-2)e^4 \mathbf{J}^{(D)}_{\{1,0\}\{1,0\}\{1,0\}}}{(D-6)(D-4)}$$

$$(4\pi)^D \Sigma_{10}(p) = \frac{16i(D-3)e^4 \mathbf{J}^{(D)}_{\{1,0\}\{1,0\}\{1,0\}}}{D-4}$$

$$(4\pi)^D \Sigma_{14}(p) = -\frac{9}{2} i e^4 p^2 \left(\mathbf{B}^{(D)}_{\{1,0\}\{1,0\}}\right)^2$$

$$(4\pi)^D \Sigma_{17}(p) = \frac{1}{2} i \lambda^2 \mathbf{J}^{(D)}_{\{1,0\}\{1,0\}\{1,0\}}$$

$$(4\pi)^D \Sigma_{18}(p) = 2iDe^4 \mathbf{J}^{(D)}_{\{1,0\}\{1,0\}\{1,0\}}$$

where we have omitted diagrams proportional to the vanishing $\mathbf{A}^{(D)}_{\{1,0\}}$ integral.

The diagrams depicted in Figs. 7 and 8 represent the contribution of LV effects to the two-loop scalar field self-energy. In our analysis, we will primarily focus on computing the expressions associated with the two-loop diagrams. Taking into account the form provided in Eq. (4), the functions $\tilde{\Sigma}_i(p)$ can be expressed as follows:

$$\tilde{\Sigma}_1(p) = \frac{i\,e^2\,\lambda\,Q_1\left(2\,(k_1\cdot p + 2\,(k_2\cdot p) + k_1\cdot k_2) + k_1{}^2\right)(\,k_2\cdot u\,)^2}{\left(k_2{}^2\right)^2.k_1{}^2.(\,k_1 + p\,)^2.(\,k_1 + k_2\,)^2}$$

$$\tilde{\Sigma}_2(p) = -\frac{i\,e^2\,\lambda\,Q_1\left(2\,(k_1\cdot p + 2\,(k_2\cdot p) + k_1\cdot k_2) + k_1{}^2\right)(\,k_2\cdot u\,)^2}{\left(k_2{}^2\right)^2.k_1{}^2.(\,k_1 + p\,)^2.(\,k_1 + k_2\,)^2}$$

$$\tilde{\Sigma}_3(p) = \frac{2\,i\,e^4\,Q_1\left(-k_1\cdot p + k_2\cdot p - k_1\cdot k_2 + k_1{}^2\right)(\,k_2\cdot u\,)^2}{\left(k_2{}^2\right)^2.k_1{}^2.(\,k_1 + p\,)^2.(\,k_1 + k_2\,)^2}$$

$$\tilde{\Sigma}_4(p) = -\Big(\big(2\,i\,e^4\,Q_2\left(k_2{}^2\,(\,k_1\cdot u\,)^2 + (k_1\cdot u)\left((k_2\cdot p)\,(k_2\cdot u) - k_2{}^2\,(p\cdot u) - 2\,(k_1\cdot k_2)\,(k_2\cdot u)\right) + \right.$$
$$\left.(k_2\cdot u)\left(-(k_1\cdot p)\,(k_2\cdot u) + (p\cdot u)\,(k_1\cdot k_2) + k_1{}^2\,(k_2\cdot u)\right)\right)\big)\Big/\left(k_2{}^2\right)^2.k_1{}^2.(\,k_1 + p\,)^2.(\,k_1 + k_2\,)^2\Big)$$

$$\tilde{\Sigma}_5(p) = \frac{i\,e^4\,Q_1\left(2\,(k_1\cdot p + 2\,(k_2\cdot p) + k_1\cdot k_2) + k_1{}^2\right)(p\cdot u + k_2\cdot u)\,(p\cdot u + 2\,(k_1\cdot u) + k_2\cdot u)}{k_2{}^2.k_1{}^2.(\,k_1 + p\,)^2.(\,k_2 - p\,)^2.(\,k_1 + k_2\,)^2}$$

$$\tilde{\Sigma}_6(p) = \frac{i\,e^4\,Q_1\left(-4\,(k_1\cdot p) - 2\,(k_2\cdot p) + 2\,(k_1\cdot k_2) + k_2{}^2\right)(k_1\cdot u - p\cdot u)\,(-p\cdot u + k_1\cdot u + 2\,(k_2\cdot u))}{k_2{}^2.k_1{}^2.(\,k_1 + p\,)^2.(\,k_2 - p\,)^2.(\,k_1 + k_2\,)^2}$$

$$\tilde{\Sigma}_7(p) = -\frac{i\,e^2\,\lambda\,Q_1\left(-4\,(k_1\cdot p) - 2\,(k_2\cdot p) + 2\,(k_1\cdot k_2) + k_2{}^2\right)(\,k_1\cdot u\,)^2}{k_1{}^2.k_2{}^2.k_1{}^2.(\,k_2 - p\,)^2.(\,k_1 + k_2\,)^2}$$

$$\tilde{\Sigma}_8(p) = \frac{i\,e^2\,\lambda\,Q_1\left(-4\,(k_1\cdot p) - 2\,(k_2\cdot p) + 2\,(k_1\cdot k_2) + k_2{}^2\right)(\,k_1\cdot u\,)^2}{k_1{}^2.k_2{}^2.k_1{}^2.(\,k_2 - p\,)^2.(\,k_1 + k_2\,)^2}$$

$$\tilde{\Sigma}_9(p) = -\frac{2\,i\,e^4\,Q_1\left(k_1\cdot p - k_2\cdot p + k_1\cdot k_2 - k_2{}^2\right)(\,k_1\cdot u\,)^2}{k_1{}^2.k_2{}^2.k_1{}^2.(\,k_2 - p\,)^2.(\,k_1 + k_2\,)^2}$$

$$\tilde{\Sigma}_{10}(p) =$$
$$-\frac{2\,i\,e^4\,Q_2\left(\left(k_2\cdot p + k_2{}^2\right)(\,k_1\cdot u\,)^2 - (k_1\cdot u)\,((k_1\cdot p)\,(k_2\cdot u) + (k_1\cdot k_2)\,(p\cdot u + 2\,(k_2\cdot u))) + k_1{}^2\,(k_2\cdot u)\,(p\cdot u + k_2\cdot u)\right)}{k_1{}^2.k_2{}^2.k_1{}^2.(\,k_2 - p\,)^2.(\,k_1 + k_2\,)^2}$$

$$\tilde{\Sigma}_{11}(p) = -\frac{i\,e^4\,Q_1\left(-4\,(k_1\cdot p) - 2\,(k_2\cdot p) + 2\,(k_1\cdot k_2) + k_2{}^2\right)\left(-2\,(k_1\cdot p) - 2\,(k_2\cdot p) + p^2 + 2\,(k_1\cdot k_2) + k_1{}^2\right)(k_2\cdot u - p\cdot u)^2}{k_2{}^2.k_1{}^2.(\,k_1 + p\,)^2.(\,k_2 - p\,)^{2^2}.(\,k_1 + k_2\,)^2}$$

$$\tilde{\Sigma}_{12}(p) =$$
$$-\Big(\big(2\,i\,e^4\,Q_2\left(2\,(k_1\cdot p + 2\,(k_2\cdot p) + k_1\cdot k_2) + k_1{}^2\right)\left(-(k_1\cdot k_2)\,(\,p\cdot u\,)^2 - p^2\,(\,k_2\cdot u\,)^2 - k_2{}^2\,(\,p\cdot u\,)^2 + (p\cdot u)\,(k_1\cdot k_2)\right.$$
$$(k_2\cdot u) + (k_1\cdot p)\,(k_2\cdot u)\,(p\cdot u - k_2\cdot u) + (k_1\cdot u)\left(p^2\,(-(k_2\cdot u)) - k_2{}^2\,(p\cdot u) + (k_2\cdot p)\,(p\cdot u + k_2\cdot u)\right) +$$
$$\left.2\,(k_2\cdot p)\,(p\cdot u)\,(k_2\cdot u)\right)\big)\Big/k_2{}^2.k_1{}^2.(\,k_1 + p\,)^2.(\,k_2 - p\,)^{2^2}.(\,k_1 + k_2\,)^2\Big)$$

$$\tilde{\Sigma}_{13}(p) = -\frac{i\,e^4\,Q_1\left(2\,(k_1\cdot p) - p^2 + 2\,(k_1\cdot k_2) + k_2{}^2\right)\left(2\,(k_2\cdot p) - p^2 + 2\,(k_1\cdot k_2) + k_1{}^2\right)(\,k_1\cdot u\,)^2}{k_1{}^2.k_2{}^2.k_1{}^2.(\,k_1 - p\,)^2.(\,k_2 - p\,)^2.(\,k_1 + k_2 - p\,)^2}$$

$$\tilde{\Sigma}_{14}(p) = \big(2\,i\,e^4\,Q_2\left(-4\,(k_1\cdot p) - 4\,(k_2\cdot p) + 4\,p^2 + 2\,(k_1\cdot k_2) + k_2{}^2\right)$$
$$\left(\left(p^2 - k_2\cdot p\right)(\,k_1\cdot u\,)^2 + (k_1\cdot u)\,((k_1\cdot p)\,(k_2\cdot u - 2\,(p\cdot u)) + (p\cdot u)\,(k_1\cdot k_2)) + k_1{}^2\,(p\cdot u)\,(p\cdot u - k_2\cdot u)\right)\big)\Big/$$
$$k_1{}^2.k_2{}^2.k_1{}^2.(\,k_1 - p\,)^2.(\,k_2 - p\,)^2.(\,k_1 + k_2 - p\,)^2$$

$$\tilde{\Sigma}_{15}(p) = -\frac{i\,e^4\,Q_1\left(2\,(k_2\cdot p) - p^2 + 2\,(k_1\cdot k_2) + k_1{}^2\right)^2(\,k_2\cdot u\,)^2}{\left(k_2{}^2\right)^2.k_1{}^2.(\,k_1 - p\,)^{2^2}.(\,k_1 + k_2 - p\,)^2}$$

$$\tilde{\Sigma}_{16}(p) = -\frac{i\,e^4\,Q_1\left(2\,(k_2\cdot p) - p^2 + 2\,(k_1\cdot k_2) + k_1{}^2\right)^2(\,k_2\cdot u\,)^2}{\left(k_2{}^2\right)^2.k_1{}^2.(\,k_1 - p\,)^{2^2}.(\,k_1 + k_2 - p\,)^2}$$

$$\tilde{\Sigma}_{17}(p) = -\frac{i\,e^4\,Q_1\left(-4\,(k_1\cdot p)+4\,p^2+k_1{}^2\right)\left(-2\,(k_1\cdot p)+2\,(k_2\cdot p)+p^2-2\,(k_1\cdot k_2)+k_1{}^2+k_2{}^2\right)(\,k_2\cdot u\,)^2}{\left(k_2{}^2\right)^2.k_1{}^2.(\,k_1-p\,)^{2^2}.(\,k_1+k_2-p\,)^2}$$

$$\tilde{\Sigma}_{18}(p) = \frac{1}{\left(k_2{}^2\right)^2.k_1{}^2.(\,k_1-p\,)^{2^2}.(\,k_1+k_2-p\,)^2}$$

$$2\,i\,e^4\,Q_2\left(-4\,(k_1\cdot p)+4\,p^2+k_1{}^2\right)\left(-2\,(k_1\cdot p)\,(\,k_2\cdot u\,)^2+k_2{}^2\,(\,p\cdot u\,)^2+p^2\,(\,k_2\cdot u\,)^2+k_2{}^2\,(\,k_1\cdot u\,)^2+k_1{}^2\,(\,k_2\cdot u\,)^2-\right.$$
$$\left.2\,(k_1\cdot u)\left(-(k_2\cdot p)\,(k_2\cdot u)+k_2{}^2\,(p\cdot u)+(k_1\cdot k_2)\,(k_2\cdot u)\right)+2\,(p\cdot u)\,(k_1\cdot k_2)\,(k_2\cdot u)-2\,(k_2\cdot p)\,(p\cdot u)\,(k_2\cdot u)\right)$$

$$\tilde{\Sigma}_{19}(p) = -\frac{i\,e^2\,\lambda\,Q_1\,(p\cdot u+k_1\cdot u)\,(-p\cdot u+k_1\cdot u-2\,(k_2\cdot u))}{k_2{}^2.k_1{}^2.(\,k_1-p\,)^2.(\,-k_1+k_2+p\,)^2}$$

$$\tilde{\Sigma}_{20}(p) = -\frac{2\,i\,e^4\,Q_1\,(k_1\cdot u-2\,(p\cdot u))\,(-p\cdot u+k_1\cdot u+k_2\cdot u)}{k_2{}^2.k_1{}^2.(\,k_1-p\,)^2.(\,-k_1+k_2+p\,)^2}$$

$$\tilde{\Sigma}_{21}(p) = -\frac{i\,e^2\,\lambda\,Q_1\,(k_1\cdot u-2\,(p\cdot u))^2}{k_1{}^2.k_2{}^2.(\,k_1-p\,)^{2^2}}$$

$$\tilde{\Sigma}_{22}(p) = -\frac{2\,i\,e^4\,Q_1\,(p\cdot u+k_1\cdot u)^2}{k_1{}^2.k_2{}^2.(\,k_1-p\,)^{2^2}}$$

$$\tilde{\Sigma}_{23}(p) = -\frac{i\,D\,e^4\,Q_1\,(k_1\cdot u-2\,(p\cdot u))^2}{k_1{}^2.k_2{}^2.(\,k_1-p\,)^{2^2}}$$

$$\tilde{\Sigma}_{24}(p) = -\frac{2\,i\,e^4\,Q_1\,(k_1\cdot u-p\cdot u)\,(k_1\cdot u-k_2\cdot u)}{k_2{}^2.k_1{}^2.(\,k_1+p\,)^2.(\,k_1+k_2\,)^2}$$

$$\tilde{\Sigma}_{25}(p) = -\frac{2\,i\,e^4\,Q_1\,(p\cdot u+k_1\cdot u)^2}{k_1{}^2.k_2{}^2.(\,k_1-p\,)^{2^2}}$$

$$\tilde{\Sigma}_{27}(p) = -\frac{i\,\lambda^2\,Q_1\,(\,k_1\cdot u\,)^2}{k_1{}^2.k_2{}^2.k_1{}^2.(\,-k_1+k_2+p\,)^2}$$

$$\tilde{\Sigma}_{28}(p) = -\frac{i\,\lambda^2\,Q_1\,(\,k_1\cdot u\,)^2}{2\,k_1{}^2.k_2{}^2.k_1{}^2.(\,-k_1+k_2+p\,)^2}$$

$$\tilde{\Sigma}_{29}(p) = -\frac{2\,i\,D\,e^4\,Q_1\,(\,k_1\cdot u\,)^2}{k_1{}^2.k_2{}^2.k_1{}^2.(\,-k_1+k_2+p\,)^2}$$

$$\tilde{\Sigma}_{30}(p) = \frac{2\,i\,(D-2)\,e^4\,Q_2\,(\,k_1\cdot u\,)^2}{k_1{}^2.k_2{}^2.k_1{}^2.(\,-k_1+k_2+p\,)^2}$$

$$\tilde{\Sigma}_{31}(p) = -\frac{i\,e^2\,\lambda\,Q_1\,(2\,(p\cdot u)+k_1\cdot u)\,(k_1\cdot u-2\,(k_2\cdot u))}{k_2{}^2.k_1{}^2.(\,k_1+p\,)^2.(\,k_2-k_1\,)^2}$$

$$\tilde{\Sigma}_{32}(p) = -\frac{2\,i\,e^4\,Q_1\,(k_1\cdot u-p\cdot u)\,(k_1\cdot u+k_2\cdot u)}{k_2{}^2.k_1{}^2.(\,k_1+p\,)^2.(\,k_2-k_1\,)^2}$$

$$\tilde{\Sigma}_{33}(p) = \frac{i\,e^2\,\lambda\,Q_1\,(k_1\cdot u-k_2\cdot u)\,(2\,(p\cdot u)+k_1\cdot u+k_2\cdot u)}{k_2{}^2.k_1{}^2.(\,k_1+k_2\,)^2.(\,k_1+k_2+p\,)^2}$$

$$\tilde{\Sigma}_{34}(p) = -\frac{2\,i\,e^4\,Q_1\,(2\,(k_1\cdot u)+k_2\cdot u)\,(-p\cdot u+k_1\cdot u+k_2\cdot u)}{k_2{}^2.k_1{}^2.(\,k_1+k_2\,)^2.(\,k_1+k_2+p\,)^2}$$

$$\tilde{\Sigma}_{35}(p) = -\frac{i\,\lambda^2\,Q_1\,(\,k_1\cdot u\,)^2}{\left(k_1{}^2\right)^3.k_2{}^2}$$

$$\tilde{\Sigma}_{36}(p) = -\frac{i\,\lambda^2\,Q_1\,(\,k_1\cdot u\,)^2}{\left(k_1{}^2\right)^3.k_2{}^2}$$

$$\tilde{\Sigma}_{37}(p) = -\frac{i\,D\,\mathrm{e}^2\,\lambda\,Q_1\,(\,k_1\cdot u\,)^2}{\left(k_1{}^2\right)^3.k_2{}^2}$$

$$\tilde{\Sigma}_{38}(p) = -\frac{i\,D\,\mathrm{e}^2\,\lambda\,Q_1\,(\,k_1\cdot u\,)^2}{\left(k_1{}^2\right)^3.k_2{}^2}$$

$$\tilde{\Sigma}_{39}(p) = \frac{2\,i\,(D-2)\,\mathrm{e}^4\,Q_2\,(\,k_1\cdot u\,)^2}{\left(k_1{}^2\right)^3.k_2{}^2}$$

$$\tilde{\Sigma}_{40}(p) = -\frac{i\,\mathrm{e}^2\,\lambda\,Q_1\,(2\,(k_1\cdot u) + k_2\cdot u)^2}{k_2{}^2.k_1{}^2.(\,k_1 + k_2\,)^{2\,2}}$$

$$\tilde{\Sigma}_{41}(p) = -\frac{i\,\mathrm{e}^2\,\lambda\,Q_1\,(2\,(k_1\cdot u) + k_2\cdot u)^2}{k_2{}^2.k_1{}^2.(\,k_1 + k_2\,)^{2\,2}}$$

$$\tilde{\Sigma}_{42}(p) = -\frac{2\,i\,\mathrm{e}^4\,Q_1\,(k_1\cdot u - k_2\cdot u)^2}{k_2{}^2.k_1{}^2.(\,k_1 + k_2\,)^{2\,2}}$$

$$\tilde{\Sigma}_{43}(p) = -\frac{i\,\mathrm{e}^2\,\lambda\,Q_1\,(2\,(p\cdot u) + k_1\cdot u)^2}{k_1{}^2.k_2{}^2.(\,k_1 + p\,)^{2\,2}}$$

$$\tilde{\Sigma}_{44}(p) = -\frac{2\,i\,\mathrm{e}^4\,Q_1\,(k_1\cdot u - p\cdot u)^2}{k_1{}^2.k_2{}^2.(\,k_1 + p\,)^{2\,2}}$$

$$\tilde{\Sigma}_{45}(p) = -\frac{i\,D\,\mathrm{e}^4\,Q_1\,(2\,(p\cdot u) + k_1\cdot u)^2}{k_1{}^2.k_2{}^2.(\,k_1 + p\,)^{2\,2}}$$

$$\tilde{\Sigma}_{46}(p) = -\frac{i\,\mathrm{e}^2\,\lambda\,Q_1\,(k_1\cdot u - k_2\cdot u)\,(-2\,(p\cdot u) + k_1\cdot u + k_2\cdot u)}{k_2{}^2.k_1{}^2.(\,k_1 + k_2\,)^2.(\,k_1 + k_2 - p\,)^2}$$

$$\tilde{\Sigma}_{47}(p) = -\frac{2\,i\,\mathrm{e}^4\,Q_1\,(2\,(k_1\cdot u) + k_2\cdot u)\,(p\cdot u + k_1\cdot u + k_2\cdot u)}{k_2{}^2.k_1{}^2.(\,k_1 + k_2\,)^2.(\,k_1 + k_2 - p\,)^2}$$

$$\tilde{\Sigma}_{48}(p) = -\frac{2\,i\,\mathrm{e}^4\,Q_1\,(p\cdot u + k_1\cdot u)\,(k_1\cdot u - k_2\cdot u)}{k_2{}^2.k_1{}^2.(\,k_1 - p\,)^2.(\,k_1 + k_2\,)^2}$$

$$\tilde{\Sigma}_{49}(p) = \frac{i\,\mathrm{e}^2\,\lambda\,Q_1\left(2\,(k_1\cdot p) + p^2 + k_1{}^2\right)(\,k_1\cdot u\,)^2}{\left(k_1{}^2\right)^3.k_2{}^2.(\,k_1 - p\,)^2}$$

$$\tilde{\Sigma}_{50}(p) = \frac{i\,D\,\mathrm{e}^4\,Q_1\left(2\,(k_1\cdot p) + p^2 + k_1{}^2\right)(\,k_1\cdot u\,)^2}{\left(k_1{}^2\right)^3.k_2{}^2.(\,k_1 - p\,)^2}$$

$$\tilde{\Sigma}_{51}(p) = -\frac{4\,i\,\mathrm{e}^4\,Q_2\left(p^2\,(\,k_1\cdot u\,)^2 + k_1{}^2\,(\,p\cdot u\,)^2 - 2\,(k_1\cdot p)\,(p\cdot u)\,(k_1\cdot u)\right)}{\left(k_1{}^2\right)^3.k_2{}^2.(\,k_1 - p\,)^2}$$

$$\tilde{\Sigma}_{52}(p) = \frac{2\,i\,\mathrm{e}^4\,Q_1\left(2\,(k_1\cdot p) + p^2 + k_1{}^2\right)(\,k_1\cdot u\,)^2}{\left(k_1{}^2\right)^2.k_2{}^2.(\,k_1 - p\,)^{2\,2}}$$

$$\tilde{\Sigma}_{53}(p) = -\frac{2\,i\,e^2\,\lambda\,Q_2\left(p^2\,(k_1\cdot u)^2 + k_1{}^2\,(p\cdot u)^2 - 2\,(k_1\cdot p)\,(p\cdot u)\,(k_1\cdot u)\right)}{\left(k_1{}^2\right)^2.k_2{}^2.(k_1-p)^{2^2}}$$

$$\tilde{\Sigma}_{54}(p) = -\frac{2\,i\,D\,e^4\,Q_2\left(p^2\,(k_1\cdot u)^2 + k_1{}^2\,(p\cdot u)^2 - 2\,(k_1\cdot p)\,(p\cdot u)\,(k_1\cdot u)\right)}{\left(k_1{}^2\right)^2.k_2{}^2.(k_1-p)^{2^2}}$$

$$\tilde{\Sigma}_{55}(p) = -\frac{2\,i\,e^4\,Q_1\left(-k_1\cdot p + k_2\cdot p - p^2 + k_1\cdot k_2\right)(k_1\cdot u)^2}{\left(k_1{}^2\right)^2.k_2{}^2.(k_1-p)^2.(k_2+p)^2}$$

$$\tilde{\Sigma}_{56}(p) =$$

$$\frac{2\,i\,e^4\,Q_2\left(\left(k_2\cdot p - p^2\right)(k_1\cdot u)^2 - (k_1\cdot u)\,((k_1\cdot p)\,(k_2\cdot u - 2\,(p\cdot u)) + (p\cdot u)\,(k_1\cdot k_2)) + k_1{}^2\,(p\cdot u)\,(k_2\cdot u - p\cdot u)\right)}{\left(k_1{}^2\right)^2.k_2{}^2.(k_1-p)^2.(k_2+p)^2}$$

$$\tilde{\Sigma}_{57}(p) = \frac{i\,e^2\,\lambda\,Q_1\left(-4\,(k_1\cdot p) + 4\,p^2 + k_1{}^2\right)(k_1\cdot u - p\cdot u)^2}{k_1{}^2.k_2{}^2.(k_1-p)^{2^3}}$$

$$\tilde{\Sigma}_{58}(p) = \frac{i\,D\,e^4\,Q_1\left(-4\,(k_1\cdot p) + 4\,p^2 + k_1{}^2\right)(k_1\cdot u - p\cdot u)^2}{k_1{}^2.k_2{}^2.(k_1-p)^{2^3}}$$

$$\tilde{\Sigma}_{59}(p) = -\frac{4\,i\,e^4\,Q_2\left(p^2\,(k_1\cdot u)^2 + k_1{}^2\,(p\cdot u)^2 - 2\,(k_1\cdot p)\,(p\cdot u)\,(k_1\cdot u)\right)}{k_1{}^2.k_2{}^2.(k_1-p)^{2^3}}$$

$$\tilde{\Sigma}_{60}(p) = \frac{i\,e^2\,\lambda\,Q_1\left(-4\,(k_1\cdot p) + 4\,p^2 + k_1{}^2\right)(k_2\cdot u)^2}{k_1{}^2.\left(k_2{}^2\right)^2.(k_1-p)^{2^2}}$$

$$\tilde{\Sigma}_{61}(p) = \frac{2\,i\,e^4\,Q_1\left(2\,(k_1\cdot p) + p^2 + k_1{}^2\right)(k_2\cdot u)^2}{k_1{}^2.\left(k_2{}^2\right)^2.(k_1-p)^{2^2}}$$

$$\tilde{\Sigma}_{62}(p) = -\frac{i\,(D-2)\,e^4\,Q_2\left(-4\,(k_1\cdot p) + 4\,p^2 + k_1{}^2\right)(k_2\cdot u)^2}{2\,k_1{}^2.\left(k_2{}^2\right)^2.(k_1-p)^{2^2}}$$

$$\tilde{\Sigma}_{63}(p) = \frac{2\,i\,e^4\,Q_1\left(k_1\cdot p + k_2\cdot p + p^2 + k_1\cdot k_2\right)(k_2\cdot u)^2}{\left(k_2{}^2\right)^2.k_1{}^2.(k_2-p)^2.(k_1-p)^2}$$

$$\tilde{\Sigma}_{64}(p) = \left(2\,i\,e^4\,Q_2\left(-(k_1\cdot p)\,(k_2\cdot u)^2 - p^2\,(k_2\cdot u)^2 - k_2{}^2\,(p\cdot u)^2 + (p\cdot u)\,(k_1\cdot k_2)\,(k_2\cdot u) + \right.\right.$$
$$\left.\left.(k_1\cdot u)\left((k_2\cdot p)\,(k_2\cdot u) - k_2{}^2\,(p\cdot u)\right) + 2\,(k_2\cdot p)\,(p\cdot u)\,(k_2\cdot u)\right)\right)\Big/\left(k_2{}^2\right)^2.k_1{}^2.(k_2-p)^2.(k_1-p)^2$$

$$\tilde{\Sigma}_{65}(p) = -\frac{i\,e^2\,\lambda\,Q_1\left(2\,(k_2\cdot p + k_1\cdot k_2) - p^2 + k_1{}^2\right)(k_1\cdot u)^2}{k_1{}^2.k_2{}^2.k_1{}^2.(k_1-p)^2.(k_1+k_2-p)^2}$$

$$\tilde{\Sigma}_{66}(p) =$$

$$-\frac{2\,i\,e^4\,Q_2\left(\left(k_2\cdot p + p^2\right)(k_1\cdot u)^2 - (k_1\cdot u)\,((p\cdot u)\,(k_1\cdot k_2) + (k_1\cdot p)\,(2\,(p\cdot u) + k_2\cdot u)) + k_1{}^2\,(p\cdot u)\,(p\cdot u + k_2\cdot u)\right)}{k_1{}^2.k_2{}^2.k_1{}^2.(k_1-p)^2.(k_1+k_2-p)^2}$$

$$\tilde{\Sigma}_{67}(p) = \frac{2\,i\,e^2\,\lambda\,Q_2\left((k_2\cdot p)\,(k_1\cdot u)^2 - (k_1\cdot u)\,((k_1\cdot p)\,(k_2\cdot u) + (p\cdot u)\,(k_1\cdot k_2)) + k_1{}^2\,(p\cdot u)\,(k_2\cdot u)\right)}{k_1{}^2.k_2{}^2.k_1{}^2.(k_1-p)^2.(k_2-k_1)^2}$$

$$\tilde{\Sigma}_{68}(p) = \frac{2\,i\,e^4\,Q_1\left(k_1\cdot p + k_2\cdot p + k_1\cdot k_2 + k_1{}^2\right)(k_1\cdot u)^2}{k_1{}^2.k_2{}^2.k_1{}^2.(k_1-p)^2.(k_2-k_1)^2}$$

$$\tilde{\Sigma}_{69}(p) = \frac{i\,e^4\,Q_1\left(-4\,(k_1\cdot p) + 4\,p^2 + k_1{}^2\right)(p\cdot u - (k_1\cdot u) + k_2\cdot u)^2}{k_2{}^2.k_1{}^2.(\,k_1 - p\,)^{22}.(\,k_1 + k_2 - p\,)^2}$$

$$\tilde{\Sigma}_{70}(p) = \frac{i\,e^4\,Q_1\left(2\,(k_2\cdot p) - p^2 + 2\,(k_1\cdot k_2) + k_1{}^2\right)(p\cdot u + k_1\cdot u)\,(-p\cdot u + k_1\cdot u + 2\,(k_2\cdot u))}{k_2{}^2.k_1{}^2.(\,k_1 - p\,)^{22}.(\,k_1 + k_2 - p\,)^2}$$

$$\tilde{\Sigma}_{71}(p) = \frac{i\,e^4\,Q_1\left(-4\,(k_1\cdot p) + 4\,p^2 + k_1{}^2\right)(-p\cdot u + k_1\cdot u + k_2\cdot u)^2}{k_2{}^2.k_1{}^2.(\,k_1 - p\,)^{22}.(\,-k_1 + k_2 + p\,)^2}$$

$$\tilde{\Sigma}_{72}(p) = \frac{i\,e^4\,Q_1\left(-2\,(k_2\cdot p) - p^2 - 2\,(k_1\cdot k_2) + k_1{}^2\right)(p\cdot u + k_1\cdot u)\,(-p\cdot u + k_1\cdot u - 2\,(k_2\cdot u))}{k_2{}^2.k_1{}^2.(\,k_1 - p\,)^{22}.(\,-k_1 + k_2 + p\,)^2}$$

$$\tilde{\Sigma}_{73}(p) = \frac{i\,e^4\,Q_1\left(2\,(k_1\cdot p) - 4\,(k_2\cdot p) - 2\,(k_1\cdot k_2) + k_1{}^2\right)(2\,(p\cdot u) + k_1\cdot u)\,(k_1\cdot u - 2\,(k_2\cdot u))}{k_2{}^2.\left(k_1{}^2\right)^2.(\,k_1 + p\,)^2.(\,k_2 - k_1\,)^2}$$

$$\tilde{\Sigma}_{74}(p) = \frac{i\,e^4\,Q_1\left(2\,(k_1\cdot k_2) + k_1{}^2 + k_2{}^2\right)(k_1\cdot u - p\cdot u)^2}{k_2{}^2.\left(k_1{}^2\right)^2.(\,k_1 + p\,)^2.(\,k_2 - k_1\,)^2}$$

$$\tilde{\Sigma}_{75}(p) = \frac{i\,e^4\,Q_1\left(2\,(k_2\cdot p) - p^2 - 2\,(k_1\cdot k_2) + k_1{}^2\right)(k_1\cdot u + k_2\cdot u)\,(2\,(p\cdot u) + k_1\cdot u - k_2\cdot u)}{k_2{}^2.k_1{}^2.(\,k_1 + p\,)^2.(\,k_1 - k_2\,)^2.(\,-k_1 + k_2 - p\,)^2}$$

$$\tilde{\Sigma}_{76}(p) = \frac{2\,i\,e^2\,\lambda\,Q_2\left((k_2\cdot p)\,(\,k_1\cdot u\,)^2 - (k_1\cdot u)\,((k_1\cdot p)\,(k_2\cdot u) + (p\cdot u)\,(k_1\cdot k_2)) + k_1{}^2\,(p\cdot u)\,(k_2\cdot u)\right)}{k_1{}^2.k_2{}^2.k_1{}^2.(\,k_1 - p\,)^2.(\,k_1 + k_2\,)^2}$$

$$\tilde{\Sigma}_{77}(p) = \frac{2\,i\,e^4\,Q_1\left(k_1\cdot p - k_2\cdot p - k_1\cdot k_2 + k_1{}^2\right)(\,k_1\cdot u\,)^2}{k_1{}^2.k_2{}^2.k_1{}^2.(\,k_1 - p\,)^2.(\,k_1 + k_2\,)^2}$$

$$\tilde{\Sigma}_{78}(p) = \frac{i\,e^2\,\lambda\,Q_1\left(-2\,(k_2\cdot p + k_1\cdot k_2) - p^2 + k_1{}^2\right)(\,k_1\cdot u\,)^2}{k_1{}^2.k_2{}^2.k_1{}^2.(\,k_1 - p\,)^2.(\,-k_1 + k_2 + p\,)^2}$$

$$\tilde{\Sigma}_{79}(p) =$$

$$\frac{2\,i\,e^4\,Q_2\left(\left(k_2\cdot p - p^2\right)(\,k_1\cdot u\,)^2 - (k_1\cdot u)\,((k_1\cdot p)\,(k_2\cdot u - 2\,(p\cdot u)) + (p\cdot u)\,(k_1\cdot k_2)) + k_1{}^2\,(p\cdot u)\,(k_2\cdot u - p\cdot u)\right)}{k_1{}^2.k_2{}^2.k_1{}^2.(\,k_1 - p\,)^2.(\,-k_1 + k_2 + p\,)^2}$$

$$\tilde{\Sigma}_{80}(p) = \frac{i\,e^2\,\lambda\,Q_1\left(2\,(k_1\cdot k_2) + k_1{}^2 + k_2{}^2\right)(\,k_1\cdot u\,)^2}{k_1{}^2.k_2{}^2.\left(k_1{}^2\right)^2.(\,k_2 - k_1\,)^2}$$

$$\tilde{\Sigma}_{81}(p) = \frac{i\,e^2\,\lambda\,Q_1\left(2\,(k_1\cdot k_2) + k_1{}^2 + k_2{}^2\right)(\,k_1\cdot u\,)^2}{k_1{}^2.k_2{}^2.\left(k_1{}^2\right)^2.(\,k_2 - k_1\,)^2}$$

$$\tilde{\Sigma}_{82}(p) = -\frac{4\,i\,e^4\,Q_2\left(k_2{}^2\,(\,k_1\cdot u\,)^2 + k_1{}^2\,(\,k_2\cdot u\,)^2 - 2\,(k_1\cdot k_2)\,(k_1\cdot u)\,(k_2\cdot u)\right)}{k_1{}^2.k_2{}^2.\left(k_1{}^2\right)^2.(\,k_2 - k_1\,)^2}$$

$$\tilde{\Sigma}_{83}(p) = \frac{i\,e^2\,\lambda\,Q_1\left(-4\,(k_1\cdot k_2) + 4\,k_1{}^2 + k_2{}^2\right)(\,k_1\cdot u\,)^2}{k_1{}^2.k_2{}^2.k_1{}^2.(\,k_2 - k_1\,)^2.(\,k_1 - k_2\,)^2}$$

$$\tilde{\Sigma}_{84}(p) = \frac{2\,i\,e^4\,Q_1\left(2\,(k_1\cdot k_2) + k_1{}^2 + k_2{}^2\right)(\,k_1\cdot u\,)^2}{k_1{}^2.k_2{}^2.k_1{}^2.(\,k_2 - k_1\,)^2.(\,k_1 - k_2\,)^2}$$

$$\tilde{\Sigma}_{85}(p) = -\frac{2\,i\,e^2\,\lambda\,Q_2\left(k_2{}^2\,(\,k_1\cdot u\,)^2 + k_1{}^2\,(\,k_2\cdot u\,)^2 - 2\,(k_1\cdot k_2)\,(k_1\cdot u)\,(k_2\cdot u)\right)}{k_1{}^2.k_2{}^2.k_1{}^2.(\,k_2 - k_1\,)^2.(\,k_1 - k_2\,)^2}$$

$$\tilde{\Sigma}_{86}(p) = \frac{i\, e^4\, Q_1 \left(k_1{}^2 - 2\,(k_1\cdot p - 2\,(k_2\cdot p) + k_1\cdot k_2)\right)(k_1\cdot u - 2\,(p\cdot u))\,(k_1\cdot u - 2\,(k_2\cdot u))}{k_2{}^2.\left(k_1{}^2\right)^2.(\,k_1 - p\,)^2.(\,k_2 - k_1\,)^2}$$

$$\tilde{\Sigma}_{87}(p) = \frac{i\, e^4\, Q_1 \left(2\,(k_1\cdot k_2) + k_1{}^2 + k_2{}^2\right)(p\cdot u + k_1\cdot u)^2}{k_2{}^2.\left(k_1{}^2\right)^2.(\,k_1 - p\,)^2.(\,k_2 - k_1\,)^2}$$

$$\tilde{\Sigma}_{88}(p) = \frac{i\, e^4\, Q_1 \left(-2\,(k_2\cdot p) - p^2 - 2\,(k_1\cdot k_2) + k_1{}^2\right)(k_1\cdot u + k_2\cdot u)\,(-2\,(p\cdot u) + k_1\cdot u - k_2\cdot u)}{k_2{}^2.k_1{}^2.(\,k_1 - p\,)^2.(\,k_1 - k_2\,)^2.(\,-k_1 + k_2 + p\,)^2}$$

$$\tilde{\Sigma}_{89}(p) = -\frac{i\, e^4\, Q_1 \left(2\,(k_1\cdot p) - 2\,(k_2\cdot p) + k_1{}^2 - k_2{}^2\right)\left(-2\,(k_2\cdot p) - p^2 + 2\,(k_1\cdot k_2) + k_1{}^2\right)(\,k_2\cdot u\,)^2}{\left(k_2{}^2\right)^2.k_1{}^2.(\,k_1 + p\,)^2.(\,k_1 + k_2\,)^2.(\,k_1 + k_2 + p\,)^2}$$

$$\tilde{\Sigma}_{90}(p) = -\frac{i\, e^4\, Q_1 \left(2\,(k_2\cdot p) + p^2 + 2\,(k_1\cdot k_2) - k_1{}^2\right)^2(\,k_1\cdot u\,)^2}{k_1{}^2.k_2{}^2.k_1{}^2.(\,k_1 - p\,)^{22}.(\,-k_1 + k_2 + p\,)^2}$$

$$\tilde{\Sigma}_{91}(p) = \frac{2\, i\, e^4\, Q_2 \left(-2\,(k_1\cdot p) - 2\,(k_2\cdot p) + p^2 + 2\,(k_1\cdot k_2) + k_1{}^2 + k_2{}^2\right)\left(p^2\,(\,k_1\cdot u\,)^2 + k_1{}^2\,(\,p\cdot u\,)^2 - 2\,(k_1\cdot p)\,(p\cdot u)\,(k_1\cdot u)\right)}{k_1{}^2.k_2{}^2.k_1{}^2.(\,k_1 - p\,)^{22}.(\,-k_1 + k_2 + p\,)^2}$$

$$\tilde{\Sigma}_{92}(p) = -\frac{i\, e^4\, Q_1 \left(2\,(k_1\cdot p) + p^2 + k_1{}^2\right)\left(-2\,(k_1\cdot k_2) + k_1{}^2 + k_2{}^2\right)(\,k_1\cdot u\,)^2}{\left(k_1{}^2\right)^2.k_2{}^2.k_1{}^2.(\,k_1 - p\,)^2.(\,k_1 + k_2\,)^2}$$

$$\tilde{\Sigma}_{93}(p) = -\Big(\Big(2\, i\, e^4\, Q_2 \left(-2\,(k_1\cdot p) - 4\,(k_2\cdot p) + 2\,(k_1\cdot k_2) + k_1{}^2\right)\big((k_2\cdot p)\,(\,k_1\cdot u\,)^2 - (k_1\cdot u)\,((k_1\cdot p)\,(k_2\cdot u) + (p\cdot u)\,(k_1\cdot k_2)) + k_1{}^2\,(p\cdot u)\,(k_2\cdot u)\big)\Big)\Big/\left(\left(k_1{}^2\right)^2.k_2{}^2.k_1{}^2.(\,k_1 - p\,)^2.(\,k_1 + k_2\,)^2\right)\Big)$$

$$\tilde{\Sigma}_{94}(p) = -\frac{i\, e^4\, Q_1 \left(-4\,(k_1\cdot p) + 4\,p^2 + k_1{}^2\right)\left(-2\,(k_1\cdot p) - 2\,(k_2\cdot p) + p^2 + 2\,(k_1\cdot k_2) + k_1{}^2 + k_2{}^2\right)(k_1\cdot u - p\cdot u)^2}{k_2{}^2.k_1{}^2.(\,k_1 - p\,)^{23}.(\,-k_1 + k_2 + p\,)^2}$$

$$\tilde{\Sigma}_{95}(p) = -\frac{1}{k_2{}^2.k_1{}^2.(\,k_1 - p\,)^{23}.(\,-k_1 + k_2 + p\,)^2}\, 2\, i\, e^4\, Q_2 \left(-2\,(k_2\cdot p) - p^2 - 2\,(k_1\cdot k_2) + k_1{}^2\right) \Big((k_2\cdot p)\,(\,k_1\cdot u\,)^2 - (k_1\cdot u)\left((k_1\cdot p)\,(k_2\cdot u) + (p\cdot u)\,(k_2\cdot p + k_1\cdot k_2) - p^2\,(k_2\cdot u)\right) + (p\cdot u)\left(-(k_1\cdot p)\,(k_2\cdot u) + (p\cdot u)\,(k_1\cdot k_2) + k_1{}^2\,(k_2\cdot u)\right)\Big)$$

$$\tilde{\Sigma}_{99}(p) = \frac{2\, i\, e^4\, Q_1\,(p\cdot u + k_1\cdot u)\,(k_2\cdot u - p\cdot u)}{k_2{}^2.k_1{}^2.(\,k_2 + p\,)^2.(\,k_1 - p\,)^2}$$

$$\tilde{\Sigma}_{100}(p) = -\frac{2\, i\, e^4\, Q_1\,(p\cdot u + k_1\cdot u)\,(p\cdot u - k_2\cdot u)}{k_2{}^2.k_1{}^2.(\,k_2 + p\,)^2.(\,k_1 - p\,)^2}$$

$$\tilde{\Sigma}_{101}(p) = -\frac{i\, \lambda^2\, Q_1\,(\,k_1\cdot u\,)^2}{\left(k_2{}^2\right)^2.\left(k_1{}^2\right)^2}$$

$$\tilde{\Sigma}_{102}(p) = -\frac{2\, i\, D\, e^4\, Q_1\,(\,k_1\cdot u\,)^2}{\left(k_2{}^2\right)^2.\left(k_1{}^2\right)^2}$$

$$\tilde{\Sigma}_{103}(p) = \frac{i\,(D-2)\, e^2\, \lambda\, Q_2\,(\,k_1\cdot u\,)^2}{2\left(k_2{}^2\right)^2.\left(k_1{}^2\right)^2}$$

$$\tilde{\Sigma}_{104}(p) = \frac{2\, i\, e^4\, Q_1\,(k_1\cdot u - p\cdot u)\,(p\cdot u + k_2\cdot u)}{k_2{}^2.k_1{}^2.(\,k_2 - p\,)^2.(\,k_1 + p\,)^2}$$

$$\tilde{\Sigma}_{105}(p) = -\frac{i\, e^4\, Q_1\,(k_1\cdot u - k_2\cdot u)^2}{k_2{}^2.k_1{}^2.(\,k_1 + k_2\,)^{22}}$$

where we have omitted the vanishing amplitudes proportional to $u^2$.

Employing the Tarasov's algorithm, we find

$$(4\pi)^D\,\Sigma_1(p) = \frac{i\,D\left(D^2-11\,D+24\right)e^2\,\lambda\,Q_1\,(p\cdot u)^2\,\mathbf{J}^{(D)}_{\{1,0\}\{1,0\}\{1,0\}}}{3\,(D-6)\,(D-4)\,(D-1)\,p^2}$$

$$(4\pi)^D\,\Sigma_2(p) = -\frac{i\,D\left(D^2-11\,D+24\right)e^2\,\lambda\,Q_1\,(p\cdot u)^2\,\mathbf{J}^{(D)}_{\{1,0\}\{1,0\}\{1,0\}}}{3\,(D-6)\,(D-4)\,(D-1)\,p^2}$$

$$(4\pi)^D\,\Sigma_3(p) = -\frac{i\left(9\,D^4-119\,D^3+550\,D^2-1002\,D+540\right)e^4\,Q_1\,(p\cdot u)^2\,\mathbf{J}^{(D)}_{\{1,0\}\{1,0\}\{1,0\}}}{3\,(D-6)\,(D-4)\,(D-1)\,p^2}$$

$$(4\pi)^D\,\Sigma_4(p) = -\frac{5\,i\left(D^2-5\,D+6\right)e^4\,Q_2\,(p\cdot u)^2\,\mathbf{J}^{(D)}_{\{1,0\}\{1,0\}\{1,0\}}}{3\,(D-4)\,p^2}$$

$$(4\pi)^D\,\Sigma_5(p) =$$
$$-\frac{i\,e^4\,Q_1\,(p\cdot u)^2\left(3\,D\left(3\,D^2-20\,D+32\right)p^2\left(\mathbf{B}^{(D)}_{\{1,0\}\{1,0\}}\right)^2+4\left(-75\,D^3+565\,D^2-1276\,D+768\right)\mathbf{J}^{(D)}_{\{1,0\}\{1,0\}\{1,0\}}\right)}{12\,(D-4)^2\,(D-1)\,p^2}$$

$$(4\pi)^D\,\Sigma_6(p) =$$
$$-\frac{i\,e^4\,Q_1\,(p\cdot u)^2\left(3\,D\left(3\,D^2-20\,D+32\right)p^2\left(\mathbf{B}^{(D)}_{\{1,0\}\{1,0\}}\right)^2+4\left(-75\,D^3+565\,D^2-1276\,D+768\right)\mathbf{J}^{(D)}_{\{1,0\}\{1,0\}\{1,0\}}\right)}{12\,(D-4)^2\,(D-1)\,p^2}$$

$$(4\pi)^D\,\Sigma_7(p) = -\frac{i\,D\left(D^2-11\,D+24\right)e^2\,\lambda\,Q_1\,(p\cdot u)^2\,\mathbf{J}^{(D)}_{\{1,0\}\{1,0\}\{1,0\}}}{3\,(D-6)\,(D-4)\,(D-1)\,p^2}$$

$$(4\pi)^D\,\Sigma_8(p) = \frac{i\,D\left(D^2-11\,D+24\right)e^2\,\lambda\,Q_1\,(p\cdot u)^2\,\mathbf{J}^{(D)}_{\{1,0\}\{1,0\}\{1,0\}}}{3\,(D-6)\,(D-4)\,(D-1)\,p^2}$$

$$(4\pi)^D\,\Sigma_9(p) = -\frac{i\left(9\,D^4-119\,D^3+550\,D^2-1002\,D+540\right)e^4\,Q_1\,(p\cdot u)^2\,\mathbf{J}^{(D)}_{\{1,0\}\{1,0\}\{1,0\}}}{3\,(D-6)\,(D-4)\,(D-1)\,p^2}$$

$$(4\pi)^D\,\Sigma_{10}(p) = -\frac{5\,i\left(D^2-5\,D+6\right)e^4\,Q_2\,(p\cdot u)^2\,\mathbf{J}^{(D)}_{\{1,0\}\{1,0\}\{1,0\}}}{3\,(D-4)\,p^2}$$

$$(4\pi)^D\,\Sigma_{11}(p) = -\Bigg(\bigg(i\,e^4\,Q_1\,(p\cdot u)^2\Big(3\,D\left(D^4-22\,D^3+164\,D^2-488\,D+480\right)p^2\left(\mathbf{B}^{(D)}_{\{1,0\}\{1,0\}}\right)^2+$$
$$16\left(49\,D^4-605\,D^3+2578\,D^2-4380\,D+2304\right)\mathbf{J}^{(D)}_{\{1,0\}\{1,0\}\{1,0\}}\Big)\bigg)\Big/\left(24\,(D-6)\,(D-4)^2\,(D-1)\,p^2\right)\Bigg)$$

$$(4\pi)^D\,\Sigma_{12}(p) = -\frac{i\left(D^2-5\,D+6\right)e^4\,Q_2\,(p\cdot u)^2\left((D-4)\,D\,p^2\left(\mathbf{B}^{(D)}_{\{1,0\}\{1,0\}}\right)^2-4\left(5\,D^2-22\,D+16\right)\mathbf{J}^{(D)}_{\{1,0\}\{1,0\}\{1,0\}}\right)}{4\,(D-4)^2\,(D-1)\,p^2}$$

$$(4\pi)^D\,\Sigma_{13}(p) = -\Bigg(\bigg(i\,e^4\,Q_1\,(p\cdot u)^2\Big(3\,D\left(D^4-22\,D^3+164\,D^2-488\,D+480\right)p^2\left(\mathbf{B}^{(D)}_{\{1,0\}\{1,0\}}\right)^2+$$
$$16\left(49\,D^4-605\,D^3+2578\,D^2-4380\,D+2304\right)\mathbf{J}^{(D)}_{\{1,0\}\{1,0\}\{1,0\}}\Big)\bigg)\Big/\left(24\,(D-6)\,(D-4)^2\,(D-1)\,p^2\right)\Bigg)$$

$$(4\pi)^D\,\Sigma_{14}(p) = -\frac{i\left(D^2-5\,D+6\right)e^4\,Q_2\,(p\cdot u)^2\left((D-4)\,D\,p^2\left(\mathbf{B}^{(D)}_{\{1,0\}\{1,0\}}\right)^2-4\left(5\,D^2-22\,D+16\right)\mathbf{J}^{(D)}_{\{1,0\}\{1,0\}\{1,0\}}\right)}{4\,(D-4)^2\,(D-1)\,p^2}$$

$$(4\pi)^D\,\Sigma_{15}(p) = \frac{2\,i\left(2\,D^4-25\,D^3+111\,D^2-180\,D+96\right)e^4\,Q_1\,(p\cdot u)^2\,\mathbf{J}^{(D)}_{\{1,0\}\{1,0\}\{1,0\}}}{3\,(D-8)\,(D-6)\,(D-4)\,(D-1)\,p^2}$$

$$(4\pi)^D\,\Sigma_{16}(p) = \frac{2\,i\left(2\,D^4 - 25\,D^3 + 111\,D^2 - 180\,D + 96\right) e^4\,Q_1\,(\,p\cdot u\,)^2\,\mathbf{J}^{(D)}_{\{1,0\}\{1,0\}\{1,0\}}}{3\,(D-8)\,(D-6)\,(D-4)\,(D-1)\,p^2}$$

$$(4\pi)^D\,\Sigma_{17}(p) = \frac{8\,i\left(2\,D^4 - 27\,D^3 + 125\,D^2 - 222\,D + 108\right) e^4\,Q_1\,(\,p\cdot u\,)^2\,\mathbf{J}^{(D)}_{\{1,0\}\{1,0\}\{1,0\}}}{3\,(D-6)\,(D-4)\,(D-1)\,p^2}$$

$$(4\pi)^D\,\Sigma_{18}(p) = \frac{8\,i\left(2\,D^3 - 19\,D^2 + 57\,D - 54\right) e^4\,Q_2\,(\,p\cdot u\,)^2\,\mathbf{J}^{(D)}_{\{1,0\}\{1,0\}\{1,0\}}}{3\,(D-6)\,(D-4)\,p^2}$$

$$(4\pi)^D\,\Sigma_{20}(p) = -\frac{10\,i\,(D-3)\,e^4\,Q_1\,(\,p\cdot u\,)^2\,\mathbf{J}^{(D)}_{\{1,0\}\{1,0\}\{1,0\}}}{(D-4)\,p^2}$$

$$(4\pi)^D\,\Sigma_{24}(p) = -\frac{10\,i\,(D-3)\,e^4\,Q_1\,(\,p\cdot u\,)^2\,\mathbf{J}^{(D)}_{\{1,0\}\{1,0\}\{1,0\}}}{(D-4)\,p^2}$$

$$(4\pi)^D\,\Sigma_{27}(p) = \frac{i\,(D-3)\,\lambda^2\,Q_1\,(\,p\cdot u\,)^2\,\mathbf{J}^{(D)}_{\{1,0\}\{1,0\}\{1,0\}}}{3\,p^2}$$

$$(4\pi)^D\,\Sigma_{28}(p) = \frac{i\,(D-3)\,\lambda^2\,Q_1\,(\,p\cdot u\,)^2\,\mathbf{J}^{(D)}_{\{1,0\}\{1,0\}\{1,0\}}}{6\,p^2}$$

$$(4\pi)^D\,\Sigma_{29}(p) = \frac{2\,i\,(D-3)\,D\,e^4\,Q_1\,(\,p\cdot u\,)^2\,\mathbf{J}^{(D)}_{\{1,0\}\{1,0\}\{1,0\}}}{3\,p^2}$$

$$(4\pi)^D\,\Sigma_{30}(p) = -\frac{2\,i\left(D^2 - 5\,D + 6\right) e^4\,Q_2\,(\,p\cdot u\,)^2\,\mathbf{J}^{(D)}_{\{1,0\}\{1,0\}\{1,0\}}}{3\,p^2}$$

$$(4\pi)^D\,\Sigma_{32}(p) = -\frac{10\,i\,(D-3)\,e^4\,Q_1\,(\,p\cdot u\,)^2\,\mathbf{J}^{(D)}_{\{1,0\}\{1,0\}\{1,0\}}}{(D-4)\,p^2}$$

$$(4\pi)^D\,\Sigma_{34}(p) = -\frac{10\,i\,(D-3)\,e^4\,Q_1\,(\,p\cdot u\,)^2\,\mathbf{J}^{(D)}_{\{1,0\}\{1,0\}\{1,0\}}}{(D-4)\,p^2}$$

$$(4\pi)^D\,\Sigma_{47}(p) = -\frac{10\,i\,(D-3)\,e^4\,Q_1\,(\,p\cdot u\,)^2\,\mathbf{J}^{(D)}_{\{1,0\}\{1,0\}\{1,0\}}}{(D-4)\,p^2}$$

$$(4\pi)^D\,\Sigma_{48}(p) = -\frac{10\,i\,(D-3)\,e^4\,Q_1\,(\,p\cdot u\,)^2\,\mathbf{J}^{(D)}_{\{1,0\}\{1,0\}\{1,0\}}}{(D-4)\,p^2}$$

$$(4\pi)^D\,\Sigma_{55}(p) = -\frac{3\,i\left(3\,D^2 - 16\,D + 12\right) e^4\,Q_1\,(\,p\cdot u\,)^2\left(\mathbf{B}^{(D)}_{\{1,0\}\{1,0\}}\right)^2}{8\,(D-1)}$$

$$(4\pi)^D\,\Sigma_{56}(p) = -\frac{3}{4}\,i\,(D-2)\,e^4\,Q_2\,(\,p\cdot u\,)^2\left(\mathbf{B}^{(D)}_{\{1,0\}\{1,0\}}\right)^2$$

$$(4\pi)^D\,\Sigma_{63}(p) = -\frac{3\,i\left(3\,D^2 - 16\,D + 12\right) e^4\,Q_1\,(\,p\cdot u\,)^2\left(\mathbf{B}^{(D)}_{\{1,0\}\{1,0\}}\right)^2}{8\,(D-1)}$$

$$(4\pi)^D\,\Sigma_{64}(p) = -\frac{3}{4}\,i\,(D-2)\,e^4\,Q_2\,(\,p\cdot u\,)^2\left(\mathbf{B}^{(D)}_{\{1,0\}\{1,0\}}\right)^2$$

$$(4\,\pi)^D\,\Sigma_{66}(p) = -\frac{3\,i\left(D^2-5\,D+6\right)e^4\,Q_2\,(\,p\cdot u\,)^2\,\mathbf{J}^{(D)}_{\{1,0\}\,\{1,0\}\,\{1,0\}}}{(D-4)\,p^2}$$

$$(4\,\pi)^D\,\Sigma_{68}(p) = \frac{12\,i\left(D^2-8\,D+15\right)e^4\,Q_1\,(\,p\cdot u\,)^2\,\mathbf{J}^{(D)}_{\{1,0\}\,\{1,0\}\,\{1,0\}}}{(D-6)\,(D-4)\,p^2}$$

$$(4\,\pi)^D\,\Sigma_{69}(p) = \frac{4\,i\left(18\,D^3-151\,D^2+363\,D-216\right)e^4\,Q_1\,(\,p\cdot u\,)^2\,\mathbf{J}^{(D)}_{\{1,0\}\,\{1,0\}\,\{1,0\}}}{3\,(D-6)\,(D-4)\,(D-1)\,p^2}$$

$$(4\,\pi)^D\,\Sigma_{70}(p) = \frac{8\,i\left(D^2-3\,D+3\right)e^4\,Q_1\,(\,p\cdot u\,)^2\,\mathbf{J}^{(D)}_{\{1,0\}\,\{1,0\}\,\{1,0\}}}{3\,(D-6)\,(D-4)\,(D-1)\,p^2}$$

$$(4\,\pi)^D\,\Sigma_{71}(p) = \frac{4\,i\left(18\,D^3-151\,D^2+363\,D-216\right)e^4\,Q_1\,(\,p\cdot u\,)^2\,\mathbf{J}^{(D)}_{\{1,0\}\,\{1,0\}\,\{1,0\}}}{3\,(D-6)\,(D-4)\,(D-1)\,p^2}$$

$$(4\,\pi)^D\,\Sigma_{72}(p) = \frac{8\,i\left(D^2-3\,D+3\right)e^4\,Q_1\,(\,p\cdot u\,)^2\,\mathbf{J}^{(D)}_{\{1,0\}\,\{1,0\}\,\{1,0\}}}{3\,(D-6)\,(D-4)\,(D-1)\,p^2}$$

$$(4\,\pi)^D\,\Sigma_{73}(p) = \frac{8\,i\left(D^2-3\,D+3\right)e^4\,Q_1\,(\,p\cdot u\,)^2\,\mathbf{J}^{(D)}_{\{1,0\}\,\{1,0\}\,\{1,0\}}}{3\,(D-6)\,(D-4)\,(D-1)\,p^2}$$

$$(4\,\pi)^D\,\Sigma_{74}(p) = \frac{2\,i\,(25\,D-72)\,e^4\,Q_1\,(\,p\cdot u\,)^2\,\mathbf{J}^{(D)}_{\{1,0\}\,\{1,0\}\,\{1,0\}}}{3\,(D-4)\,p^2}$$

$$(4\,\pi)^D\,\Sigma_{75}(p) =$$
$$-\frac{i\,e^4\,Q_1\,(\,p\cdot u\,)^2\left(3\,D\left(3\,D^2-20\,D+32\right)p^2\left(\mathbf{B}^{(D)}_{\{1,0\}\,\{1,0\}}\right)^2+4\left(-75\,D^3+565\,D^2-1276\,D+768\right)\mathbf{J}^{(D)}_{\{1,0\}\,\{1,0\}\,\{1,0\}}\right)}{12\,(D-4)^2\,(D-1)\,p^2}$$

$$(4\,\pi)^D\,\Sigma_{77}(p) = \frac{12\,i\left(D^2-8\,D+15\right)e^4\,Q_1\,(\,p\cdot u\,)^2\,\mathbf{J}^{(D)}_{\{1,0\}\,\{1,0\}\,\{1,0\}}}{(D-6)\,(D-4)\,p^2}$$

$$(4\,\pi)^D\,\Sigma_{79}(p) = -\frac{3\,i\left(D^2-5\,D+6\right)e^4\,Q_2\,(\,p\cdot u\,)^2\,\mathbf{J}^{(D)}_{\{1,0\}\,\{1,0\}\,\{1,0\}}}{(D-4)\,p^2}$$

$$(4\,\pi)^D\,\Sigma_{86}(p) = \frac{8\,i\left(D^2-3\,D+3\right)e^4\,Q_1\,(\,p\cdot u\,)^2\,\mathbf{J}^{(D)}_{\{1,0\}\,\{1,0\}\,\{1,0\}}}{3\,(D-6)\,(D-4)\,(D-1)\,p^2}$$

$$(4\,\pi)^D\,\Sigma_{87}(p) = \frac{2\,i\,(25\,D-72)\,e^4\,Q_1\,(\,p\cdot u\,)^2\,\mathbf{J}^{(D)}_{\{1,0\}\,\{1,0\}\,\{1,0\}}}{3\,(D-4)\,p^2}$$

$$(4\,\pi)^D\,\Sigma_{88}(p) =$$
$$-\frac{i\,e^4\,Q_1\,(\,p\cdot u\,)^2\left(3\,D\left(3\,D^2-20\,D+32\right)p^2\left(\mathbf{B}^{(D)}_{\{1,0\}\,\{1,0\}}\right)^2+4\left(-75\,D^3+565\,D^2-1276\,D+768\right)\mathbf{J}^{(D)}_{\{1,0\}\,\{1,0\}\,\{1,0\}}\right)}{12\,(D-4)^2\,(D-1)\,p^2}$$

$$(4\,\pi)^D\,\Sigma_{89}(p) = \frac{1}{6\,(D-6)\,(D-4)^2\,(D-1)\,p^2}\,i\,e^4\,Q_1\,(\,p\cdot u\,)^2$$
$$\left(2\left(25\,D^5-400\,D^4+2497\,D^3-7462\,D^2+10\,224\,D-4608\right)\mathbf{J}^{(D)}_{\{1,0\}\,\{1,0\}\,\{1,0\}}-3\,D\left(D^2-10\,D+24\right)p^2\left(\mathbf{B}^{(D)}_{\{1,0\}\,\{1,0\}}\right)^2\right)$$

$$(4\,\pi)^D\,\Sigma_{90}(p) = \frac{4\,i\left(D^3-5\,D^2+6\,D-6\right)\mathrm{e}^4\,Q_1\,(\,p\cdot u\,)^2\,\mathbf{J}^{(D)}_{\{1,0\}\{1,0\}\{1,0\}}}{3\,(D-6)\,(D-4)\,(D-1)\,p^2}$$

$$(4\,\pi)^D\,\Sigma_{91}(p) = \frac{4\,i\left(D^2-5\,D+6\right)\mathrm{e}^4\,Q_2\,(\,p\cdot u\,)^2\,\mathbf{J}^{(D)}_{\{1,0\}\{1,0\}\{1,0\}}}{(D-4)\,p^2}$$

$$(4\,\pi)^D\,\Sigma_{92}(p) = -\frac{32\,i\left(2\,D^2-15\,D+27\right)\mathrm{e}^4\,Q_1\,(\,p\cdot u\,)^2\,\mathbf{J}^{(D)}_{\{1,0\}\{1,0\}\{1,0\}}}{3\,(D-6)\,(D-4)\,p^2}$$

$$(4\,\pi)^D\,\Sigma_{93}(p) = \frac{2\,i\,(D-2)^2\,\mathrm{e}^4\,Q_2\,(\,p\cdot u\,)^2\,\mathbf{J}^{(D)}_{\{1,0\}\{1,0\}\{1,0\}}}{(D-6)\,(D-4)\,(D-1)\,p^2}$$

$$(4\,\pi)^D\,\Sigma_{94}(p) = -\frac{32\,i\left(2\,D^2-15\,D+27\right)\mathrm{e}^4\,Q_1\,(\,p\cdot u\,)^2\,\mathbf{J}^{(D)}_{\{1,0\}\{1,0\}\{1,0\}}}{3\,(D-6)\,(D-4)\,p^2}$$

$$(4\,\pi)^D\,\Sigma_{95}(p) = \frac{2\,i\,(D-2)^2\,\mathrm{e}^4\,Q_2\,(\,p\cdot u\,)^2\,\mathbf{J}^{(D)}_{\{1,0\}\{1,0\}\{1,0\}}}{(D-6)\,(D-4)\,(D-1)\,p^2}$$

$$(4\,\pi)^D\,\Sigma_{99}(p) = -\frac{9}{2}\,i\,\mathrm{e}^4\,Q_1\,(\,p\cdot u\,)^2\left(\mathbf{B}^{(D)}_{\{1,0\}\{1,0\}}\right)^2$$

$$(4\,\pi)^D\,\Sigma_{100}(p) = -\frac{9}{2}\,i\,\mathrm{e}^4\,Q_1\,(\,p\cdot u\,)^2\left(\mathbf{B}^{(D)}_{\{1,0\}\{1,0\}}\right)^2$$

$$(4\,\pi)^D\,\Sigma_{104}(p) = -\frac{9}{2}\,i\,\mathrm{e}^4\,Q_1\,(\,p\cdot u\,)^2\left(\mathbf{B}^{(D)}_{\{1,0\}\{1,0\}}\right)^2$$

Expanding the integrals for $D = 4 - 2\epsilon$ and adding all contributions, we finally find

$$\begin{aligned} -i\Sigma_{2l-LV} \;=\; & \frac{(p\cdot u)^2}{18432\pi^4\epsilon^2}\Big\{60e^4(11Q_1+4Q_2) - \epsilon\Big[120e^4\log\left(-p^2\right)(11Q_1+4Q_2) \\ & -9\lambda^2 Q_1 + 8e^4\Big(11Q_1(15\gamma_E - 26 - 30\log(2) - 15\log(\pi)) \\ & +2Q_2(30\gamma_E - 43 - 60\log(2) - 30\log(\pi))\Big)\Big]\Big\}. \end{aligned} \tag{5}$$

## III. FINAL REMARKS

In conclusion, this supplemental material has presented a detailed calculation of the two-loop self-energy amplitudes for the photon and the scalar field in CPT-even Lorentz-violating scalar electrodynamics. By considering the Feynman diagrams and applying techniques such as tensor integral decomposition and the Tarasov algorithm, we obtained explicit expressions for the amplitudes. The computation involved the evaluation of various integrals, including one-loop and two-loop integrals, which were either well-known or calculated in previous studies. Overall, the detailed analysis presented in this supplemental material enhances our knowledge of the two-loop self-energy amplitudes in CPT-even Lorentz-violating scalar electrodynamics, furthering our understanding of the underlying physics and laying the groundwork for future studies in this field.

In addition to the two-loop self-energy amplitudes, our study also includes the computation of the three-point functions in CPT-even Lorentz-violating scalar electrodynamics. These three-point functions involve a large number of diagrams, exceeding seven hundred in total. Due to the complexity and extensive nature of these diagrams, we have chosen not to present the detailed calculations in this supplemental material.

### Appendix A: Definition o the integrals

The basic integrals used in this text and employed by the TARCER package, as defined in Ref. [5], are

$$\mathbf{A}^{(D)}_{\{1,0\}} = \frac{1}{\pi^{D/2}} \int \frac{d^D k}{k^2} = 0; \tag{A1}$$

$$\mathbf{B}^{(D)}_{\{1,0\},\{1,0\}} = \frac{1}{\pi^{D/2}} \int \frac{d^D k}{k^2 (k-p)^2} = \frac{i}{\epsilon} - i \left(\log(-p^2) + \gamma_E - 2\right) + \mathcal{O}(\epsilon); \tag{A2}$$

$$\mathbf{J}^{(D)}_{\{1,0\},\{1,0\},\{1,0\}} = \frac{1}{\pi^D} \int \frac{d^D k_1 \, d^D k_2}{k_1^2 (k_1-k_2)^2 (k_2-p)^2} = \frac{p^2}{2} \left(\frac{1}{2\epsilon} - \log(-p^2) - \gamma_E + \frac{13}{4}\right) + \mathcal{O}(\epsilon), \tag{A3}$$

where $\gamma_E$ is the Euler-Mascheroni constant and $D = 4 - 2\epsilon$. The one-loop integrals are well-known and have been extensively studied in the literature. A comprehensive calculation of the two-loop integral was carried out in Ref. [7].

[1] R. Mertig, M. Bohm and A. Denner, Comput. Phys. Commun. **64**, 345-359 (1991) doi:10.1016/0010-4655(91)90130-D; V. Shtabovenko, R. Mertig and F. Orellana, Comput. Phys. Commun. **207**,

432-444 (2016) doi:10.1016/j.cpc.2016.06.008 [arXiv:1601.01167 [hep-ph]]; V. Shtabovenko, R. Mertig and F. Orellana, Comput. Phys. Commun. **256**, 107478 (2020). doi:10.1016/j.cpc.2020.107478 [arXiv:2001.04407 [hep-ph]];

[2] T. Hahn, Comput. Phys. Commun. **140**, 418-431 (2001) doi:10.1016/S0010-4655(01)00290-9 [arXiv:hep-ph/0012260 [hep-ph]].

[3] A. Alloul, N. D. Christensen, C. Degrande, C. Duhr, and B. Fuks, Comput. Phys. Commun. **185**, 2250 (2014).

[4] V. Shtabovenko, Comput. Phys. Commun. **218**, 48-65 (2017) doi:10.1016/j.cpc.2017.04.014 [arXiv:1611.06793 [physics.comp-ph]].

[5] R. Mertig and R. Scharf, Comput. Phys. Commun. **111**, 265-273 (1998) doi:10.1016/S0010-4655(98)00042-3 [arXiv:hep-ph/9801383 [hep-ph]].

[6] O. V. Tarasov, Nucl. Phys. B **502**, 455-482 (1997) doi:10.1016/S0550-3213(97)00376-3 [arXiv:hep-ph/9703319 [hep-ph]].

[7] S. P. Martin and D. G. Robertson, Comput. Phys. Commun. **174**, 133-151 (2006) doi:10.1016/j.cpc.2005.08.005 [arXiv:hep-ph/0501132 [hep-ph]].

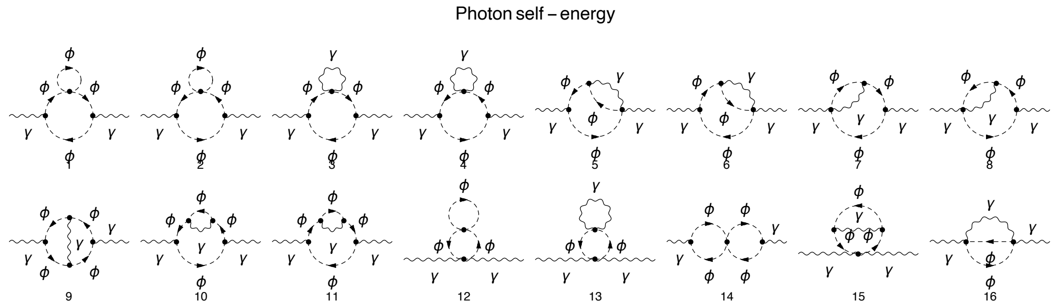


Figure 1: Feynman diagrams for the two-loop photon self-energy. Dashed and wavy lines represent the scalar and photon propagators, respectively.

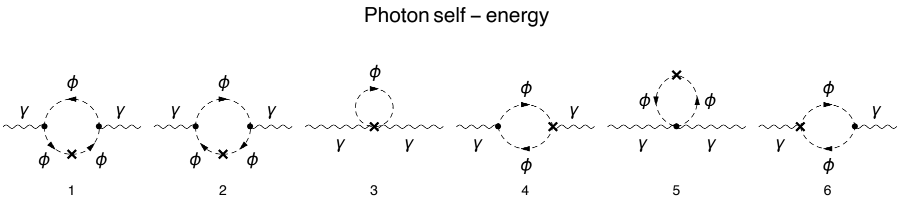


Figure 2: Contribution of order $e^4$ to the photon self-energy. The crossed vertices represent the insertion of an one-loop counterterm.

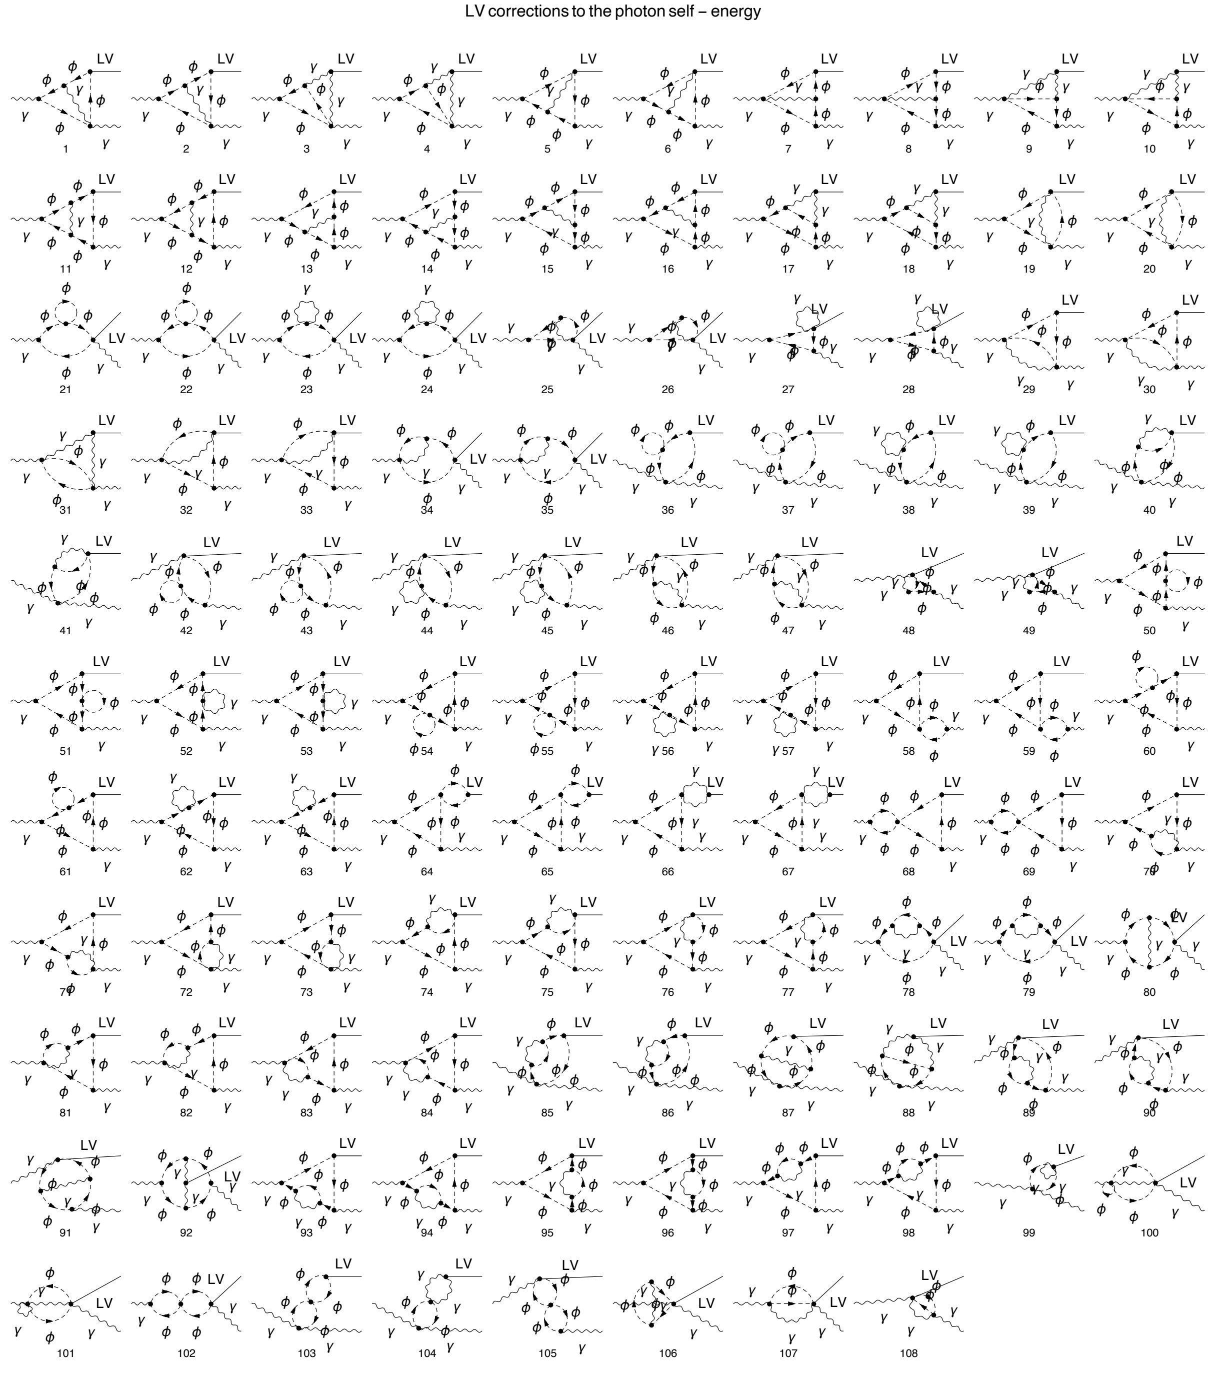


Figure 3: Feynman diagrams for the LV corrections to the two-loop photon self-energy. The straight line represents the insertion of a LV vertex.

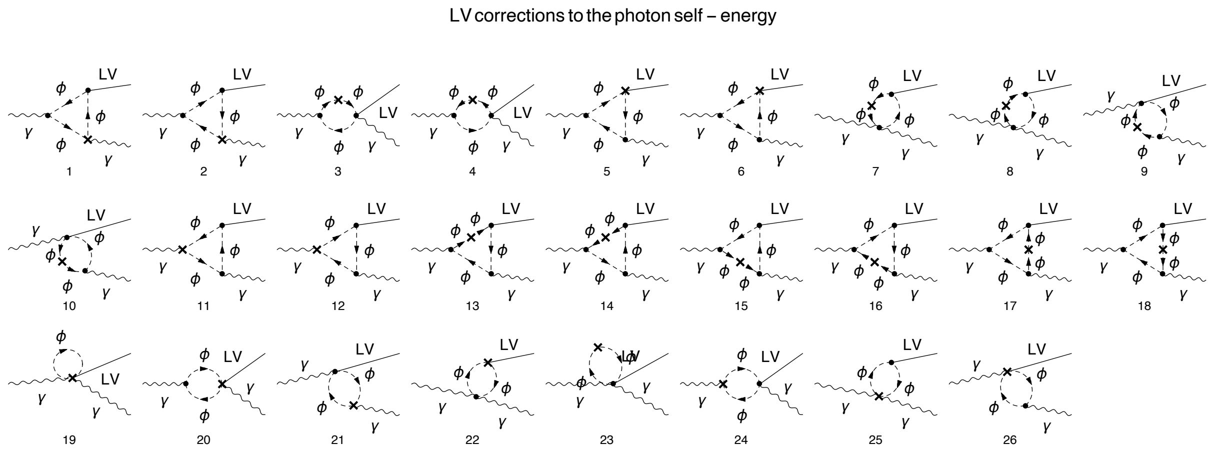


Figure 4: One-loop counterterm insertions in the LV corrections of order $e^4$ to the photon self-energy.

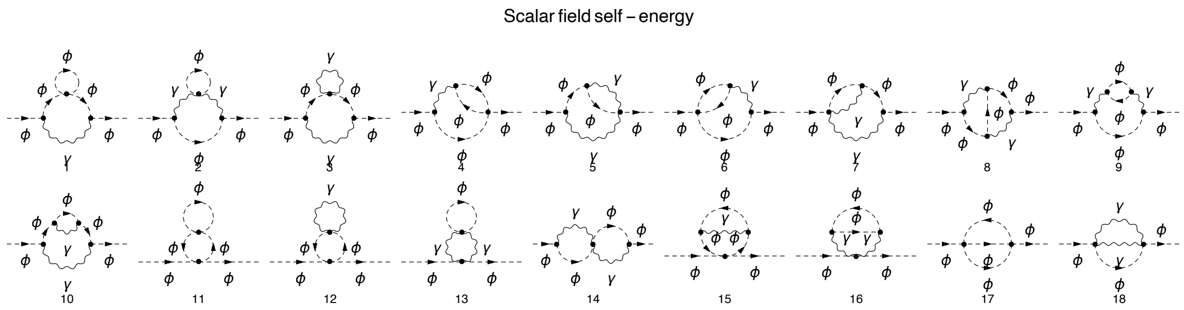


Figure 5: Scalar field self-energy.

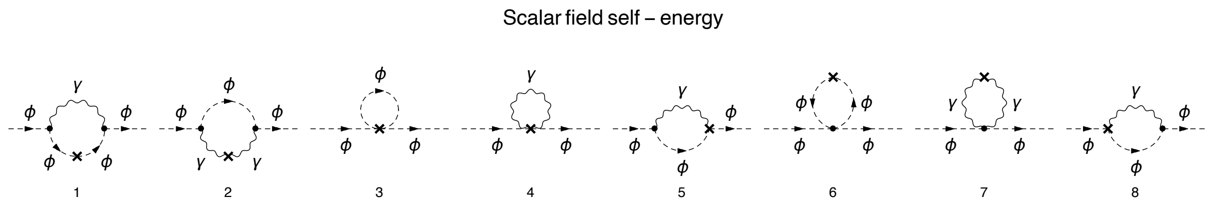


Figure 6: Scalar field self-energy.

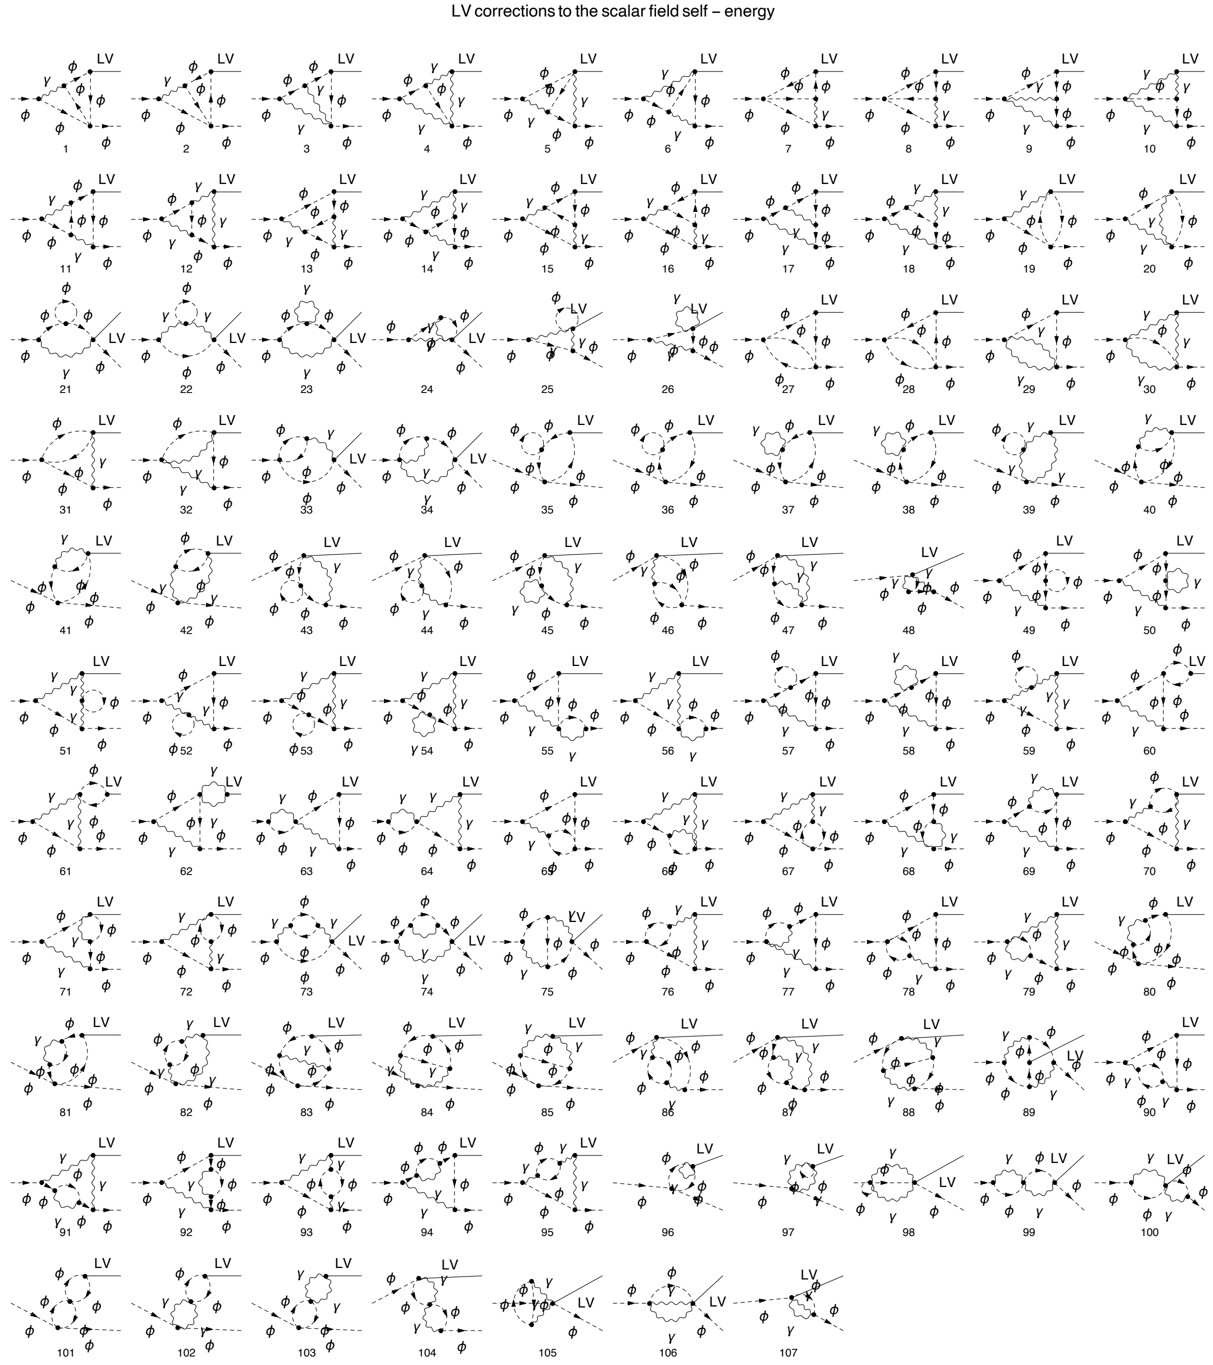


Figure 7: LV corrections to the scalar field self-energy.

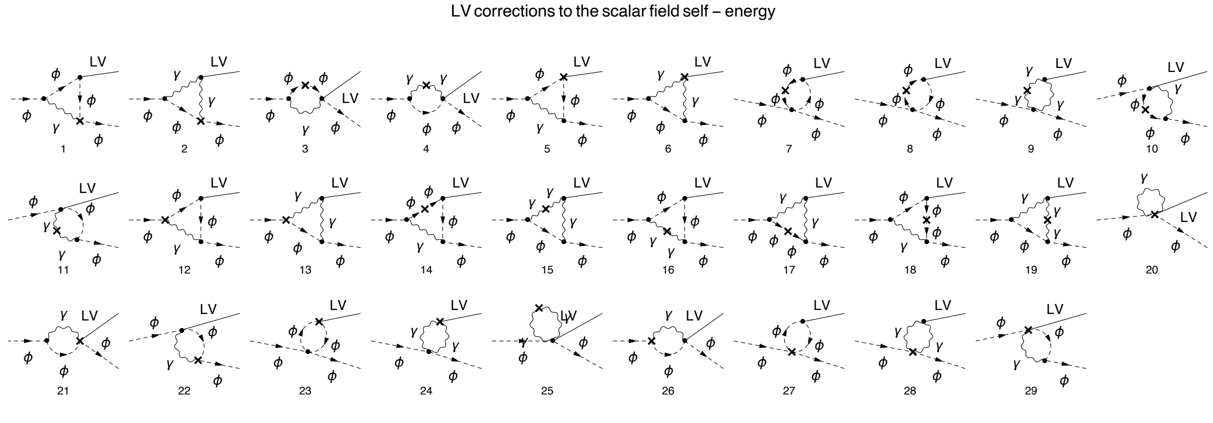


Figure 8: One-loop counterterm insertions in the LV corrections to the scalar field self-energy.
